# Supplementary material for: Spatiotemporal modelling of sea duck abundance: implications for marine spatial planning
Source: arXiv:1705.00644 source file (2017-05-01)
Supplement: Supplementary file 2 [file Appendix_S2.pdf]

# Appendix S2. Covariate details

We evaluated biophysical covariates (Table S2.1) expected to influence the distribution, abundance, and movements of sea ducks or, more likely, the distribution and availability of their benthic prey (e.g., mollusks and crustaceans); we did not have information related directly to the distribution of preferred prey. Biophysical covariates could be characterized as spatial (varying only among segments), temporal (varying within or among winters, but not among segments) or as spatiotemporal effects (varying among segments and within or among winters). We allowed the effect of bathymetry and relative sea surface temperature to vary over time within a given winter via interactions with day of season. We also included a survey effort covariate and covariates that were solely a function of segment geographic location, which we used to address potential spatial correlation in the data. We standardized (i.e., mean centered and scaled) all continuous covariates. Appendix S3 describes and illustrates the use of an R function to visualize the spatial and temporal distribution of these covariates in Nantucket Sound.

**Table S2.1** Biophysical and survey covariates used to evaluate the distribution and abundance of Common Eider, Black, Surf, and White-winged Scoter, and Long-tailed Duck in Nantucket Sound during winters 2003 - 2005.

| Variable (abbreviation) | Units | Variable type[1] | Description |
|---|---|---|---|
| Day of year (*time*) | day | T | seasonality; number of days from 31 December; negative values indicate days prior to 31 December |
| Bathymetry (*depth*) | m | S | bottom depth relative to mean high water; National Oceanic and Atmospheric Administration's (NOAA) National Geographic Data Center (NGDC): http://ngdc.noaa.gov/dem/squareCellGrid/download/385 (Eakins et al. 2009) |
| Sediment grain size (*meanphi*) | phi | S | sediment grain size (phi scale; Poti et al. 2012) |
| Sea floor surface area relative to planimetric area (*SAR*) | N/A | S | ratio of sea floor surface area (calculated from bathymetry; Jenness 2004) to planimetric area; estimate of the topographic variability of the sea floor |
| Epibenthic tidal velocity (mean; *tidebmean*) | m/s | S | average epibenthic tidal velocity during 2003-2005 based on monthly Finite-Volume Community Ocean Model (FVCOM) data (structured grids from http://fvcom.smast.umassd.edu/Data/FVCOM/NECOFS/Archive/; Chen et al. 2003, 2011) |
| Epibenthic tidal velocity (standard deviation; *tidesd*) | m/s | S | standard deviation of epibenthic tidal velocity during 2003-2005 base based on monthly FVCOM structured grids (Chen et al. 2003, 2011) |

| Variable (abbreviation) | Units | Variable type[1] | Description |
|---|---|---|---|
| Water column stratification potential (*strat*) | $s^3/m^2$ | S | potential for seasonal thermal stratification of the water column (Simpson and Hunter 1974), calculated as the ratio of depth ($h$; from bathymetry) to the third power of surface tidal velocity ($u$; from monthly FVCOM structured grids; Chen et al. 2003, 2011); we report $\log_{10}(h/u^3)$ for each segment. Higher values indicate areas more prone to thermal stratification during the summer. Although the numerical value of $\log_{10}(h/u^3)$ at which stratification occurs depends on the choice of $u$, relative values among locations remain consistent (Simpson and Sharples 2012) |
| Chlorophyll-a (*chla*) | $mg/m^3$ | S | geometric mean of monthly composite chlorophyll-a levels from July 2002 (first available) to March 2006; data from the Aqua MODIS satellite via NOAA Environmental Research Division's Data Access Program (ERDDAP): http://coastwatch.pfeg.noaa.gov/erddap/info/erdMEchlamday/index.html |
| Chromophoric dissolved organic material (*cdom*) | N/A | S | geometric mean of monthly composite chromophoric dissolved organic material levels (measured based on absorbance values) from July 2002 (first available) to March 2006; data from the Aqua MODIS satellite via NOAA ERDDAP: http://coastwatch.pfeg.noaa.gov/erddap/info/erdMEcdommday/index.html. No units (absorbancy measure). Note the experimental nature of this product. |

| Variable (abbreviation) | Units | Variable type[1] | Description |
|---|---|---|---|
| Sea bottom temperature ($SBT$) | °C | ST | sea bottom (epibenthic) temperature averaged from May to October for each year (2003-2005) from monthly FVCOM structured grids (Chen et al. 2003, 2011). May through October corresponds to the period of settling of relevant bivalve spawn in the area (Evans et al. 2011), and temperature potentially influences mussel settling and growth (Fay et al. 1983, Newell 1989) |
| Sea surface temperature (monthly; $SST_m$) | °C | ST | monthly sea surface temperature from monthly FVCOM structured grid (Chen et al. 2003, 2011); available alternative sea surface temperature sources possessed too coarse resolution (e.g., AHVRR Pathfinder; Zipkin et al. 2010) or inconsistent measurements in the study area (e.g., Aqua MODIS; Winiarski et al. 2013) |
| Sea surface temperature (Nov - Mar; $SST_w$) | °C | ST | average winter (November through March) sea surface temperature from monthly FVCOM structured grids (Chen et al. 2003, 2011) |
| Sea surface temperature (relative; $SST_{rel}$) | °C | ST | difference between the monthly sea surface temperature of a segment and the average sea surface temperature of the entire study area; based on monthly FVCOM structured grids (Chen et al. 2003, 2011) |

| Variable (abbreviation) | Units | Variable type[1] | Description |
|---|---|---|---|
| North Atlantic Oscillation (Dec - Mar; $NAO_w$) | N/A | T | winter (December through March) North Atlantic Oscillation index based on the principal component time series of the leading empirical orthogonal function of sea level pressure anomalies over the Atlantic sector (Hurrell 1995, Hurrell and Deser 2010); data from the Climate Analysis Section, National Center for Atmospheric Research: https://climatedataguide.ucar.edu/climate-data/hurrell-north-atlantic-oscillation-nao-index-pc-based (accessed 14 April 2014) |
| Distance to land (*d2land*) | km | S | distance to the nearest location of zero depth (from bathymetry) |
| Ferry route within 1 km (*ferry*) | N/A | S | indicator of whether the ferry route from Cape Cod to Nantucket (Massachusetts Department of Transportation, Office of Transportation Planning) intersects a given segment; the ferry route was buffered by 1 km to accommodate potential sea duck responses to ship traffic at a distance and uncertainty in ferry route (Larsen and Laubek 2005, De La Cruz et al. 2014). Ferries traversed this route approximately 16 times per day during the study period |
| Winter 2004 (*y2004*) | N/A | T | indicator comparing surveys occurring from November 2004 through April 2005 with those occurring from December 2003 through April 2004 |
| Winter 2005 (*y2005*) | N/A | T | indicator comparing surveys occurring from October 2005 through March 2006 with those occurring from December 2003 through April 2004 |

| Variable (abbreviation) | Units | Variable type[1] | Description |
| --- | --- | --- | --- |
| Easting (*xkm*) | km | S | distance between the easting of a segment center from the median easting of all segments surveyed in the study area; negative and positive values indicate segments west and east of the median easting, respectively |
| Northing (*ykm*) | km | S | distance between the northing of a segment center from the median northing of all segments surveyed in the study area; negative and positive values indicate segments south and north of the median northing, respectively |
| Survey effort (*obs_window*) | $km^2$ | ST | area of strip transect surveyed in a given segment on a given survey date; calculated as the product of the length and width of the strip transect |

[1]Variable type: S (spatial; varying only among segments); T (temporal; varying only over time); ST (spatiotemporal; varying in space and time)

## Literature cited


Chen, C., H. Huang, R. C. Beardsley, Q. Xu, R. Limeburner, G. W. Cowles, Y. Sun, J. Qi, and H. Lin. 2011. Tidal dynamics in the Gulf of Maine and New England Shelf: An application of FVCOM. Journal of Geophysical Research: Oceans 116:1–14.

Chen, C., H. Liu, and R. C. Beardsley. 2003. An unstructured grid, finite-volume, three-dimensional primitive equations ocean model: Application to coastal ocean and estuaries. Journal of Atmospheric and Oceanic Technology 20:159–186.

De La Cruz, S. E. W., J. M. Eadie, A. Keith Miles, J. Yee, K. A. Spragens, E. C. Palm, and J. Y. Takekawa. 2014. Resource selection and space use by sea ducks during the non-breeding season: Implications for habitat conservation planning in urbanized estuaries. Biological Conservation 169:68–78.

Eakins, B., L. Taylor, K. Carignan, R. Warnken, E. Lim, and P. Medley. 2009. Digital elevation model of Nantucket, Massachusetts: Procedures, data sources and analysis, NOAA Technical Memorandum NESDIS NGDC-26. Department of Commerce, Boulder, CO, USA.

Evans, N., K. Ford, B. Chase, and J. Sheppard. 2011. Recommended time of year restrictions (TOYs) for coastal alteration projects to protect marine fisheries resources in Massachusetts. Massachusetts Division of Marine Fisheries, New Bedford, MA, USA.

Fay, C. W., R. J. Neves, and G. B. Pardue. 1983. Species profiles: Life histories and environmental requirements of coastal fishes and invertebrates (Mid-Atlantic) – surf clam. U.S. Fish. Wildl. Serv. Biol. Rep. 82(11. 13). U.S. Army Corps of Engineers, TR El-82-4. 23 pp.

Hurrell, J. W. 1995. Decadal trends in the North Atlantic Oscillation: Regional temperatures and precipitation. Science 269:676–679.

Hurrell, J. W., and C. Deser. 2010. North Atlantic climate variability: The role of the North Atlantic Oscillation. Journal of Marine Systems 79:231–244.

Jenness, J. S. 2004. Calculating landscape surface area from digital elevation models. Wildlife Society Bulletin 32:829–839.

Larsen, J. K., and B. Laubek. 2005. Impacts of high-speed ferry disturbance on wintering sea ducks. Wildfowl 55:99–116.

Newell, R. I. 1989. Species profiles: Life histories and environmental requirements of coastal fishes and invertebrates (North and Mid-Atlantic)–blue mussel. U.S. Fish. Wildl. Serv. Biol. Rep. 82(11. 102). U.S. Army Corps of Engineers, TR El-82-4. 25 pp.

Poti, M., B. Kinlan, and C. Menza. 2012. Chapter 3: Surficial sediments. Pages 33–58 *in* C. Menza, B. Kinlan, D. Dorfman, M. Poti, and C. Caldow, editors. A biogeographic assessment of seabirds, deep sea corals and ocean habitats of the New York Bight: Sci-

ence to support offshore spatial planning. NOAA Technical Memorandum NOS NCCOS 141. Silver Spring, MD.

Simpson, J. H., and J. R. Hunter. 1974. Fronts in the Irish Sea. Nature 250:404–406.

Simpson, J. H., and J. Sharples. 2012. Introduction to the physical and biological oceanography of shelf seas. Cambridge University Press, New York, New York, USA.

Winiarski, K. J., D. L. Miller, P. W. C. Paton, and S. R. McWilliams. 2013. Spatially explicit model of wintering Common Loons: Conservation implications. Marine Ecology Progress Series 492:273–283.

Zipkin, E. F., B. Gardner, A. T. Gilbert, A. F. O. Jr, J. A. Royle, and E. D. Silverman. 2010. Distribution patterns of wintering sea ducks in relation to the North Atlantic Oscillation and local environmental characteristics. Oecologia 163:893–902.
