# Supplementary material for: Spatiotemporal modelling of sea duck abundance: implications for marine spatial planning
Source: arXiv:1705.00644 source file (2017-05-01)
Supplement: Supplementary file 3 [file Appendix_S3.pdf]

# Appendix S3. Visualizing covariate distribution

We illustrate the visualization of biophysical covariates used in the construction of sea duck distribution and abundance models in Nantucket Sound. A custom function (`plot_covariate`) plots, as applicable, the spatial distribution and temporal dynamics of these covariates in the study area.

The arguments of the `plot_covariate` function allow some flexibility in manipulating the plotted output:

```
## function (z = "depth", data = env.segs, x = "x", y = "y", plotwind = FALSE,
##     segs = TRUE, agg.seg = c(NA, "mean", "sum"), winter = "winter",
##     month = "date", legend.title = NULL, legend.size = 10, scale = FALSE,
##     diverge = FALSE)
## NULL
```

Only a few arguments are likely to be modified in the current context: `z` defines the covariate of interest, and can take any of the following values (see Appendix S2 for definitions): SSTw, SSTm, SSTrel, SBT, chla, cdom, meanphi, depth, d2land, SAR, tidebmean, tidesd, strat, NAOw, ferry, or length. `plotwind` and `segs` are logicals indicating whether the user would like to plot the permitted wind energy development area or segment boundaries (see Figure 1 in manuscript), respectively. `agg.seg` allows temporally dynamic (i.e., varying within a winter or among winters) covariate values to be summarized (e.g., average, sum) within each segment; the default is to plot their dynamics, and not summarize, within the study area. `legend.title` and `legend.size` permit the modification of the legend title and legend size, respectively. The `scale` option standardizes `z` prior to plotting, and the `diverge` option changes the legend of a continuous covariate to divergent colors on either side of zero, a useful modification for visualizing standardized covariates.

## Spatial covariates

The bathymetry of Nantucket Sound varied only in space, and can be visualized with the default options (Figure S3.1, left panel). More informatively, perhaps, the standardized depth values can be plotted with a legend scale diverging around zero, as well as a custom legend title and the wind development area indicating (Figure S3.1, right panel), using:

```r
plot_covariate("depth") # Figure S3.1, left
# Figure S3.1, right
plot_covariate("depth", legend.title = "Scaled\ndepth (m)",
               plotwind = TRUE, scale = TRUE, diverge = TRUE)
```

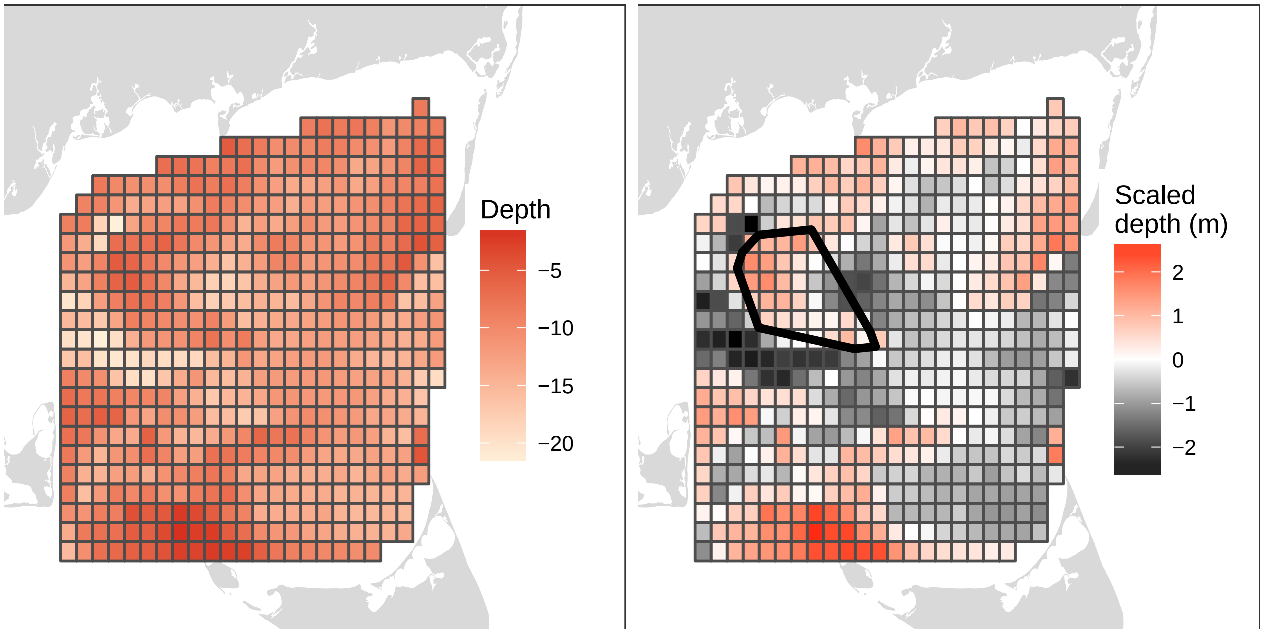


**Figure S3.1**. Nantucket Sound bathymetry (left) and standardized with a diverging legend scale, custom legend title, and delineated wind development area (right).

## Spatiotemporal covariates

Certain covariates varied spatially within Nantucket Sound but also monthly and/or annually; `plot_covariate` identifies these temporal changes and divides the plot accordingly. For example, the average sea surface temperature from November through March (SSTw) varied among segments in Nantucket Sound, as well as on an annual basis (Figure S3.2). Sea surface temperature relative to other segments in a given month (SSTrel) varied spatially, annually, and monthly (Figure S3.3).

```r
plot_covariate("SSTw", scale = TRUE, diverge = TRUE) # Figure S3.2
```

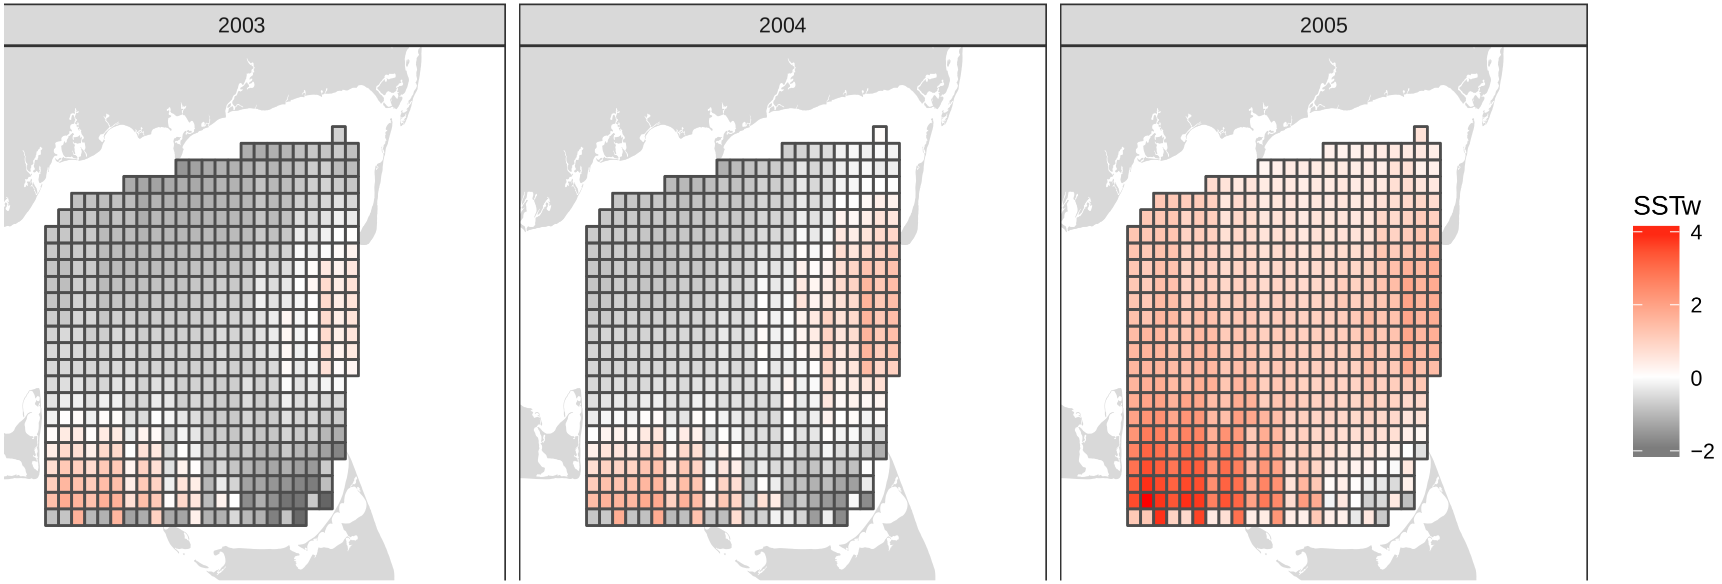


**Figure S3.2**. Spatial and annual variation in standardized sea surface temperature from Novemeber through March (SSTw) in Nantucket Sound.

```r
plot_covariate("SSTrel", segs = FALSE, scale = TRUE, diverge = TRUE) # Figure S3.3
```

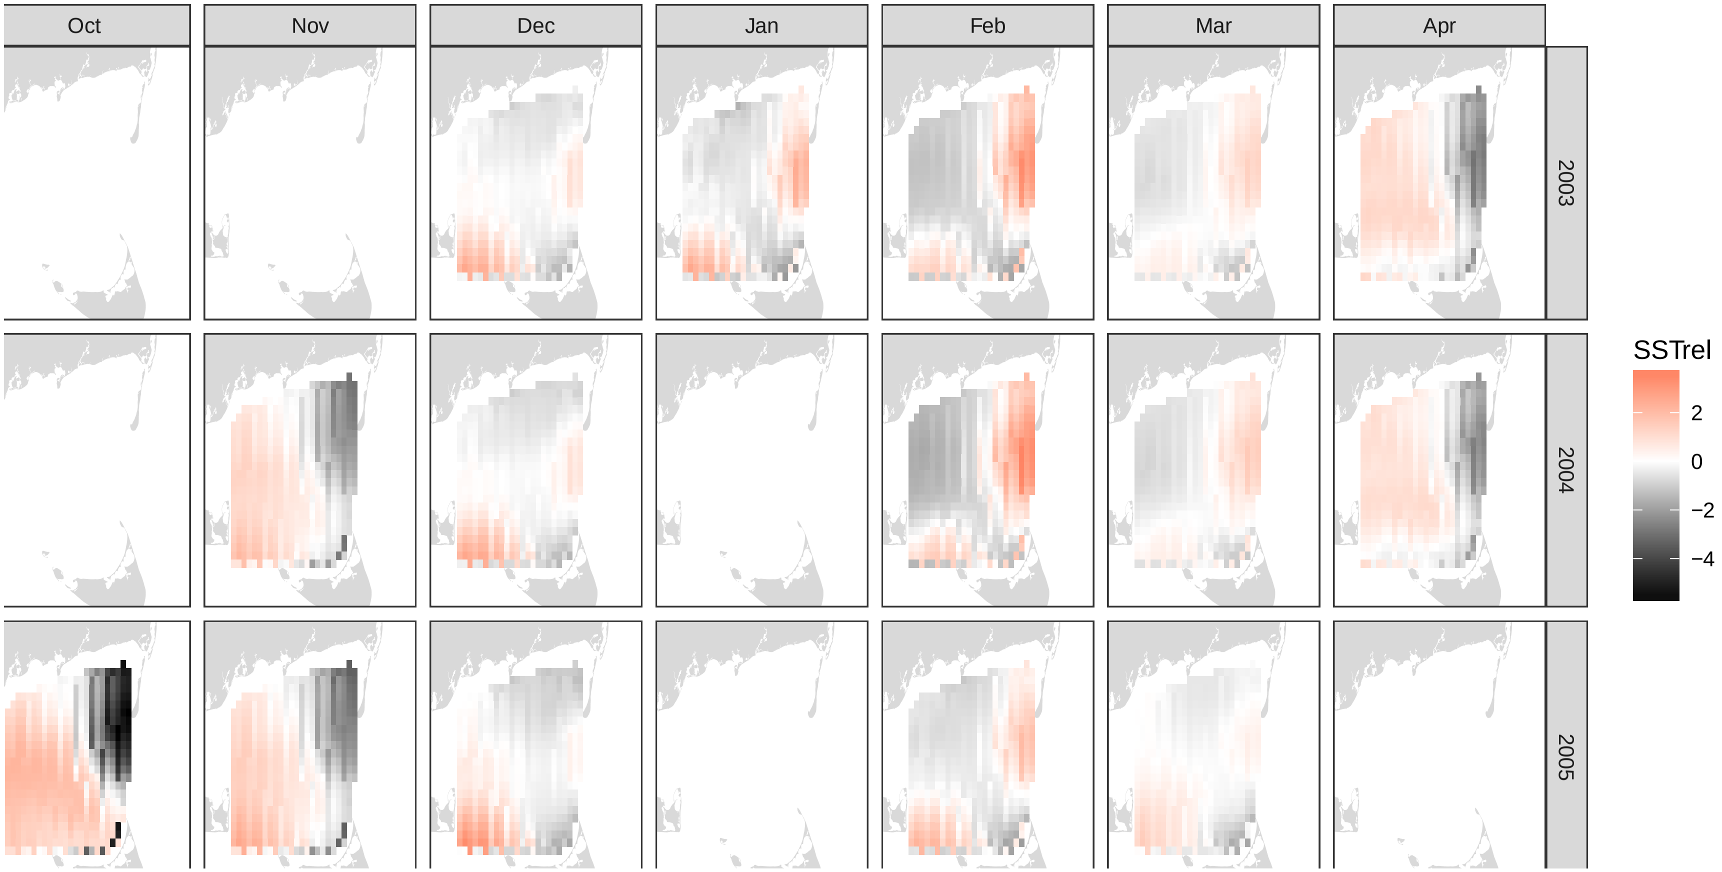


**Figure S3.3**. Spatial, monthly, and annual variation in standardized sea surface temperature relative to other segments (SSTrel) in Nantucket Sound. Empty panels indicate that data are not available for a particular year and month combination.

Lastly, it can be useful to aggregate temporally-dynamic covariate values within segments. For example, the total length of transect surveyed in each segment over the course of this study is obtained with:

```
plot_covariate("length", agg.seg = "sum",
               legend.title = "Survey effort\n(km transect)") # Figure S3.4
```

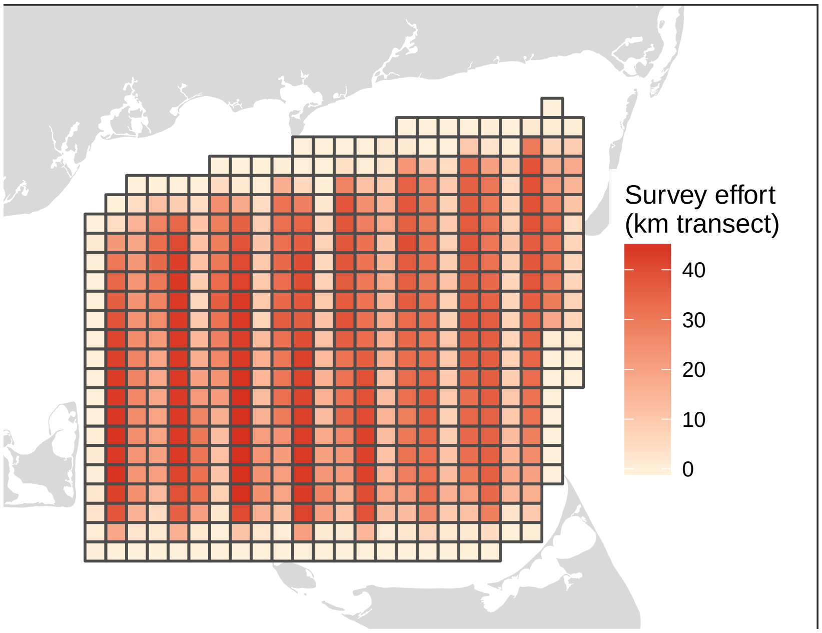


**Figure S3.4**. Total length (km) of strip transects surveyed in 504 2.25km$^2$ segments during 30 aerial sea duck surveys in Nantucket Sound.
