# Supplementary material for: Spatiotemporal modelling of sea duck abundance: implications for marine spatial planning
Source: arXiv:1705.00644 source file (2017-05-01)
Supplement: Supplementary file 4 [file Appendix_S4.pdf]

# Appendix S4. Early stopping

## Occupancy models

All occupancy models converged to the maximum likelihood estimates (i.e., did not stop early; Figure S4.1). Failure to stop early sometimes happens in data sets with many observations and strong effects (see comment of Kneib in Bühlmann *et al.* 2014). This suggests that the effects of the environmental variables on sea duck occupancy are rather complex.

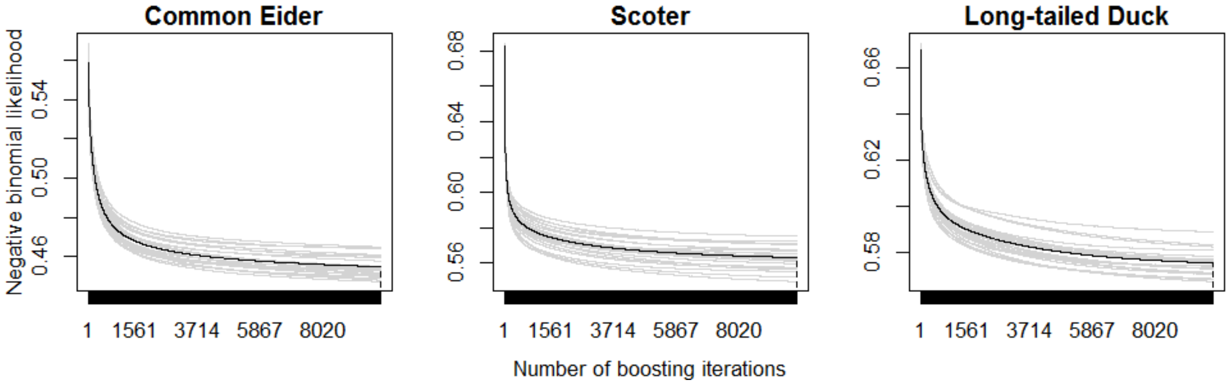


**Figure S4.1** Bootstrapped out-of-bag empirical risk in sea duck occupancy models based on 25-fold subsampling. Gray lines indicate the out-of-bag risk on each subsample and the black line indicates the average out-of-bag risk; the optimal iteration is indicated by the dashed vertical line.

## Count models

In contrast to occupancy model, bootstrapping prescribed early stopping for both parameters in all count models (Figure S4.2).

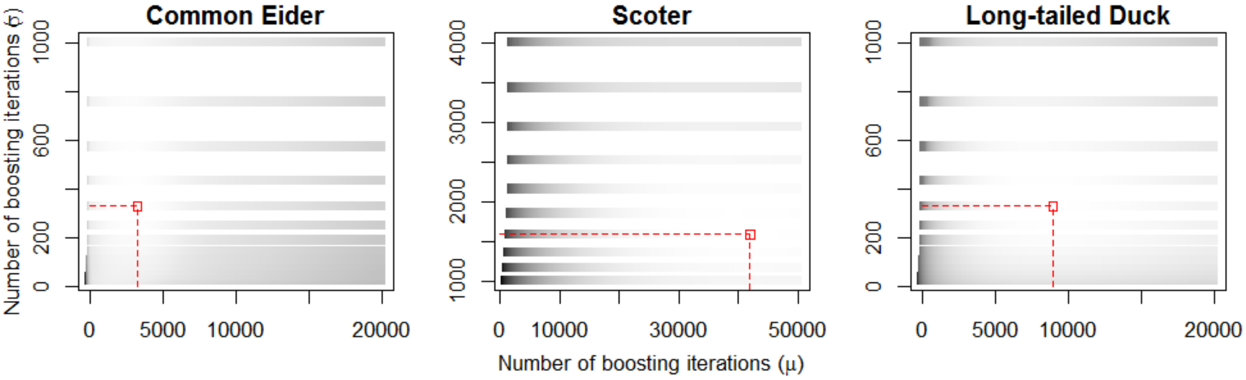


**Figure S4.2** Bootstrapped out-of-bag empirical risk in sea duck conditional count models based on 25-fold subsampling. Lighter colors indicate lower average out-of-bag risk (over the 25 samples) for a given combination of $m_{\text{stop}}$-values for $\mu$ and $\sigma$; the optimal combination is indicated by the red square.

## Literature Cited

Bühlmann, P., Gertheiss, J., Hieke, S., Kneib, T., Ma, S., Schumacher, M., Tutz, G., Wang, C.-Y., Wang, Z. & Ziegler, A. (2014). Discussion of 'the evolution of boosting algorithms' and 'extending statistical boosting'. *Methods of Information in Medicine*, **53**, 436–445.
