# Supplementary material for: Spatiotemporal modelling of sea duck abundance: implications for marine spatial planning
Source: arXiv:1705.00644 source file (2017-05-01)
Supplement: Supplementary file 5 [file Appendix_S6.pdf]

# Appendix S6. Scoter stable covariate effects

Marginal functional plots of the relationships between covariates (controlling for all other variables; i.e., at their mean values) and the occupancy, conditional mean abundance, and conditional overdispersion of abundance of scoters (Black, Surf, and White-winged Scoter) in Nantucket Sound, Massachusetts, USA. Covariate plots are ordered roughly in descending order of the magnitude of their influence on the additive predictor in each model (or model parameter for count models). Vertical lines along the $x$-axis (i.e., rug plots) indicate observed covariate values. Covariates (and any abbreviations) are defined in detail in Appendix S2; only effects selected to be stable (see Appendix S1) are depicted.

# Occupancy

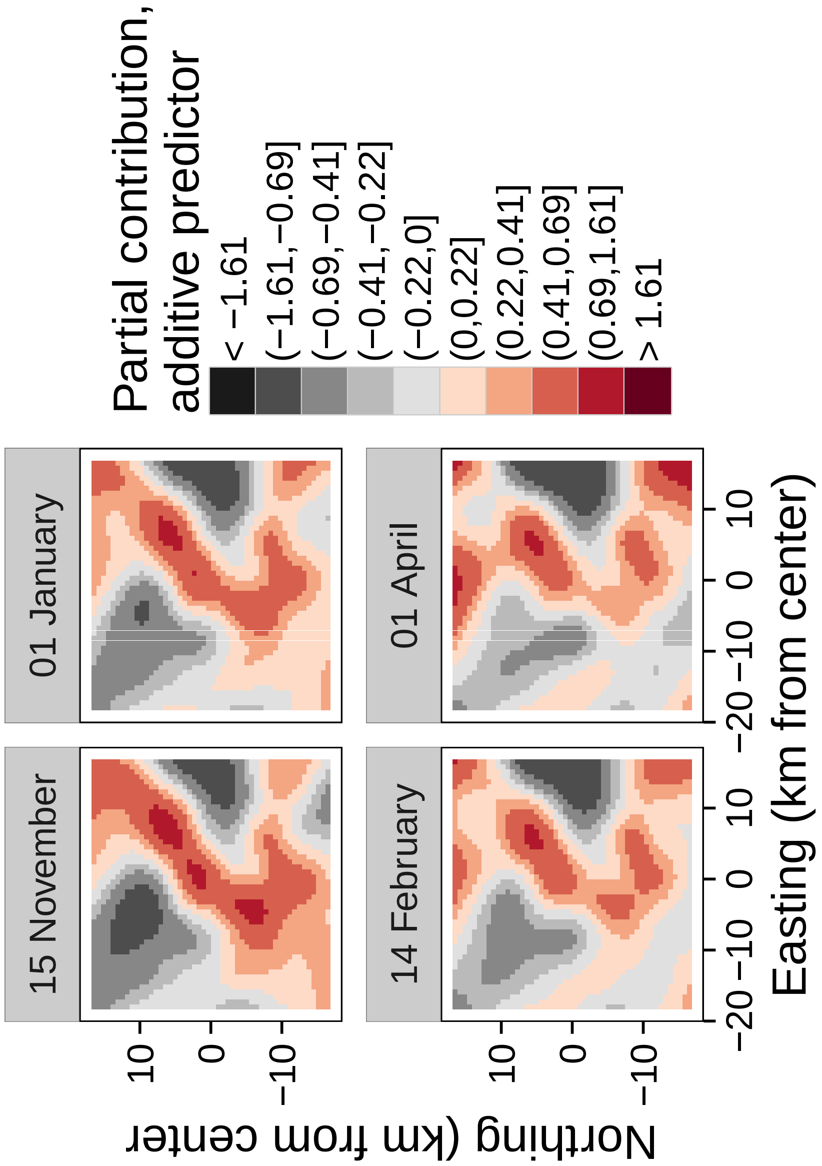

Partial contribution, additive predictor
< −1.61
(−1.61,−0.69]
(−0.69,−0.41]
(−0.41,−0.22]
(−0.22,0]
(0,0.22]
(0.22,0.41]
(0.41,0.69]
(0.69,1.61]
> 1.61
15 November
01 January
14 February
01 April
Northing (km from center)
Easting (km from center)
10
0
−10
−20

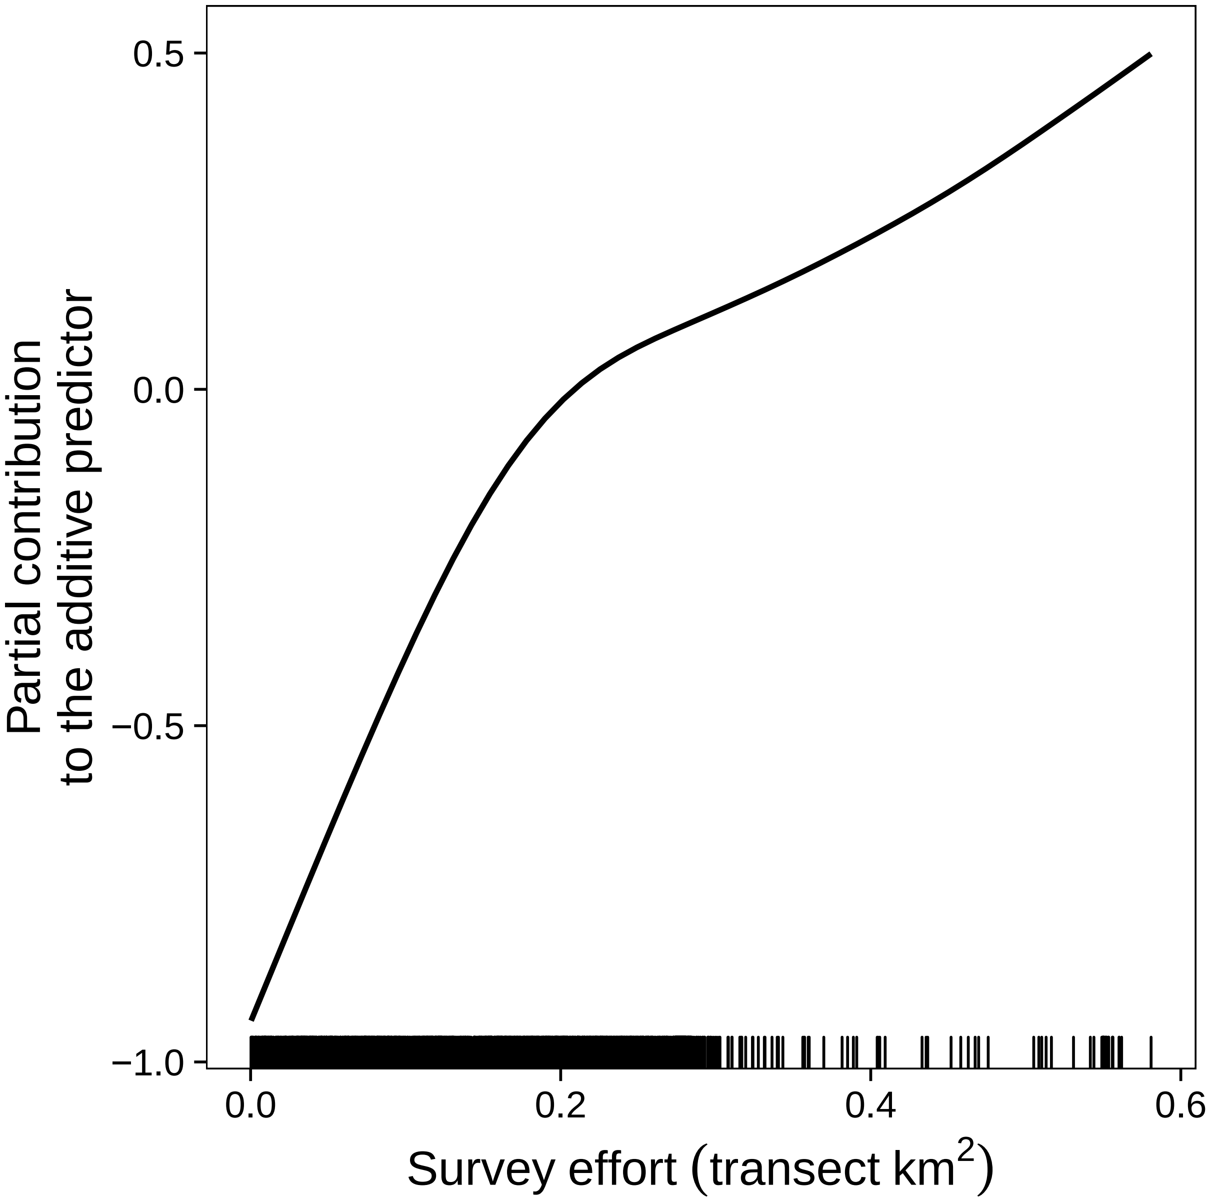
Partial contribution
to the additive predictor
0.5
0.0
−0.5
−1.0
0.0
0.2
0.4
0.6
Survey effort (transect km2)

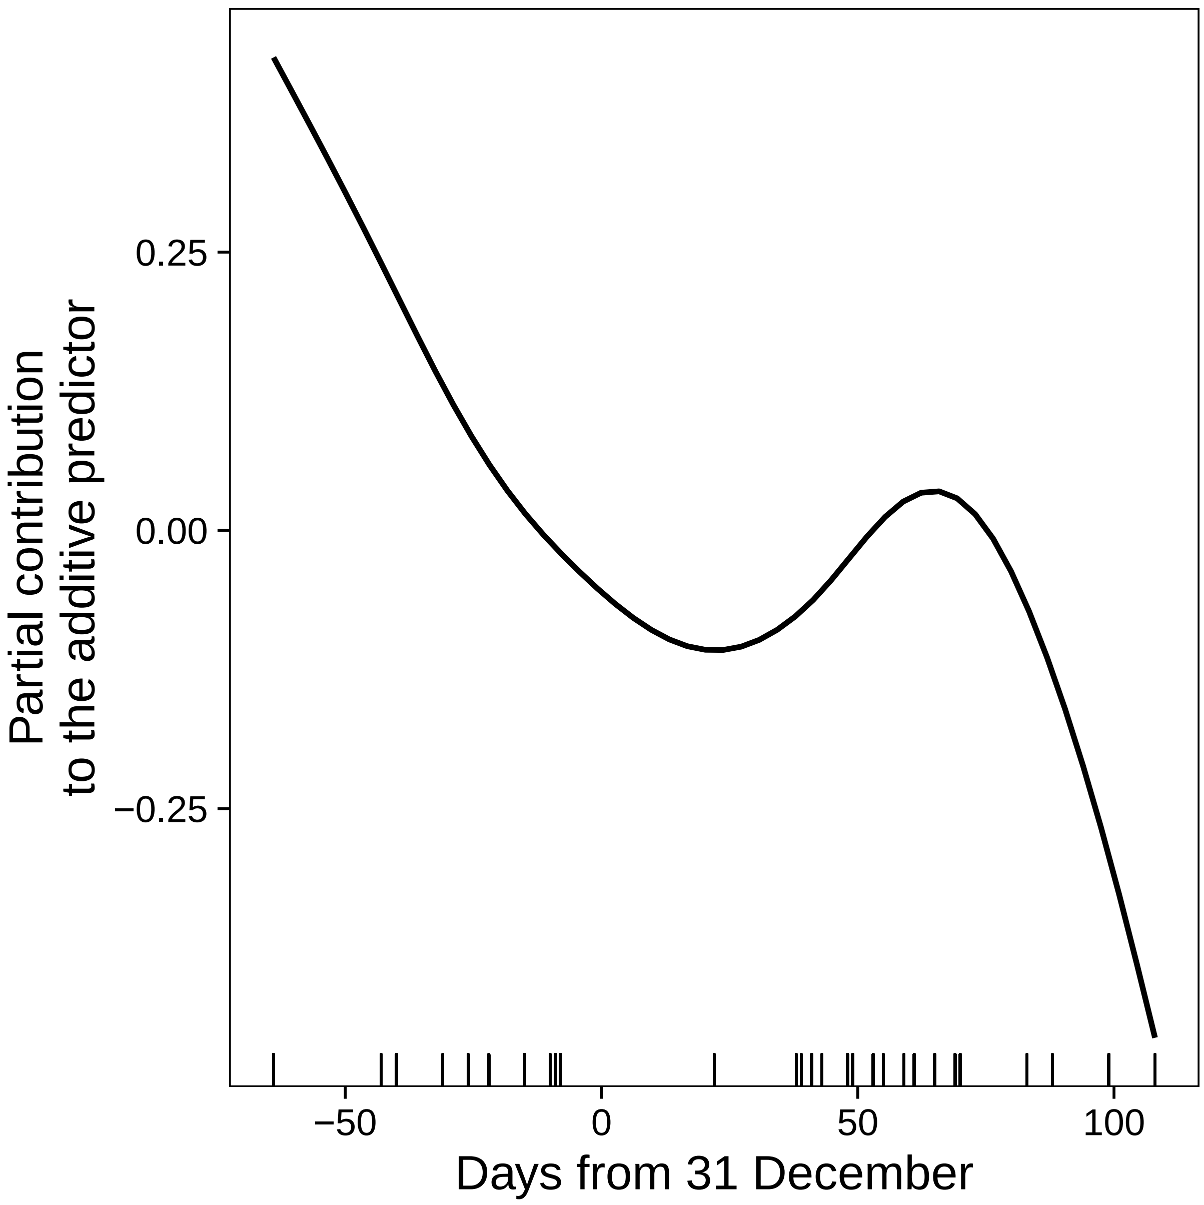
Partial contribution
to the additive predictor
0.25
0.00
−0.25
−50
0
50
100
Days from 31 December

13

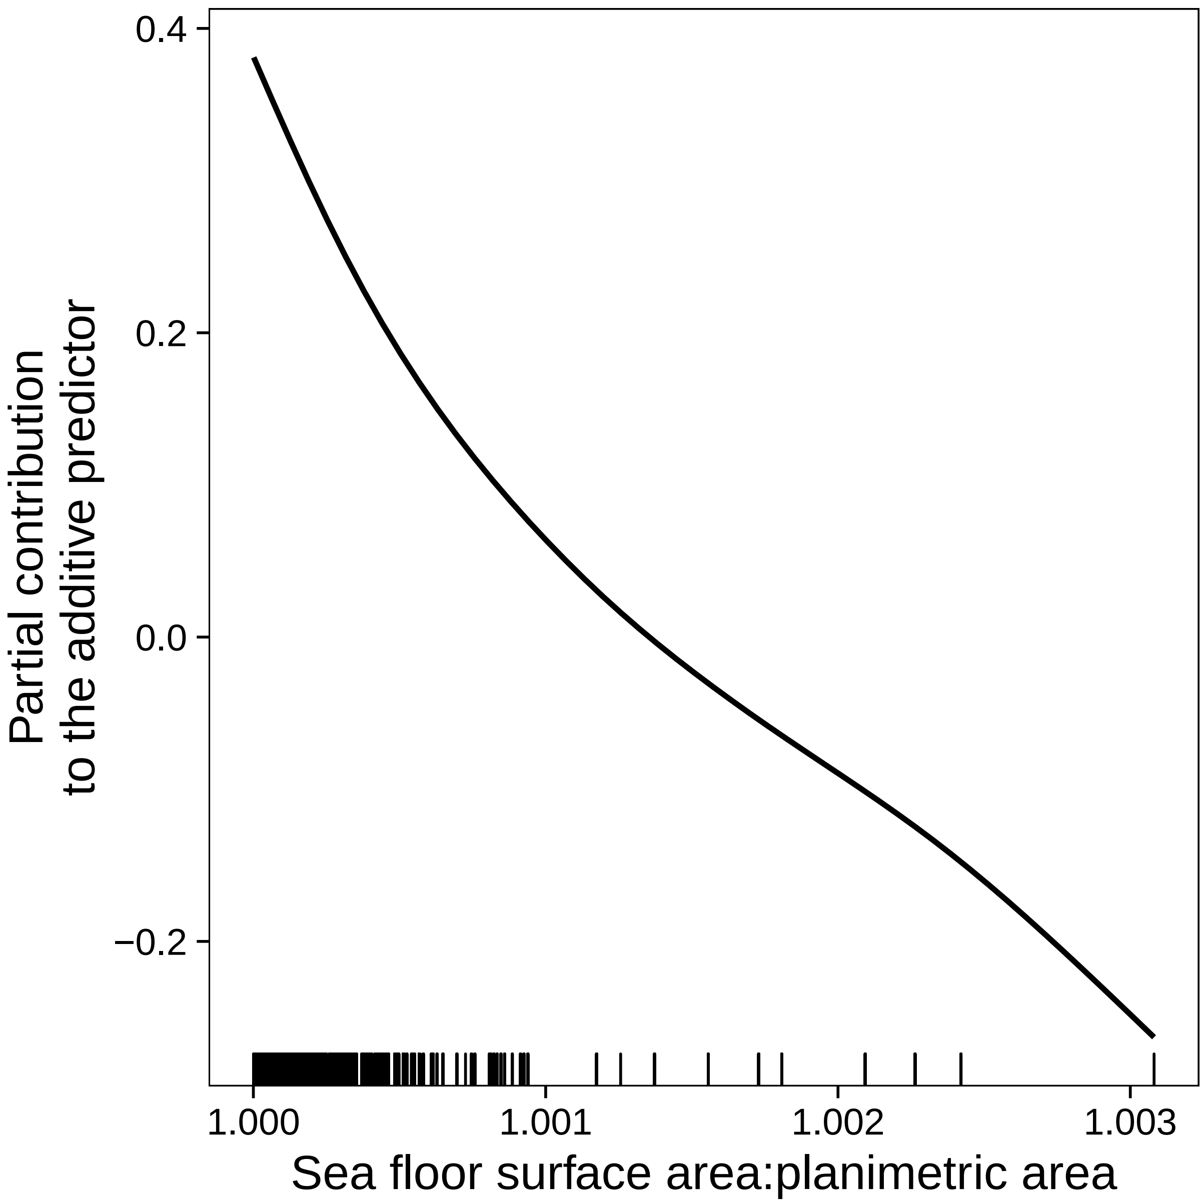
Partial contribution
to the additive predictor
0.4
0.2
0.0
−0.2
1.000
1.001
1.002
1.003
Sea floor surface area:planimetric area

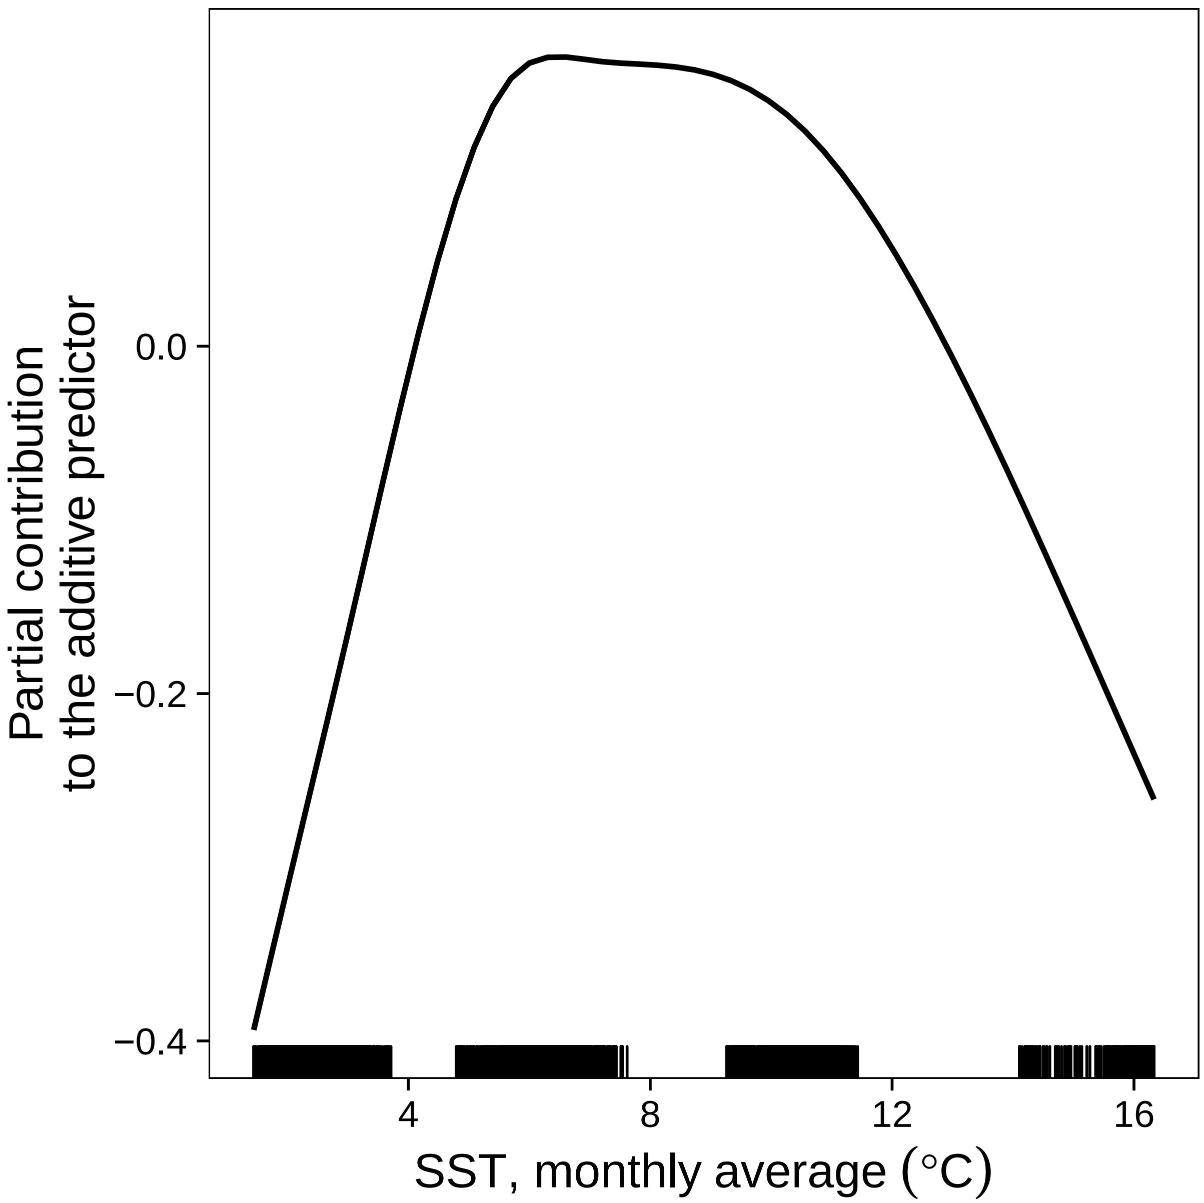
Partial contribution
to the additive predictor
0.0
−0.2
−0.4
4
8
12
16
SST, monthly average (°C)

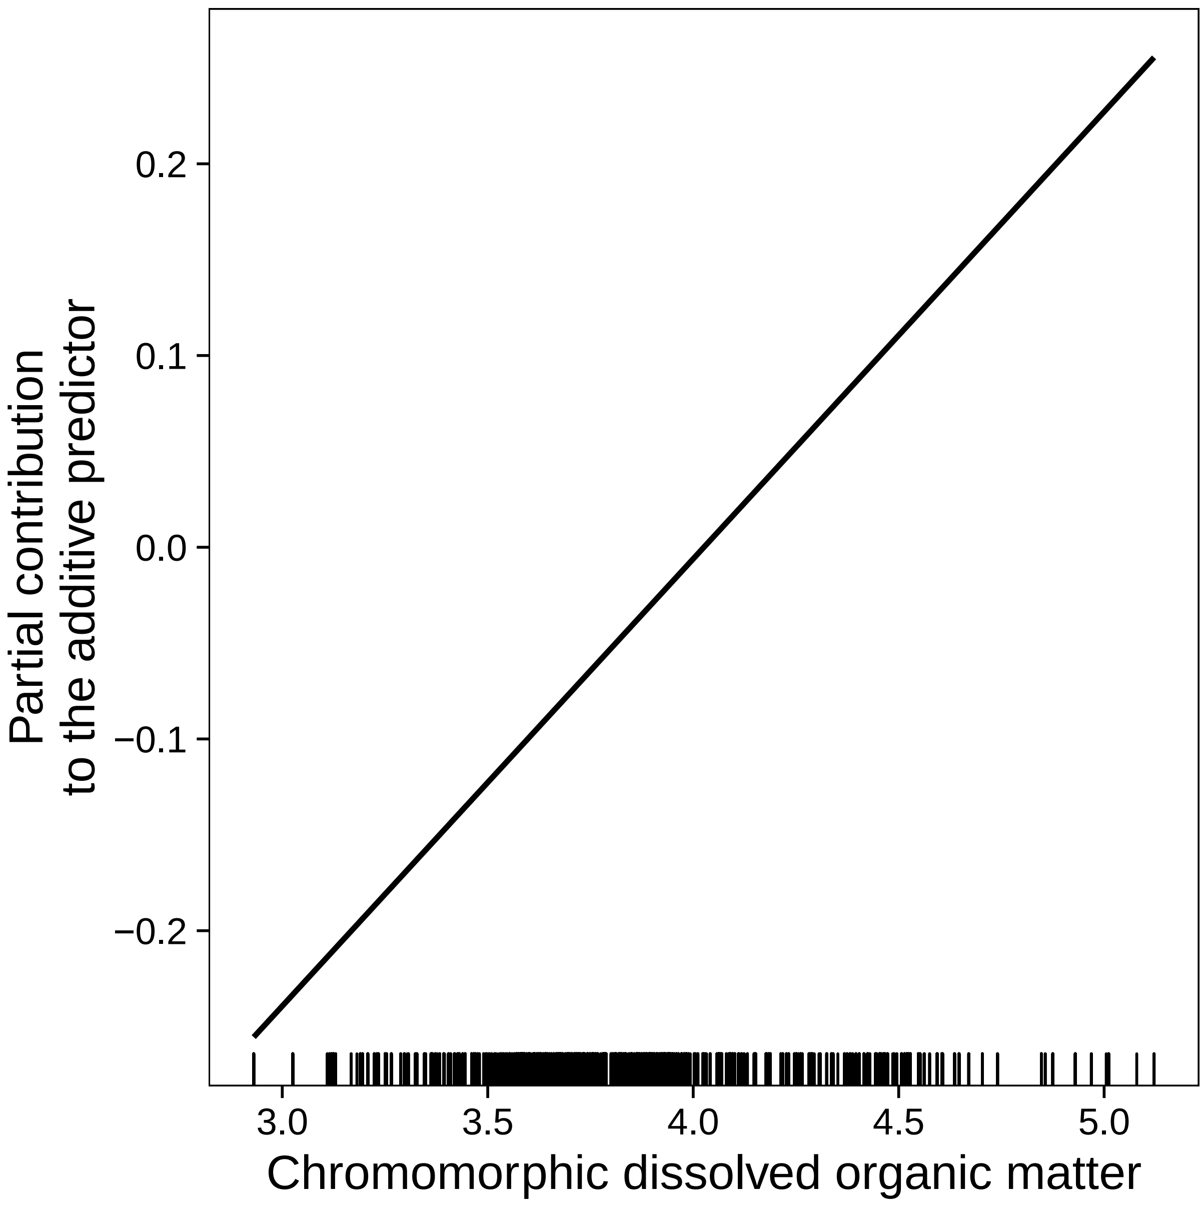
Partial contribution
to the additive predictor
0.2
0.1
0.0
−0.1
−0.2
3.0
3.5
4.0
4.5
5.0
Chromomorphic dissolved organic matter

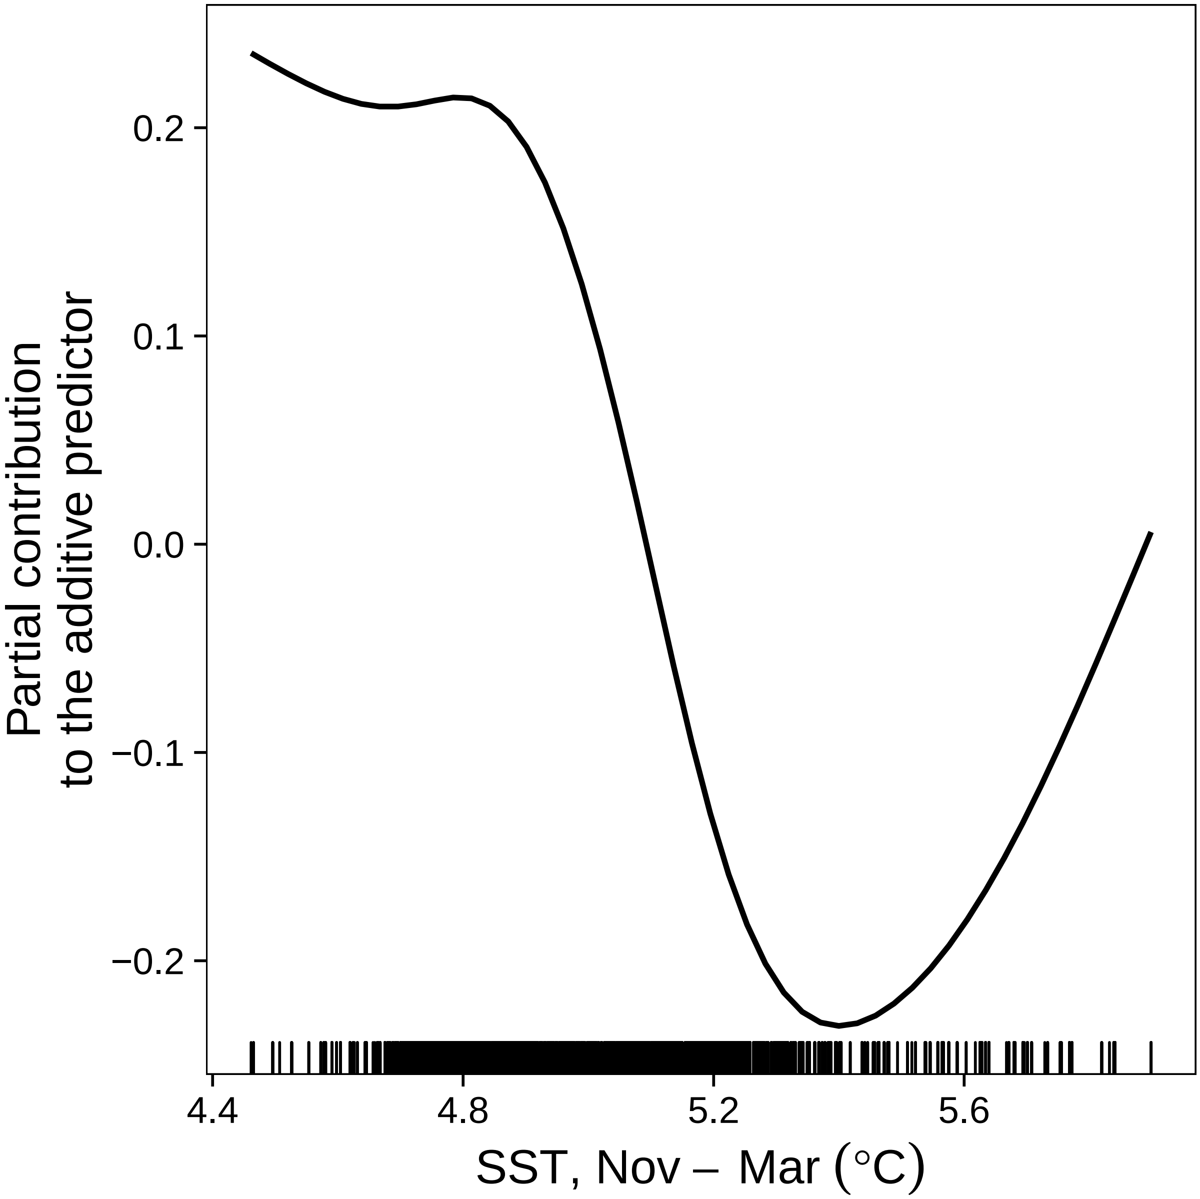

Partial contribution
to the additive predictor
0.2
0.1
0.0
−0.1
−0.2
4.4
4.8
5.2
5.6
SST, Nov – Mar (°C)


17

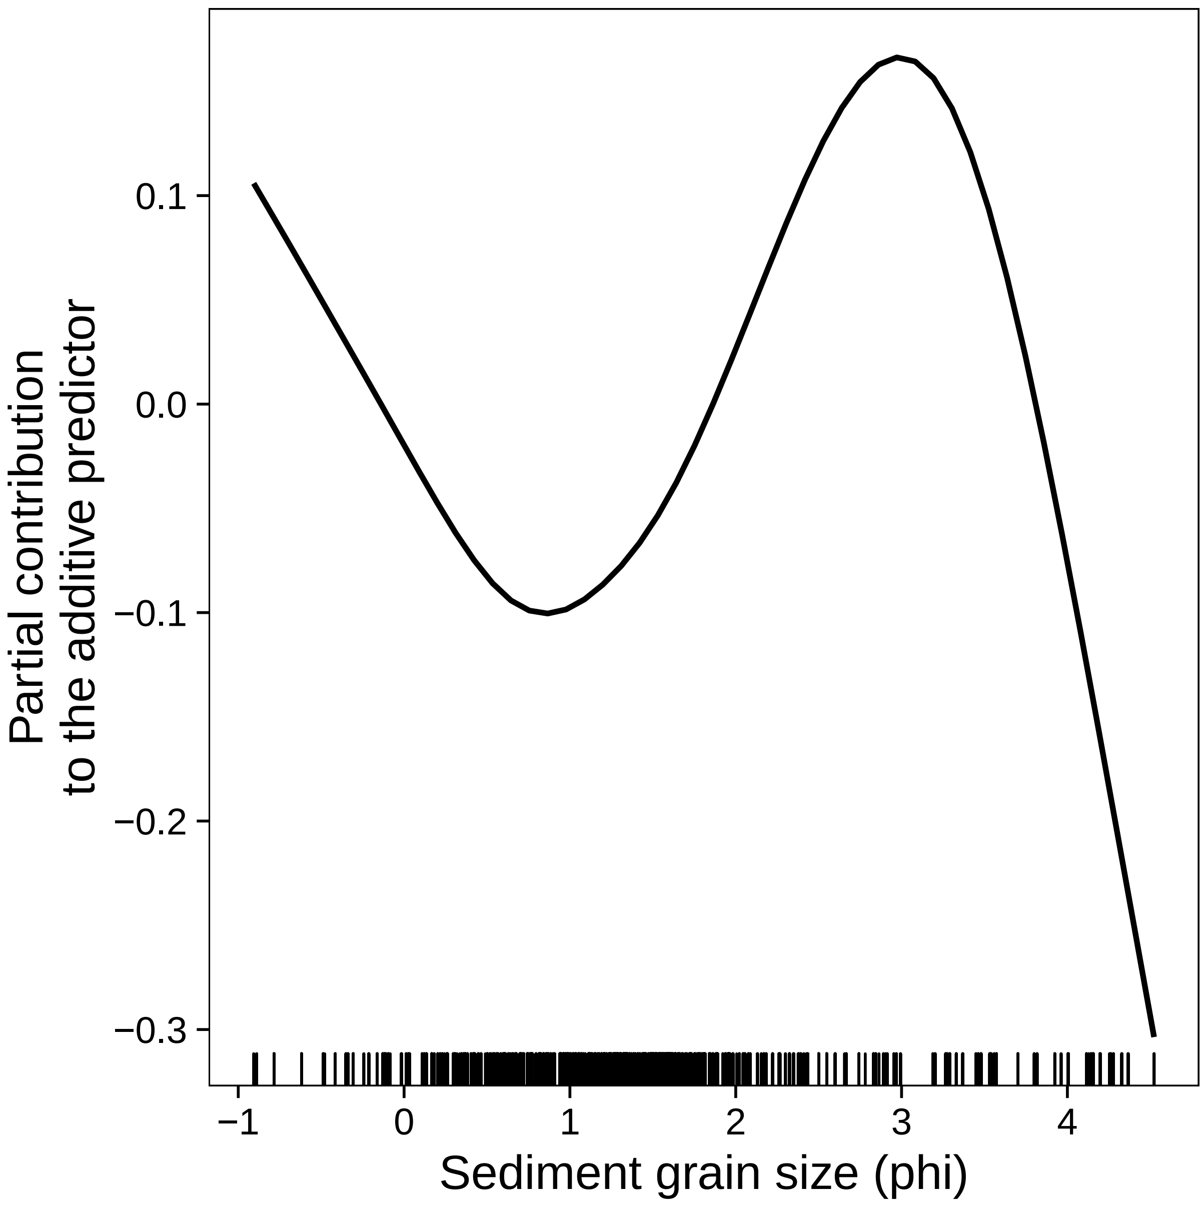
Partial contribution
to the additive predictor
0.1
0.0
−0.1
−0.2
−0.3
−1
0
1
2
3
4
Sediment grain size (phi)

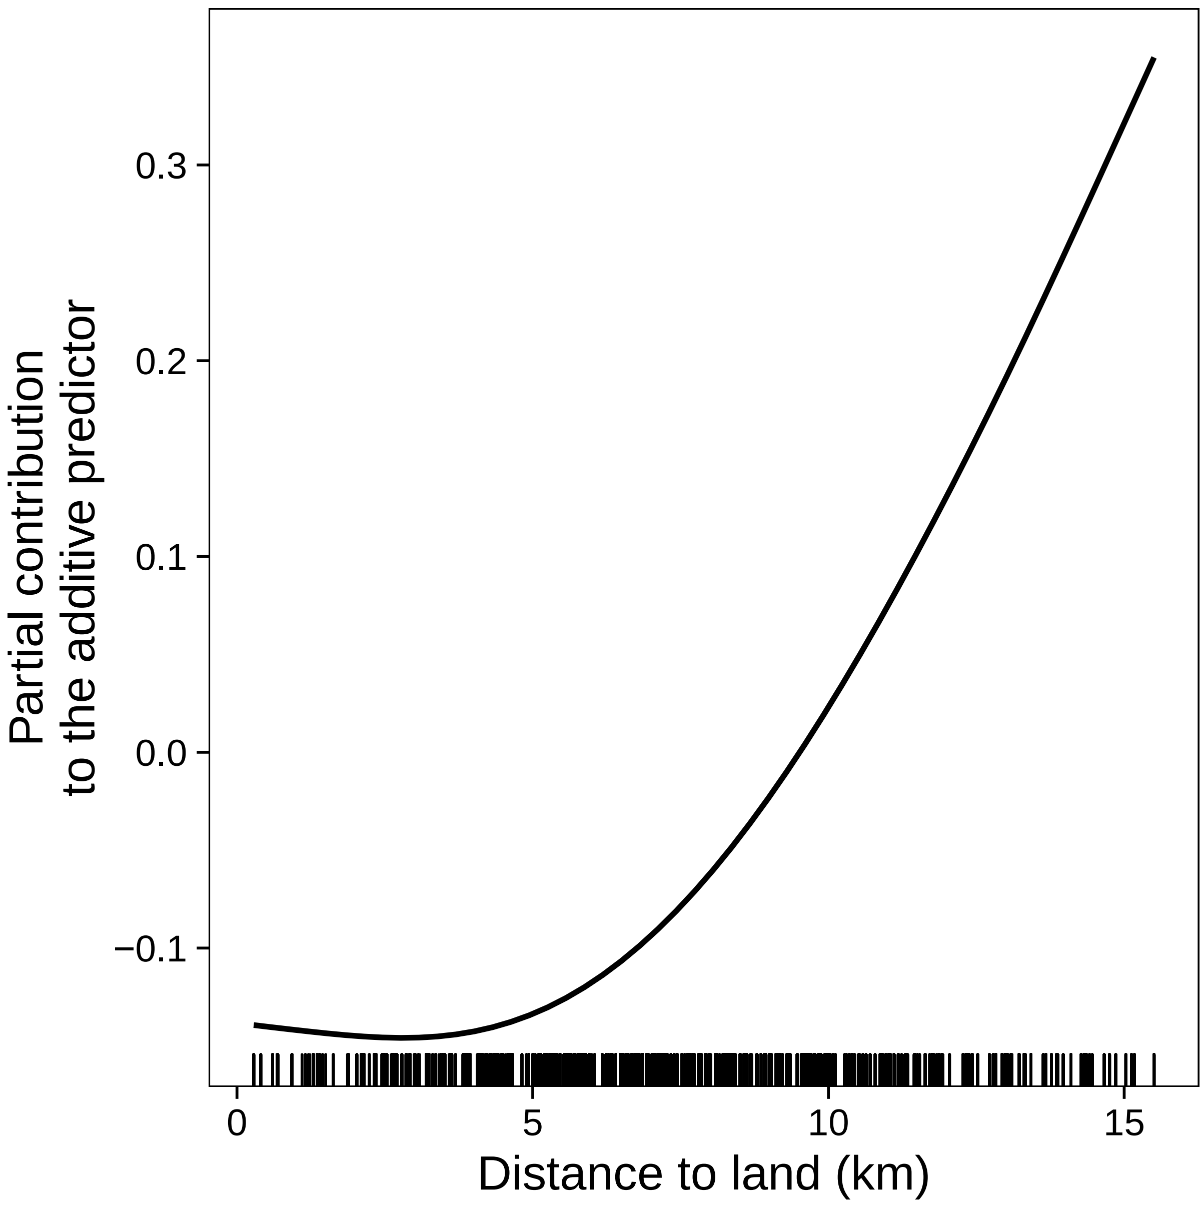
Partial contribution
to the additive predictor
Distance to land (km)
0.3
0.2
0.1
0.0
−0.1
0
5
10
15

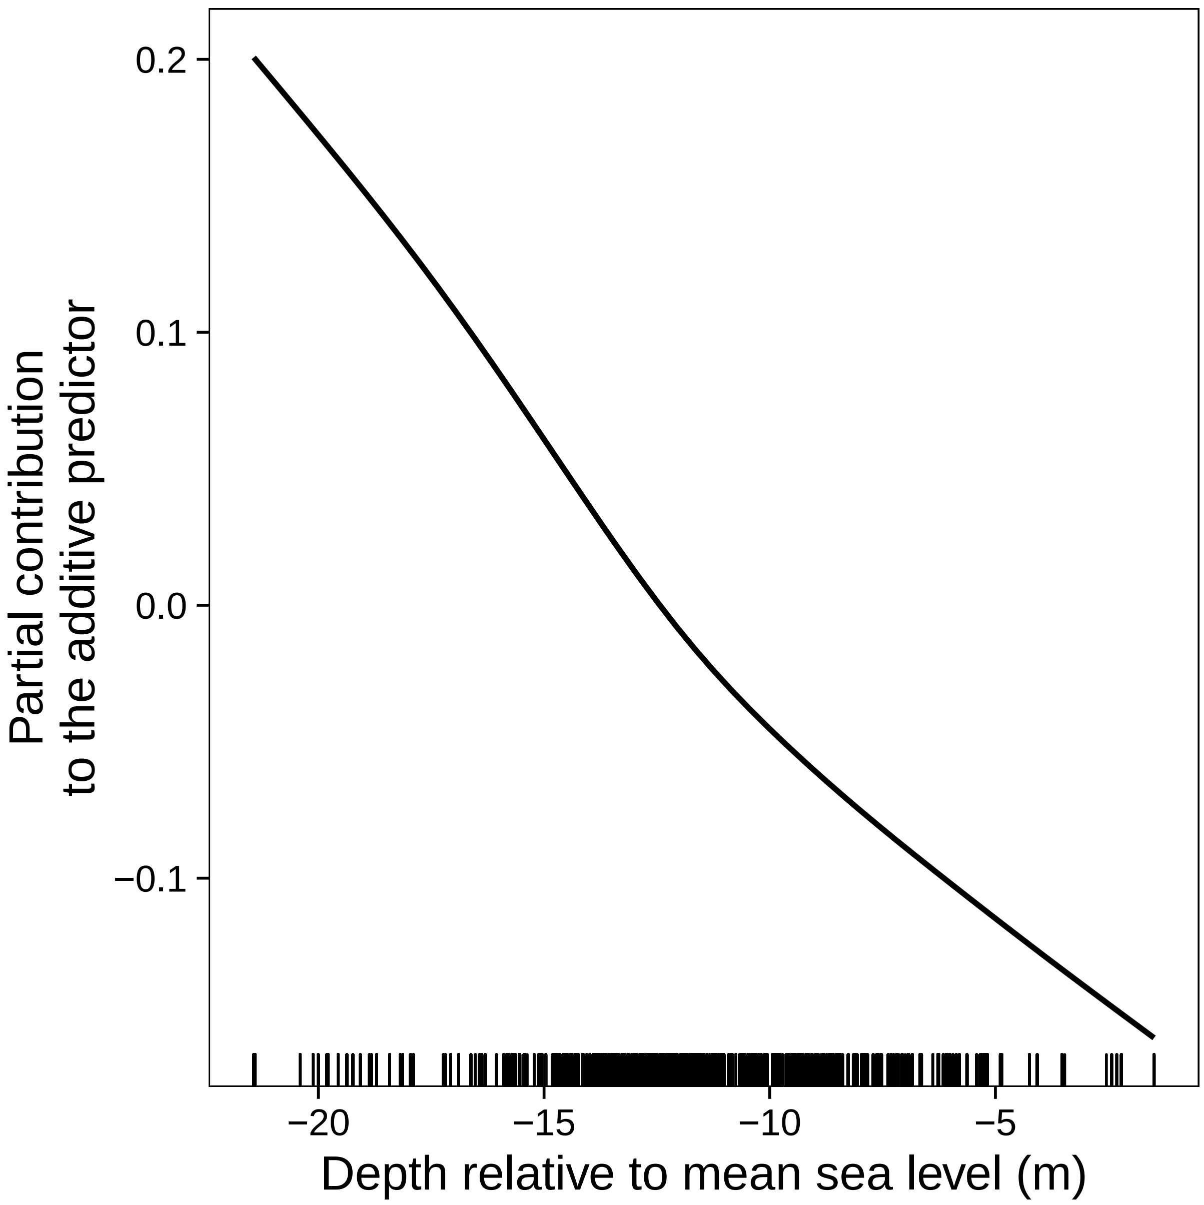
Partial contribution
to the additive predictor
0.2
0.1
0.0
−0.1
−20
−15
−10
−5
Depth relative to mean sea level (m)

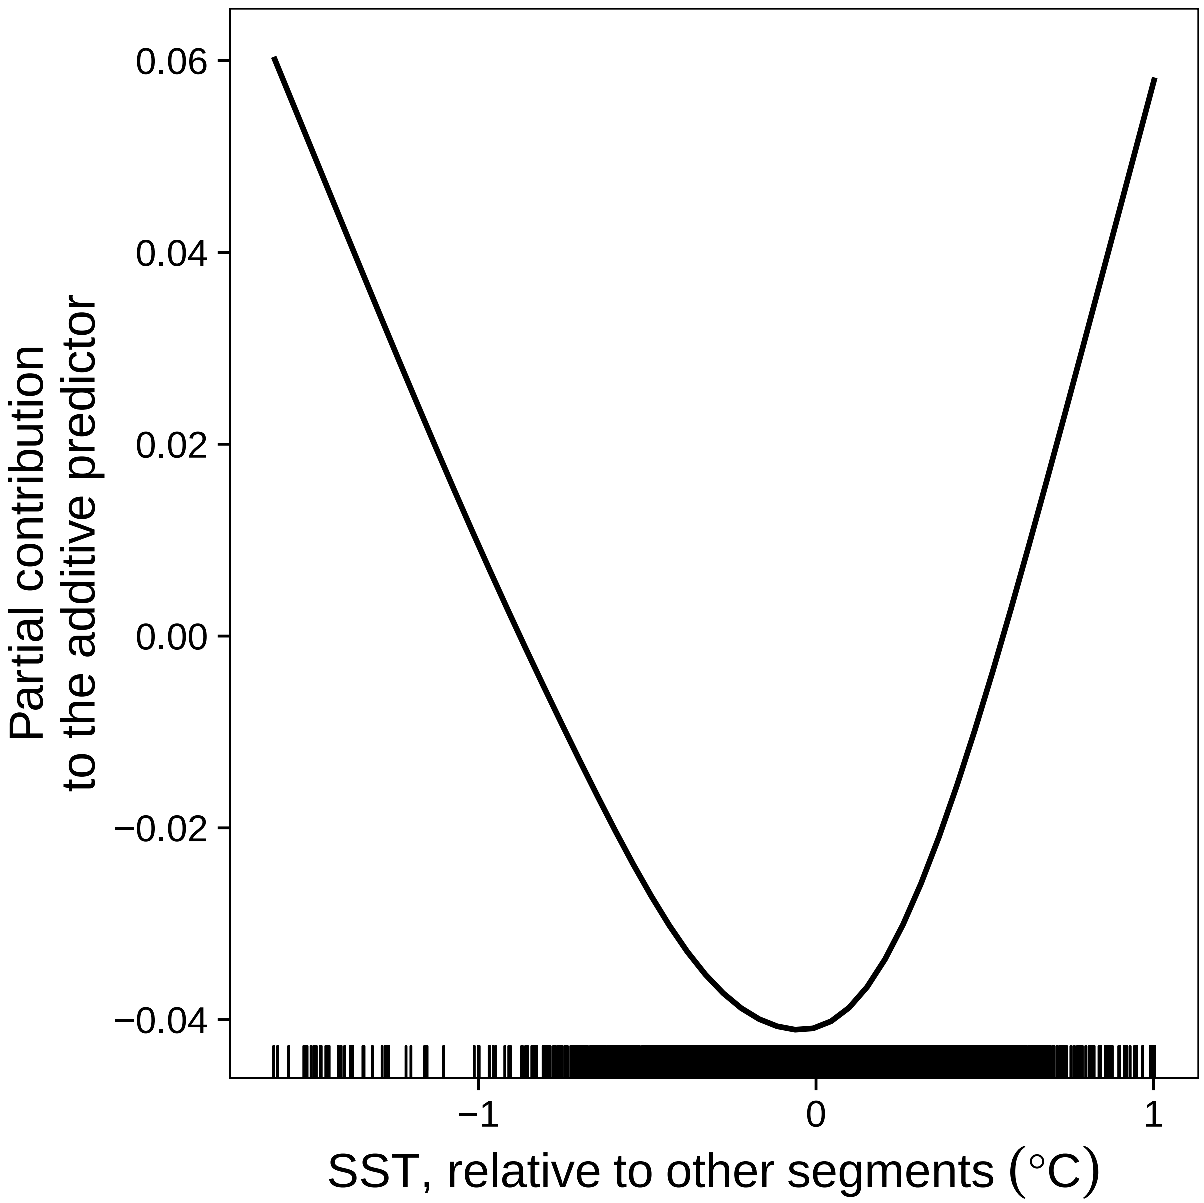
Partial contribution
to the additive predictor
0.06
0.04
0.02
0.00
−0.02
−0.04
−1
0
1
SST, relative to other segments (°C)

## Conditional mean

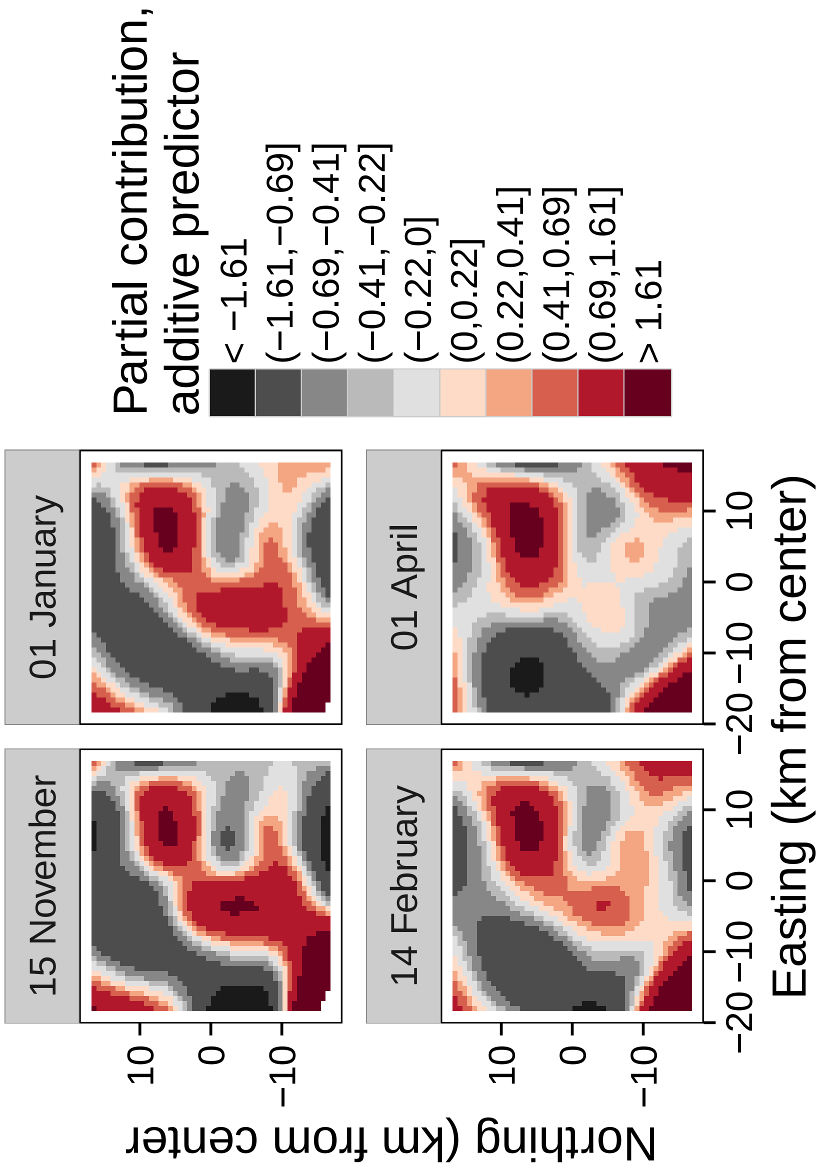

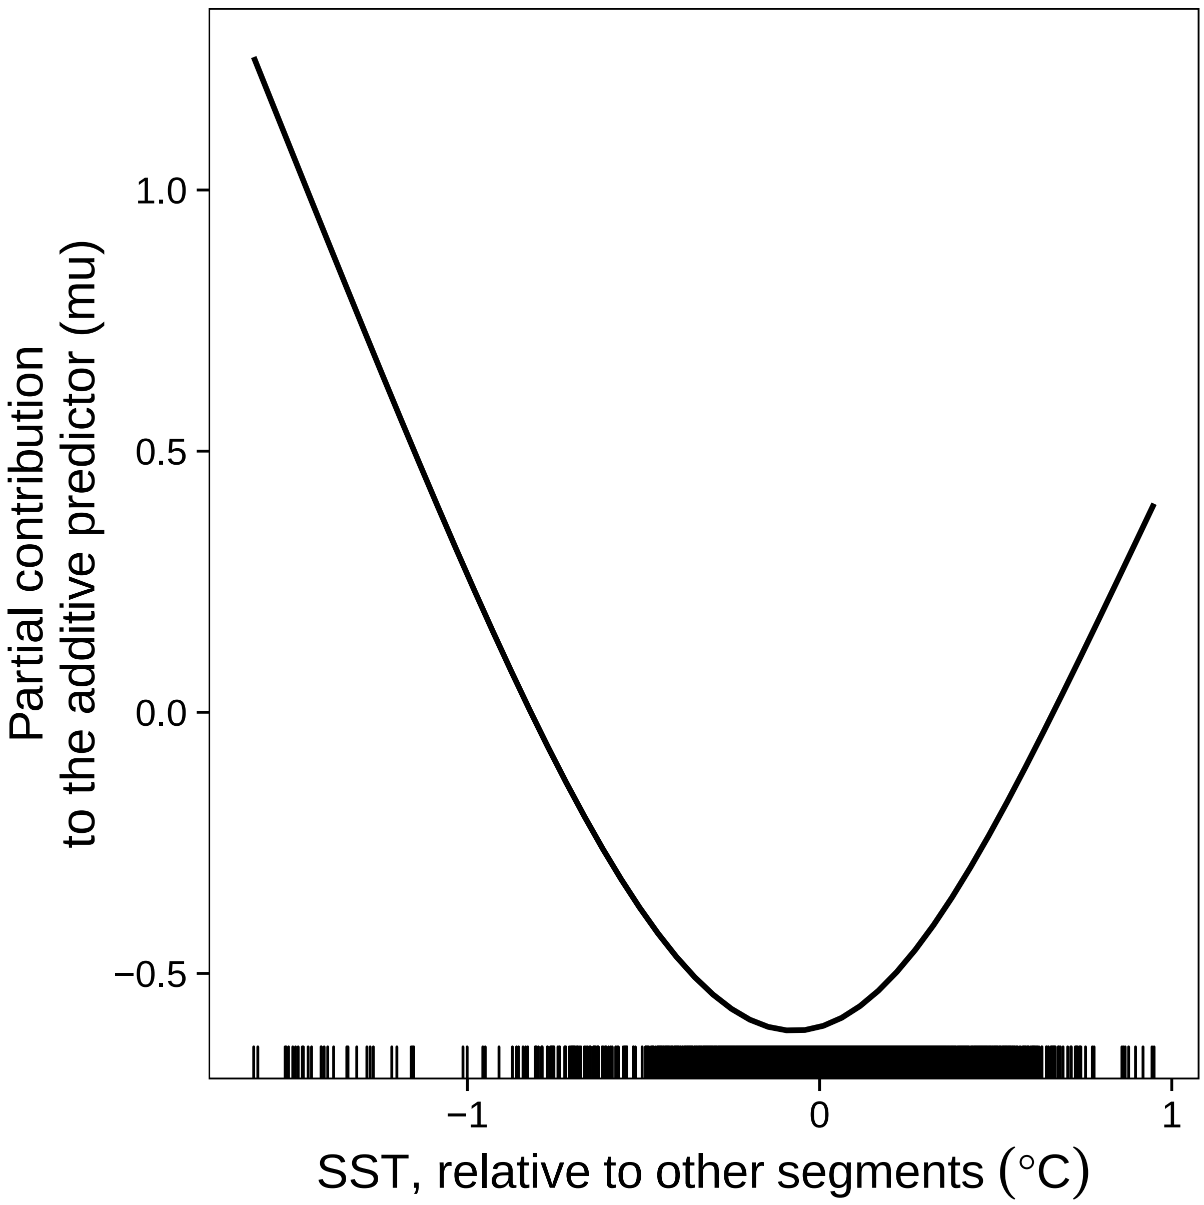

Partial contribution
to the additive predictor (mu)
1.0
0.5
0.0
−0.5
−1
0
1
SST, relative to other segments (°C)


24

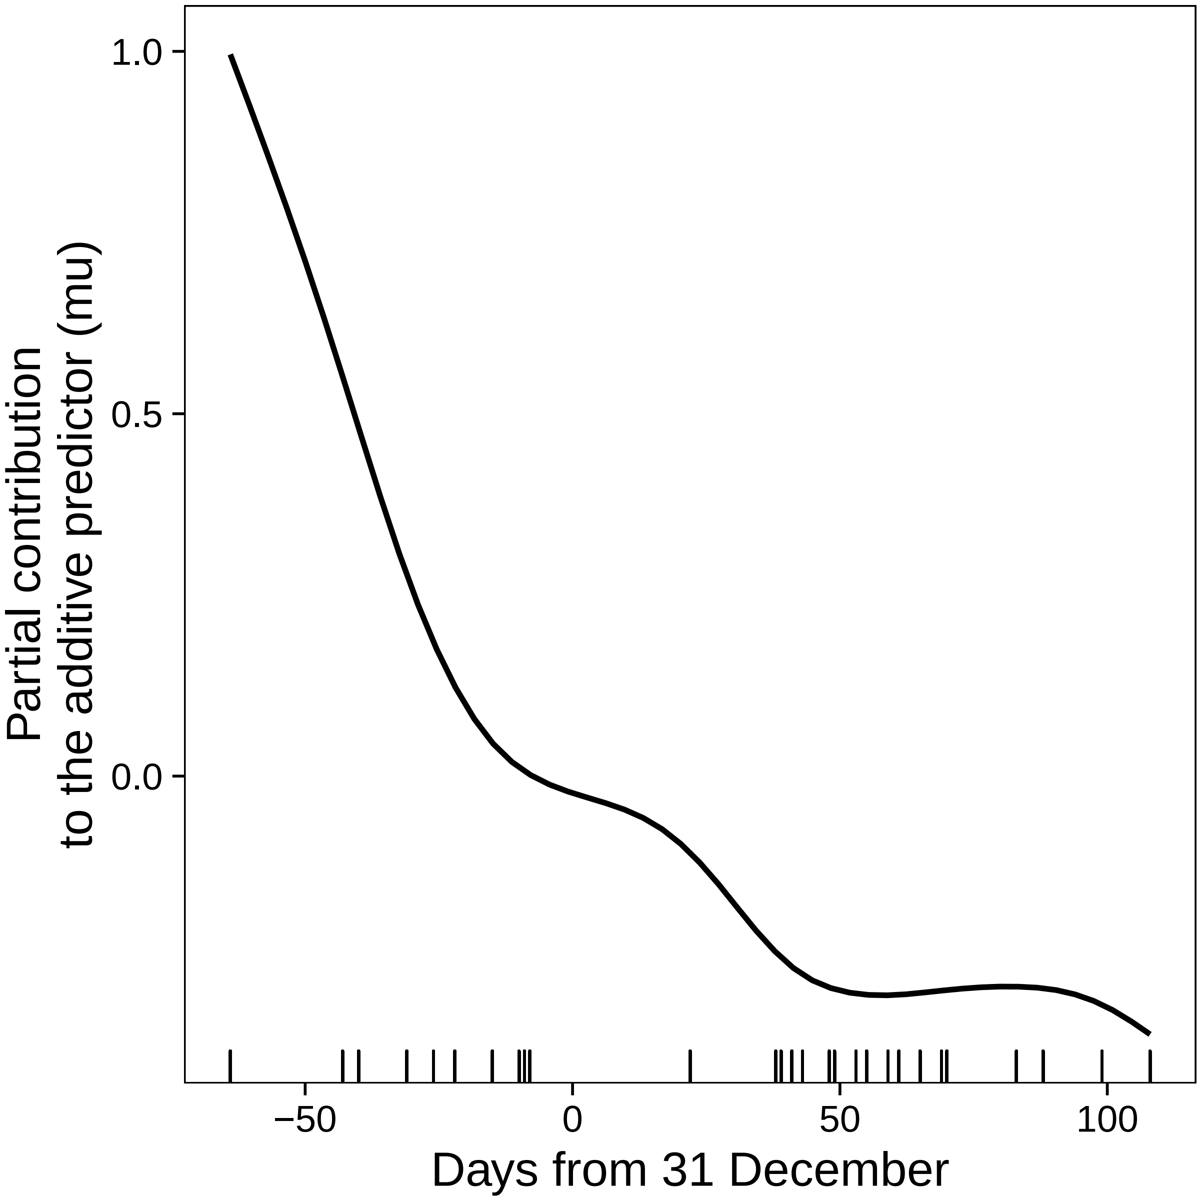
Partial contribution
to the additive predictor (mu)
1.0
0.5
0.0
−50
0
50
100
Days from 31 December

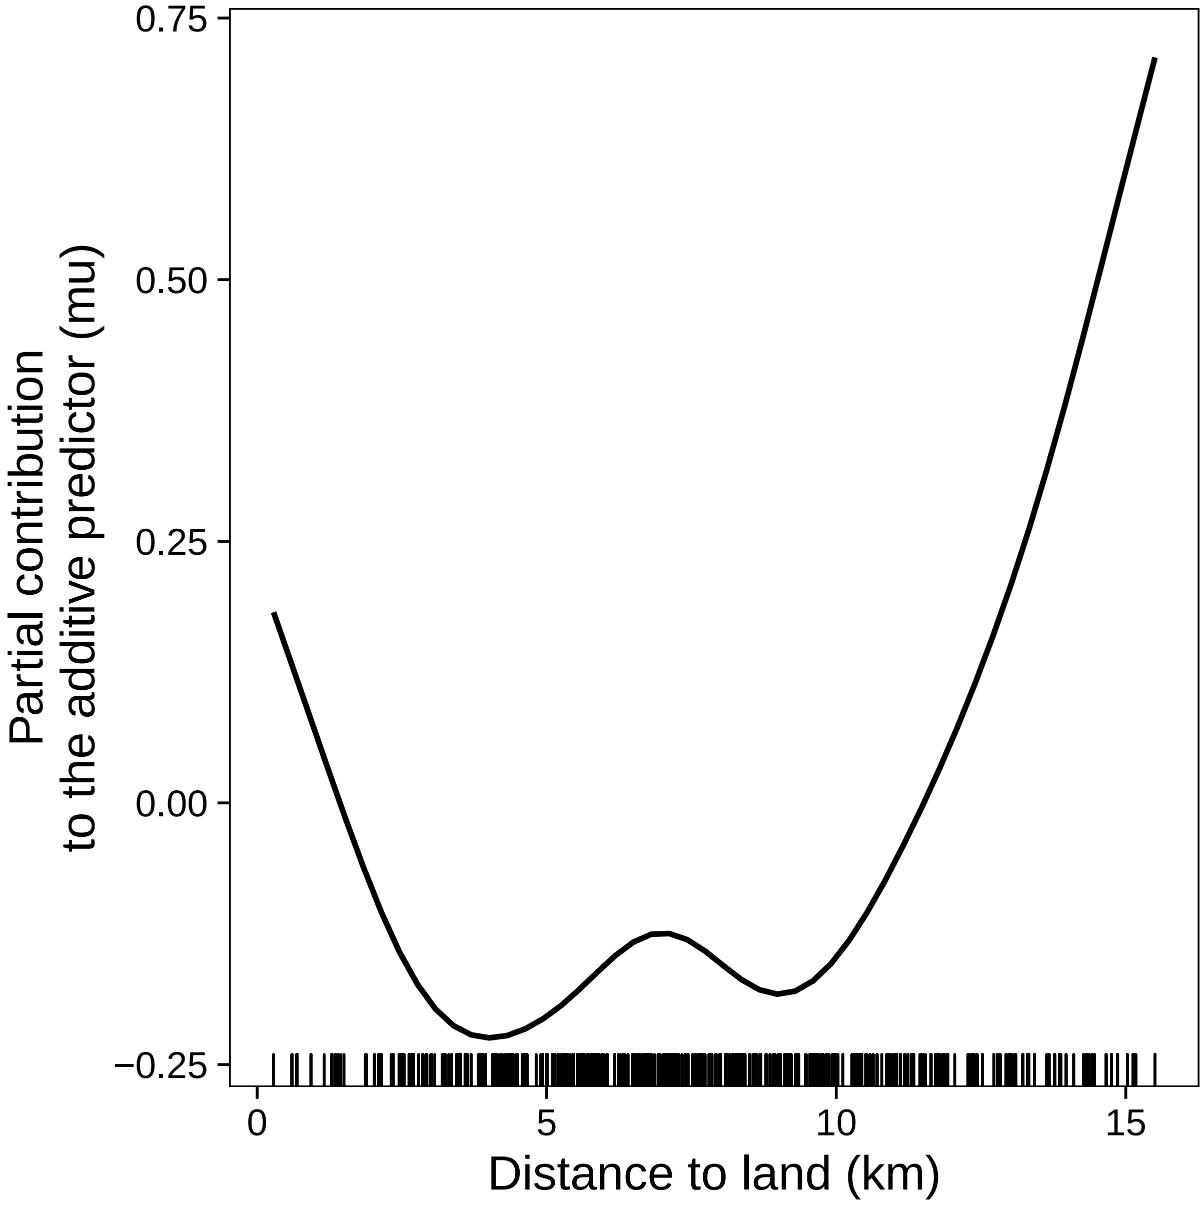

Partial contribution
to the additive predictor (mu)
0.75
0.50
0.25
0.00
−0.25
0
5
10
15
Distance to land (km)

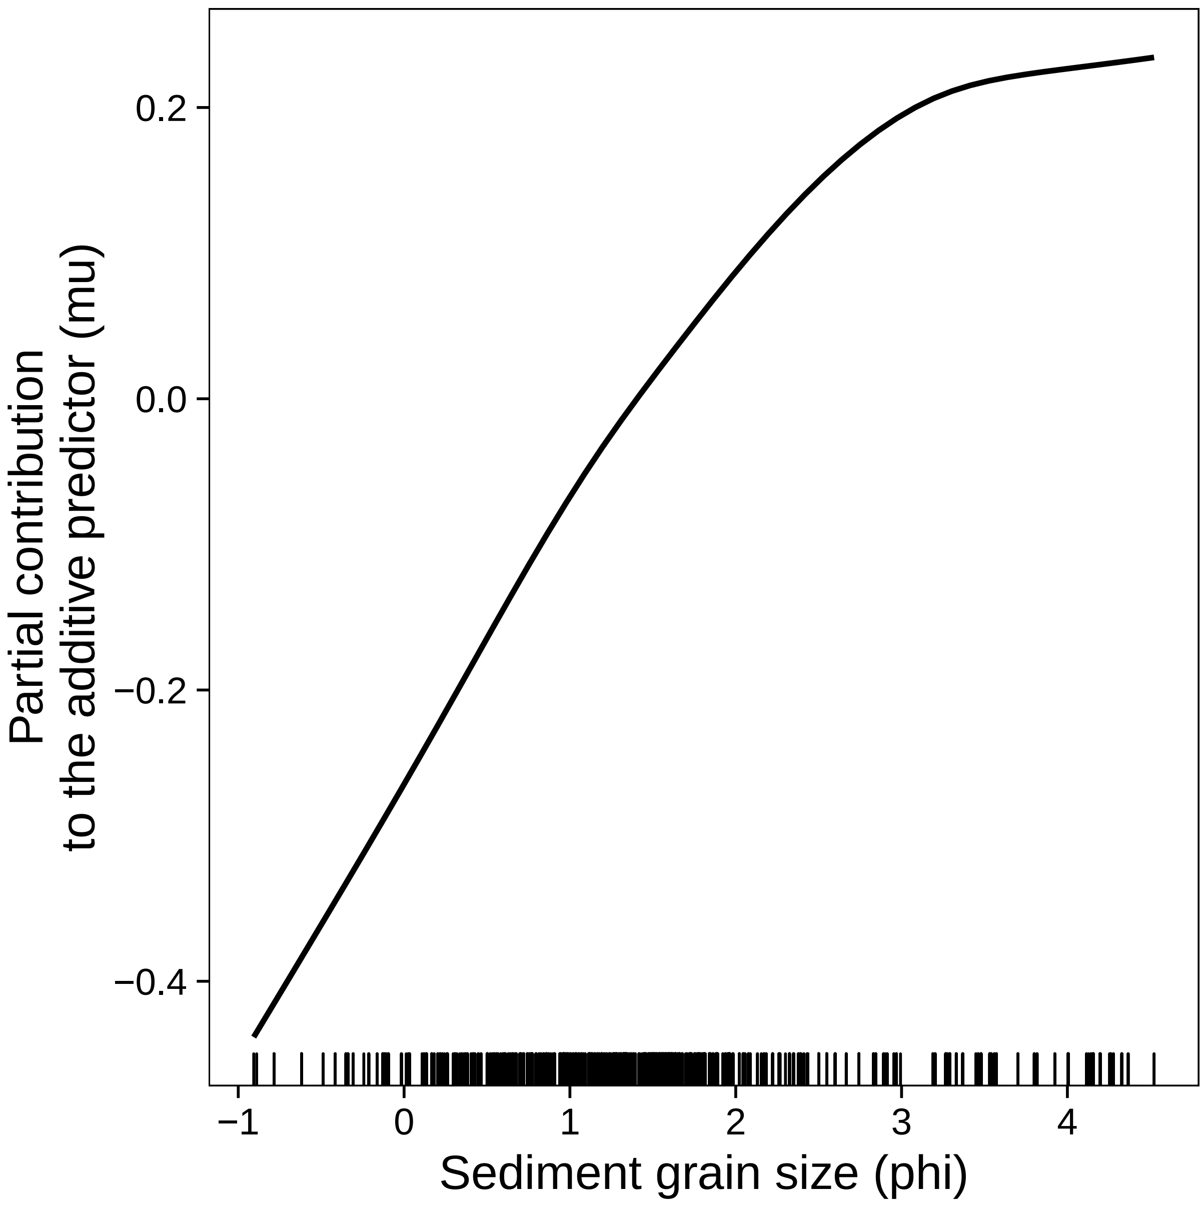

Partial contribution
to the additive predictor (mu)
0.2
0.0
−0.2
−0.4
−1
0
1
2
3
4
Sediment grain size (phi)


27

## Conditional overdispersion

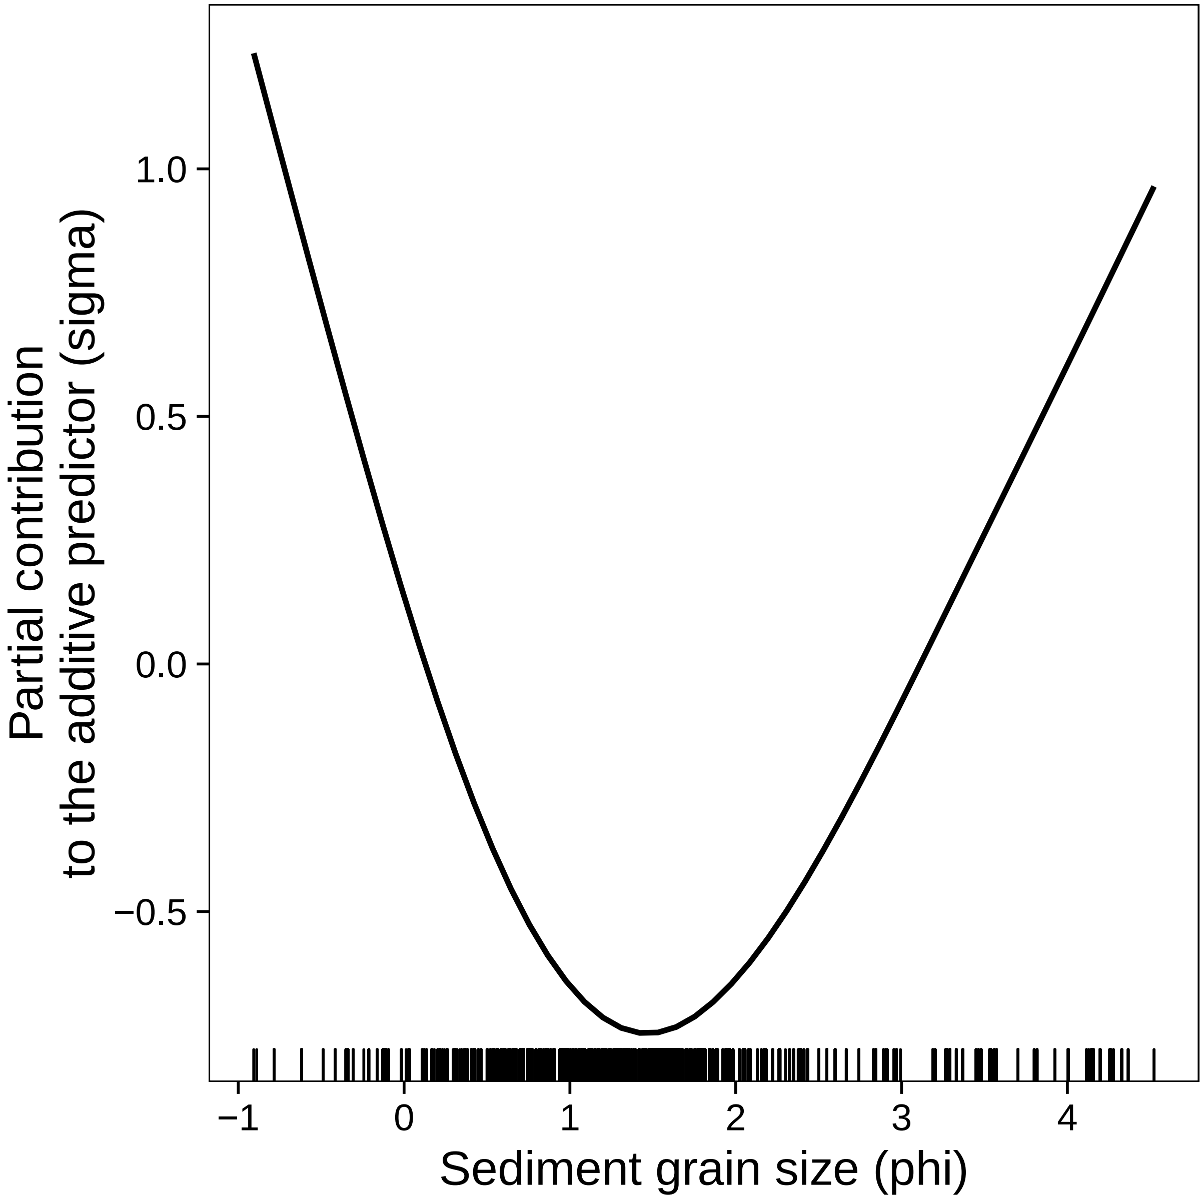

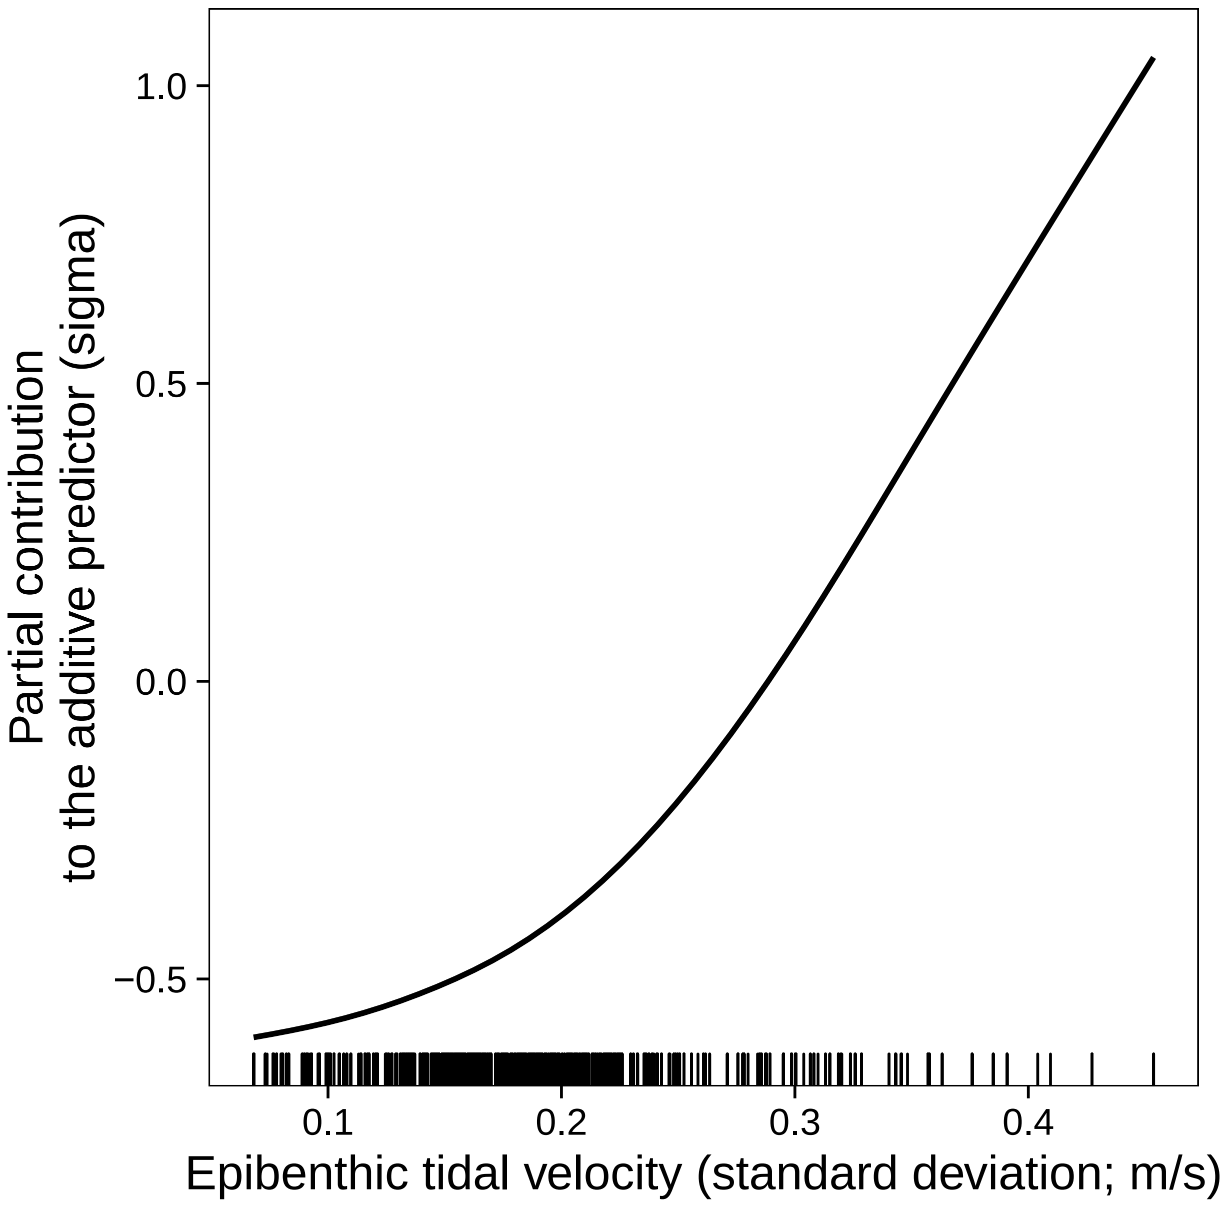
Partial contribution
to the additive predictor (sigma)
1.0
0.5
0.0
−0.5
0.1
0.2
0.3
0.4
Epibenthic tidal velocity (standard deviation; m/s)

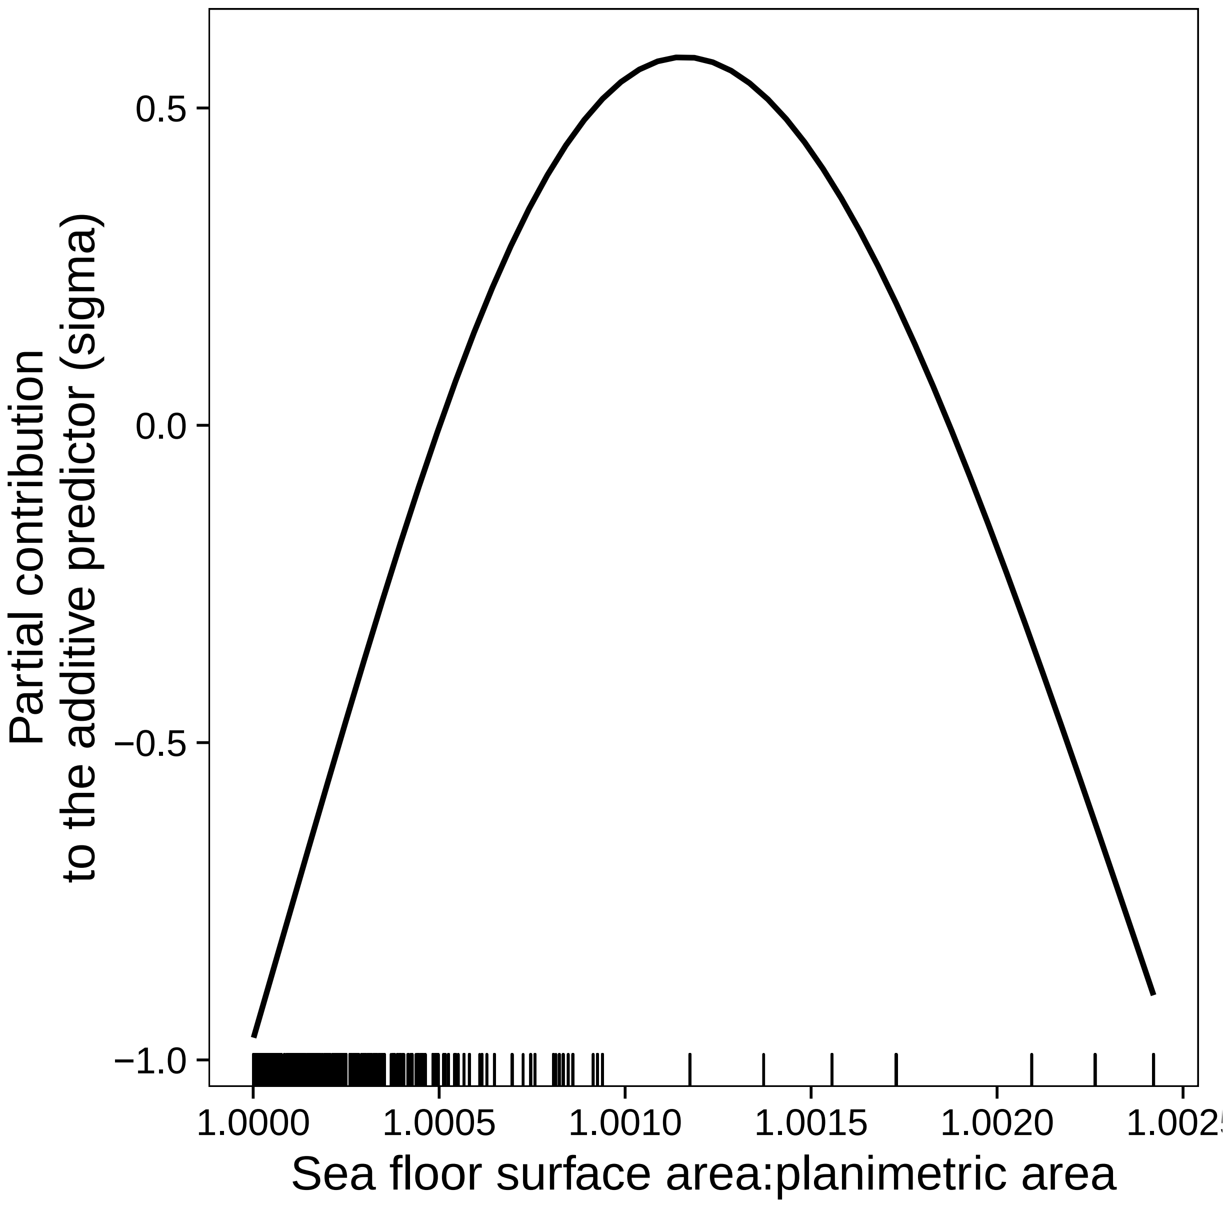
0.5
0.0
−0.5
−1.0
Partial contribution
to the additive predictor (sigma)
1.0000
1.0005
1.0010
1.0015
1.0020
1.002
Sea floor surface area:planimetric area

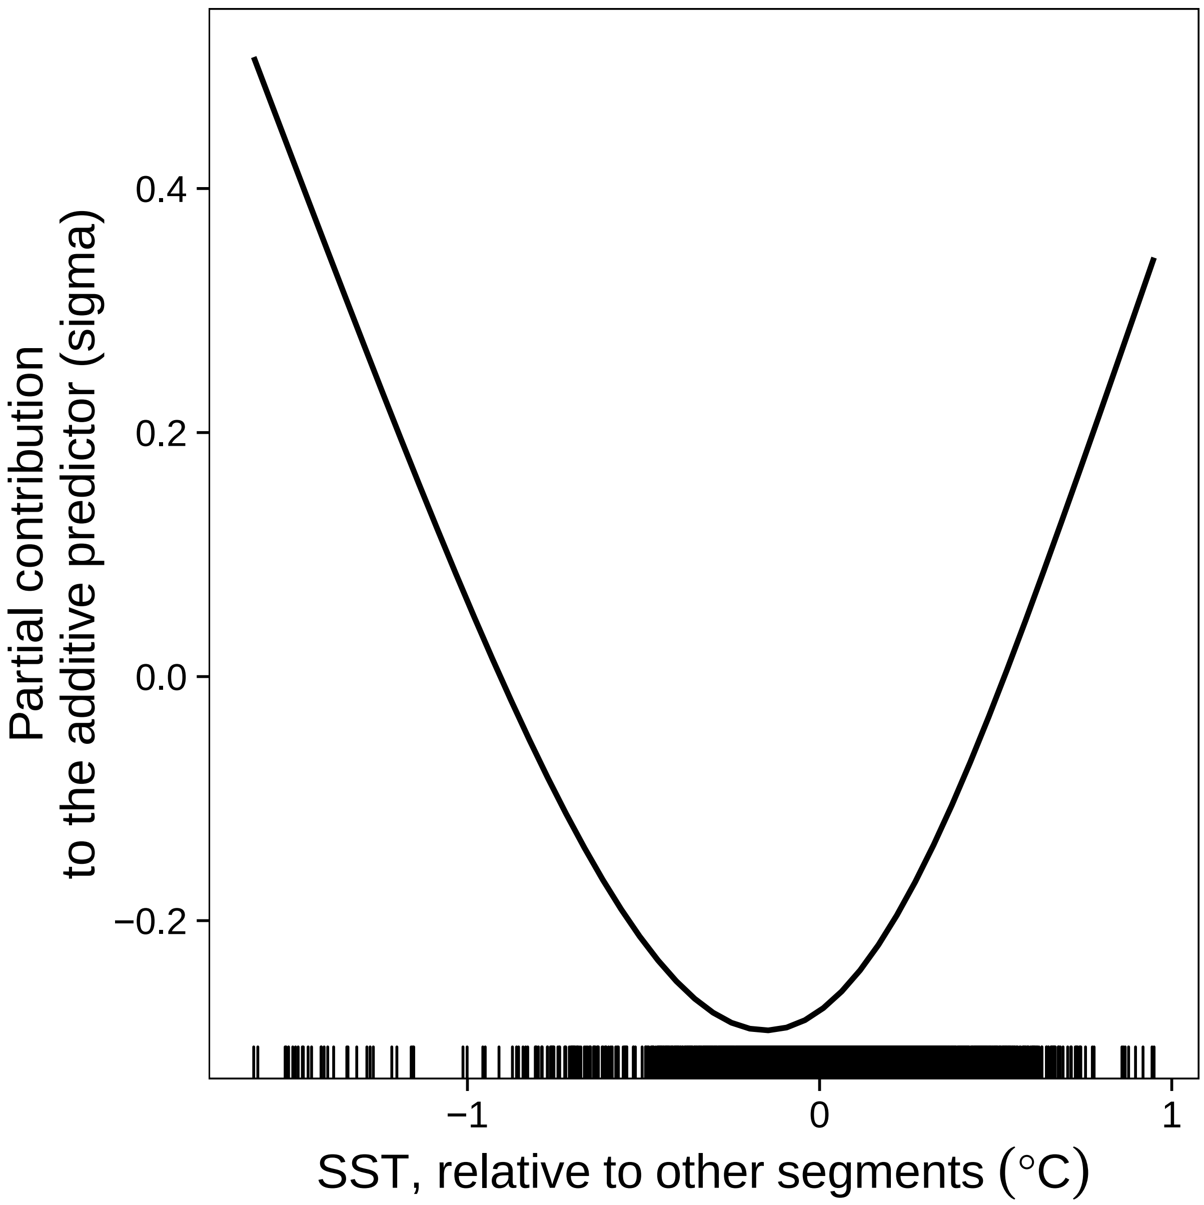
Partial contribution
to the additive predictor (sigma)
0.4
0.2
0.0
−0.2
−1
0
1
SST, relative to other segments (°C)

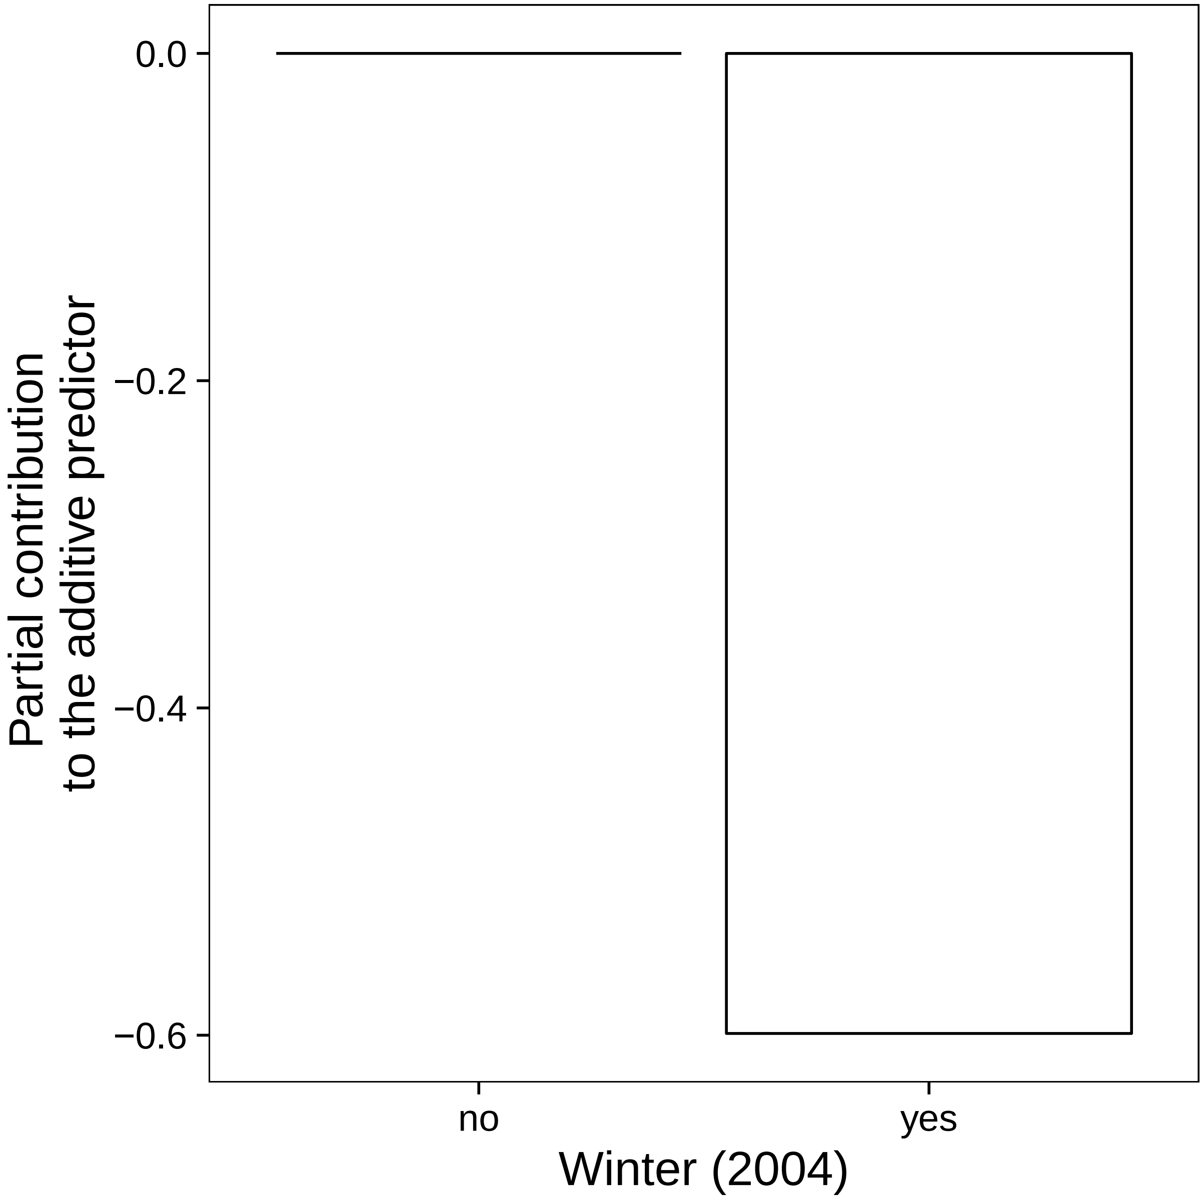

0.0
−0.2
−0.4
−0.6
Partial contribution
to the additive predictor
no
yes
Winter (2004)


33

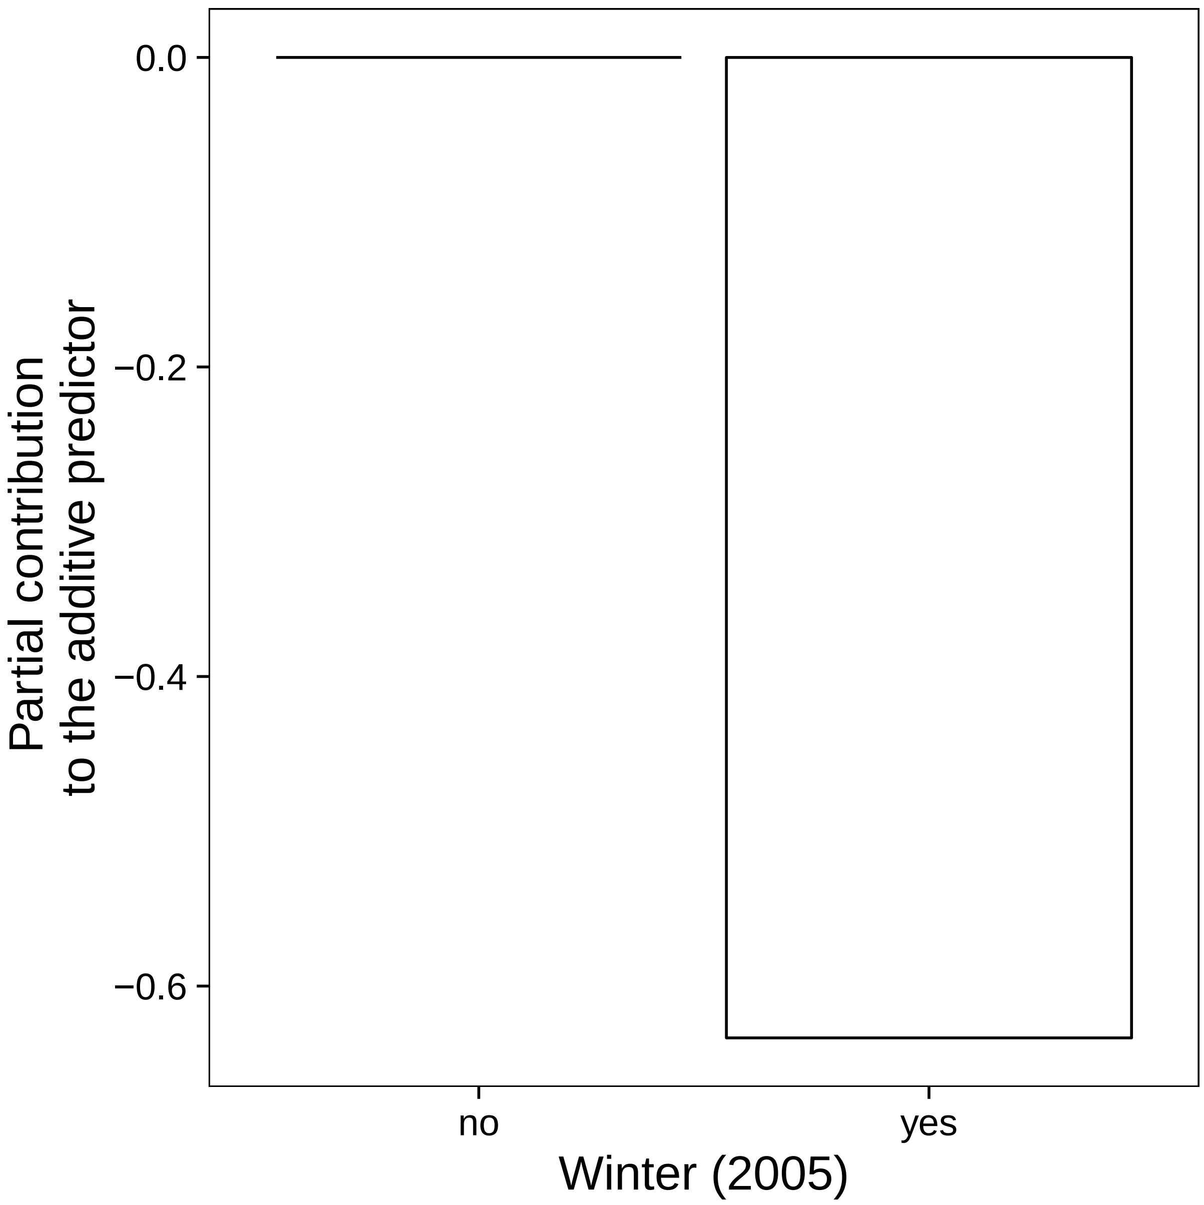
0.0
−0.2
−0.4
−0.6
Partial contribution
to the additive predictor
no
yes
Winter (2005)
