# Supplementary material for: Spatiotemporal modelling of sea duck abundance: implications for marine spatial planning
Source: arXiv:1705.00644 source file (2017-05-01)

## Appendix S5. Common Eider stable covariate effects

Marginal functional plots of the relationships between covariates (controlling for all other variables; i.e., at their mean values) and the occupancy, conditional mean abundance, and conditional overdispersion of abundance of Common Eider in Nantucket Sound, Massachusetts, USA. Covariate plots are ordered roughly in descending order of the magnitude of their influence on the additive predictor in each model (or model parameter for count models). Vertical lines along the  $x$ -axis (i.e., rug plots) indicate observed covariate values. Covariates (and any abbreviations) are defined in detail in Appendix S2; only effects selected to be stable (see Appendix S1) are depicted.

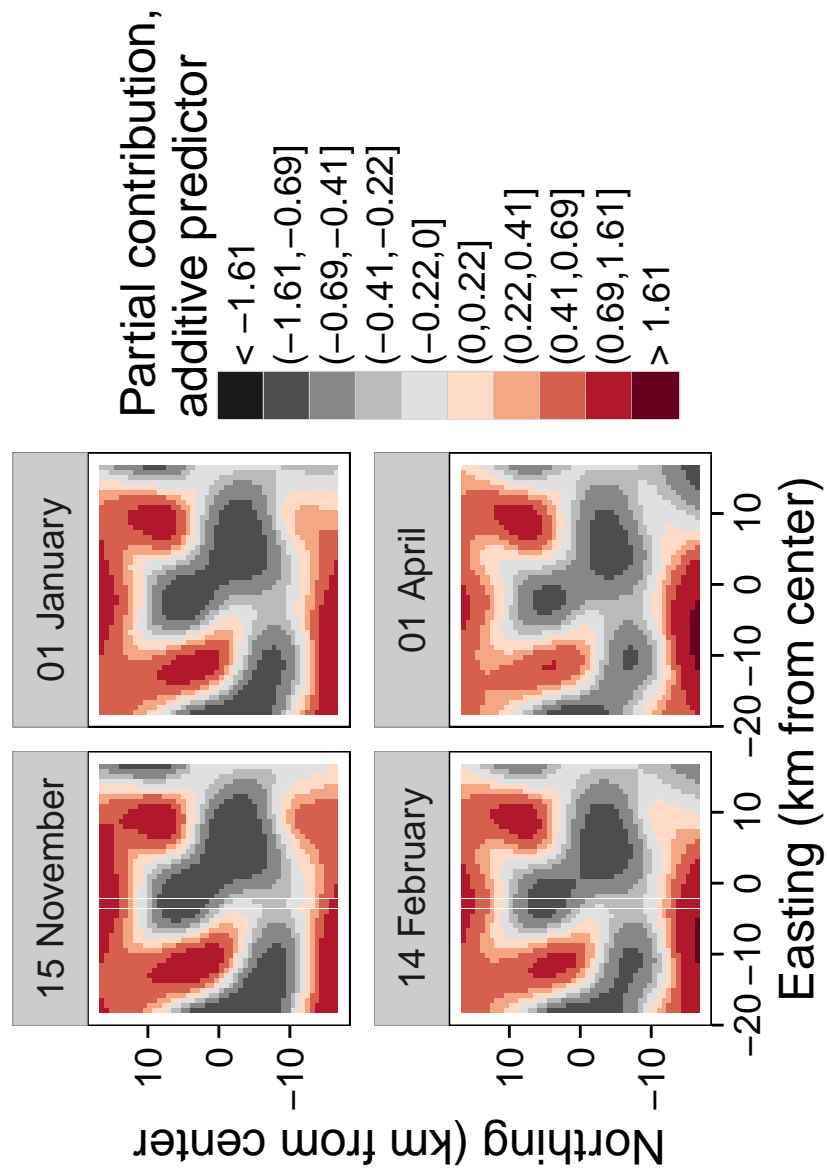

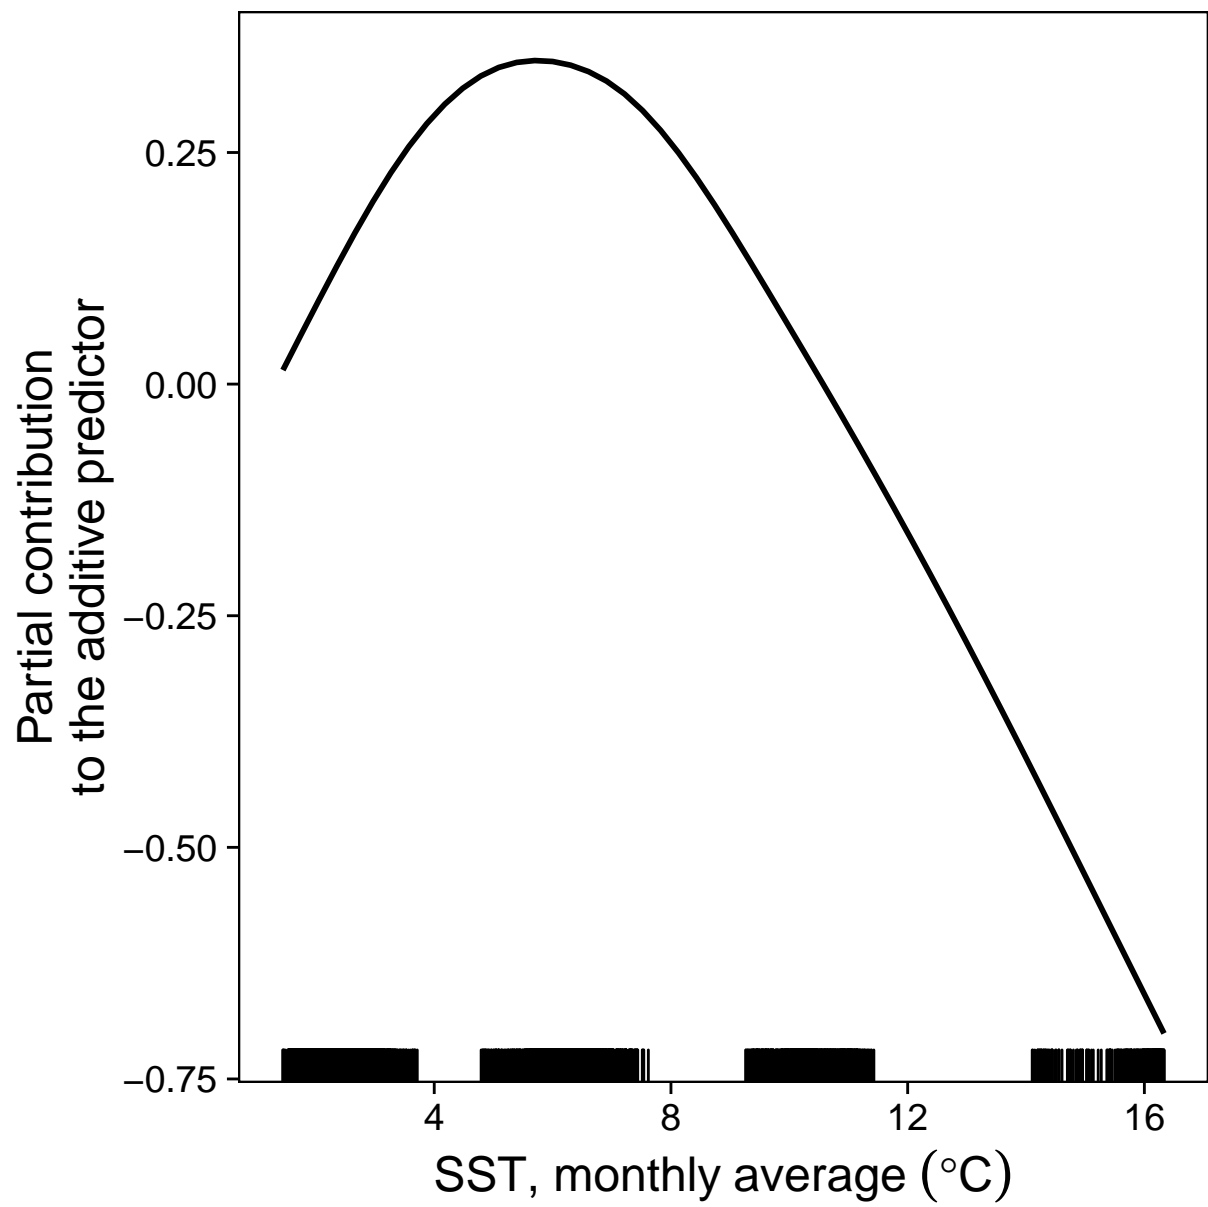

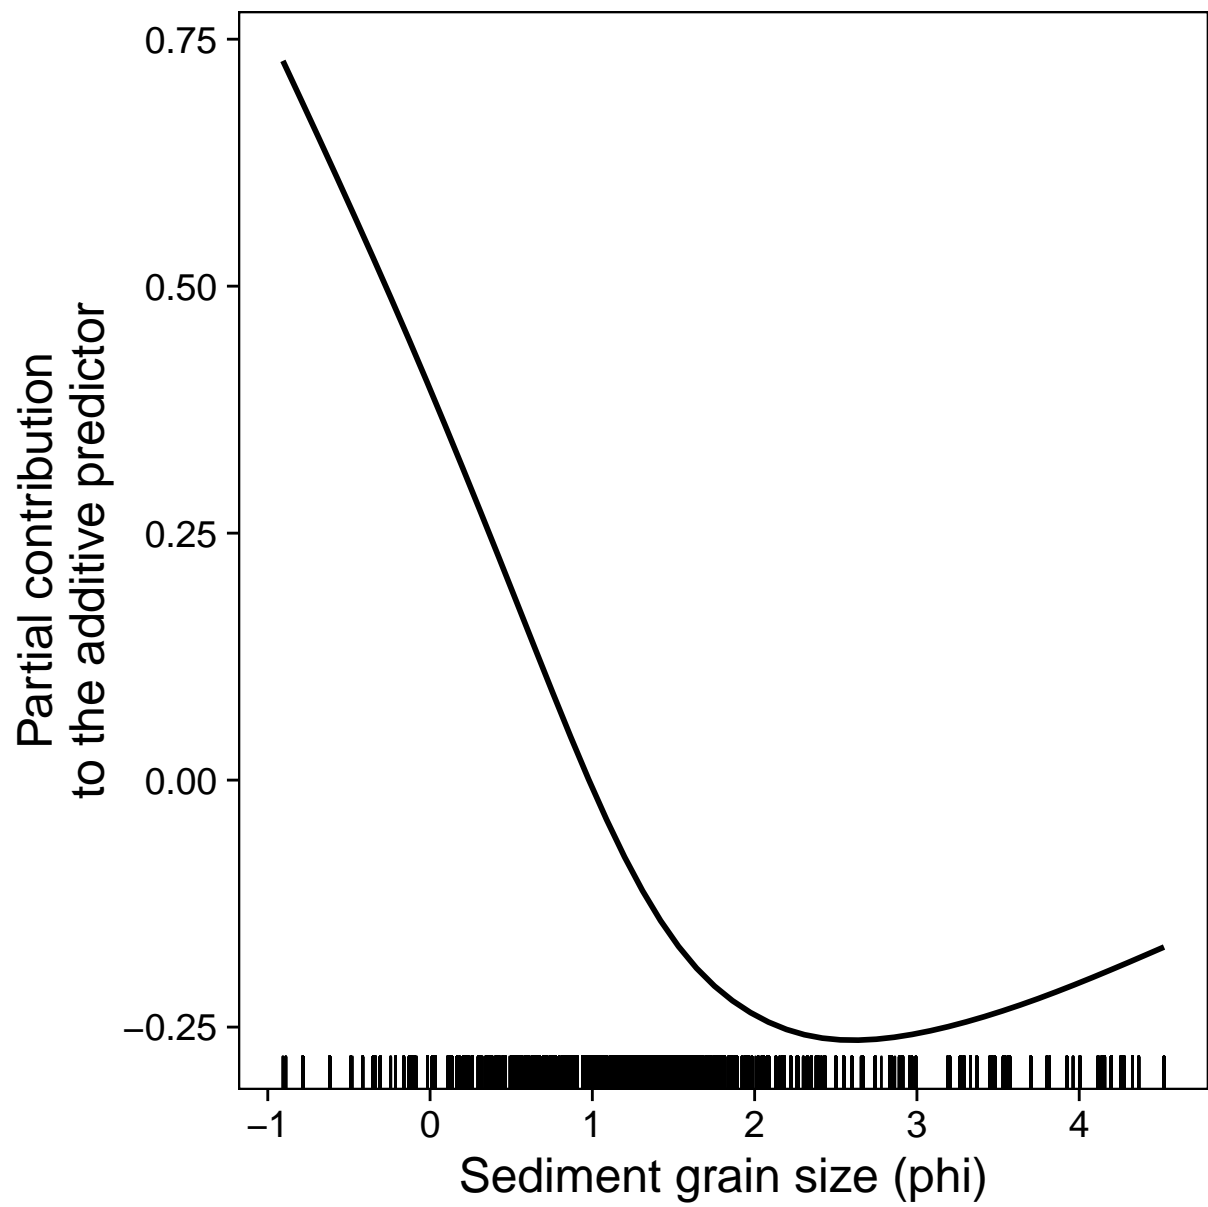

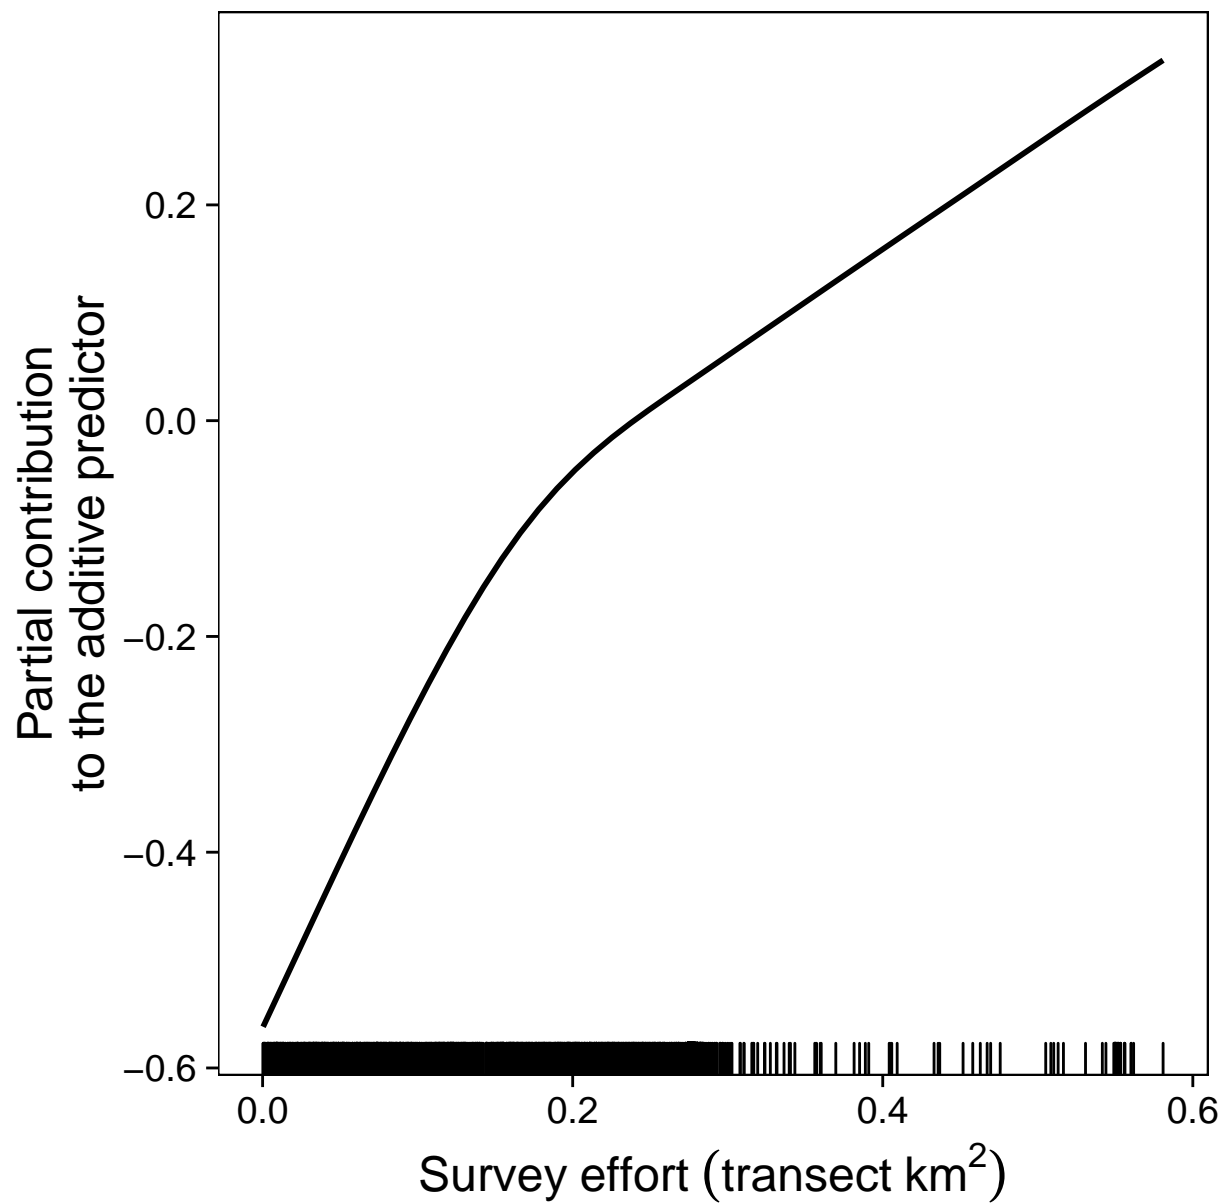

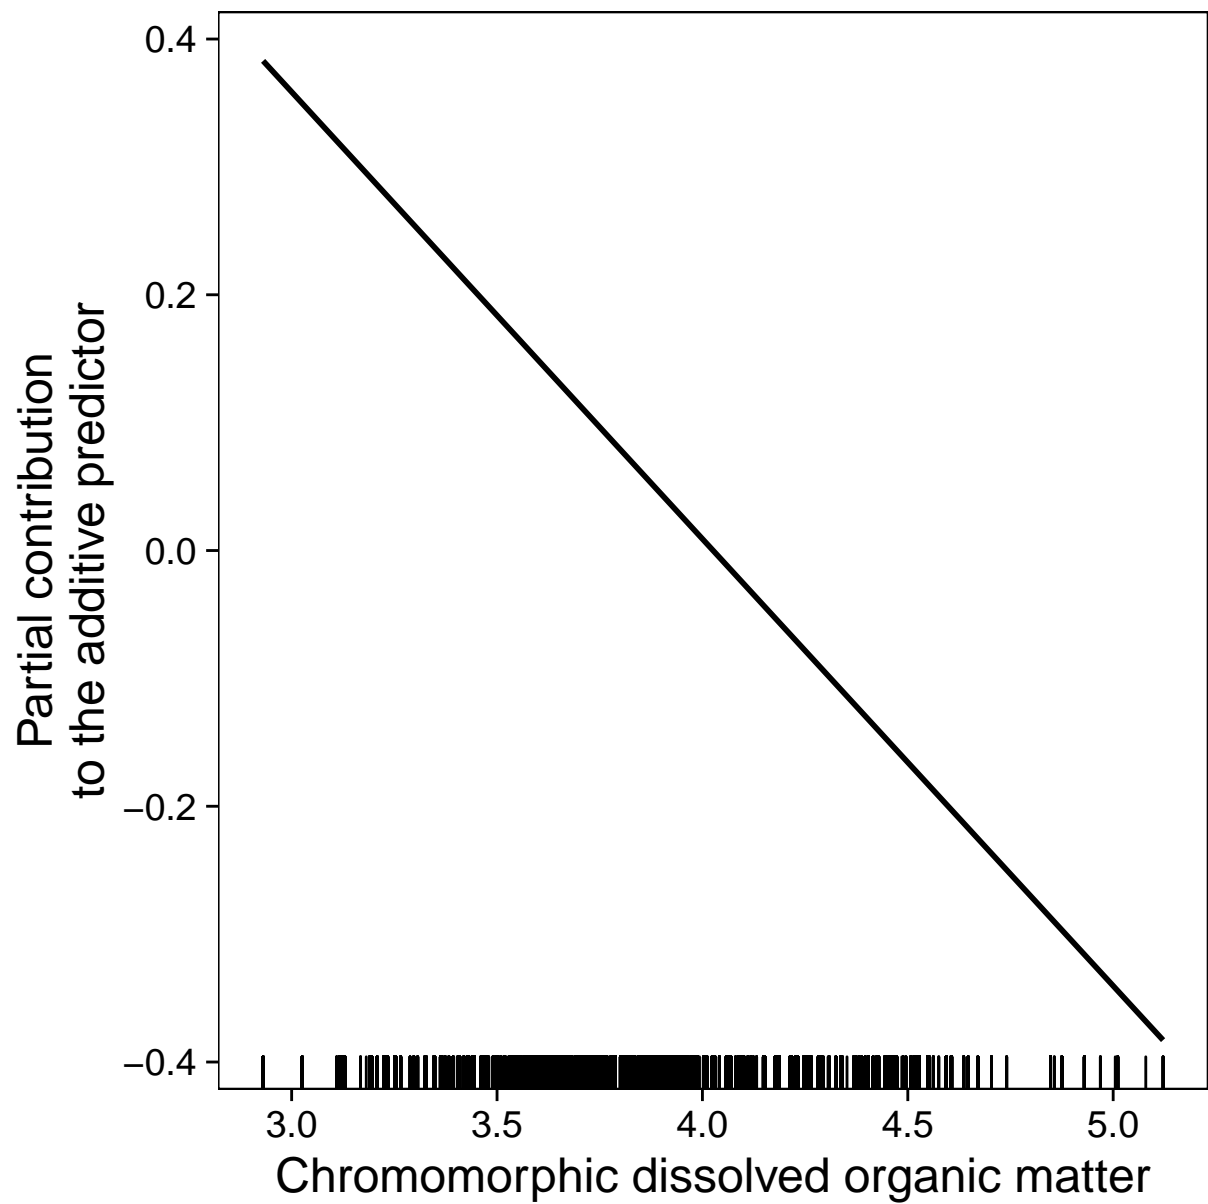

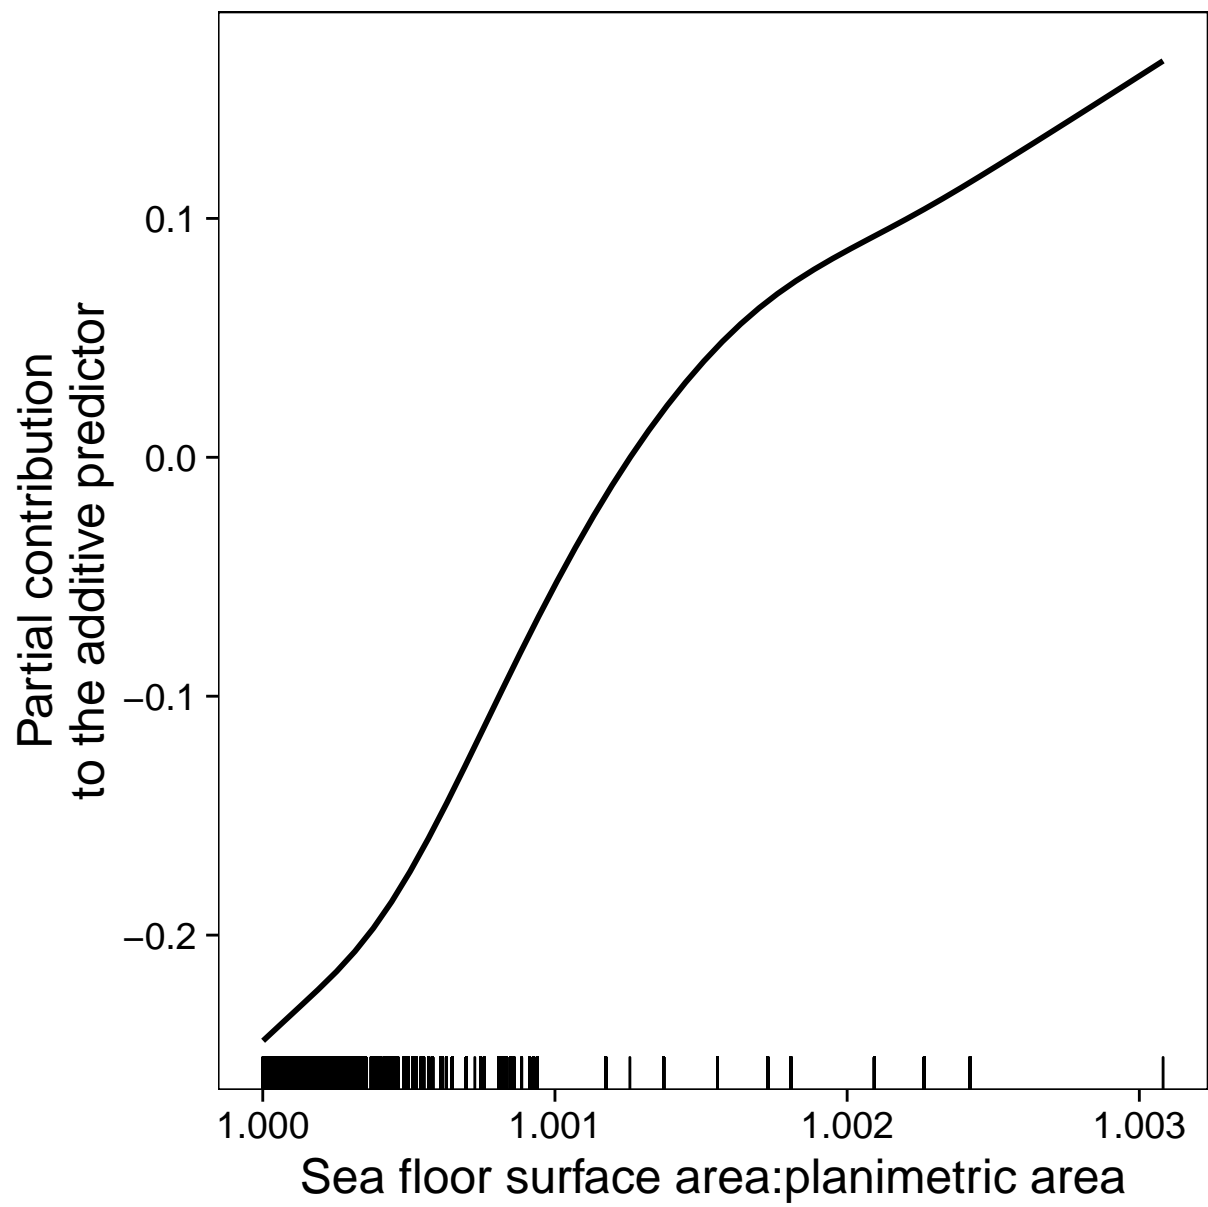

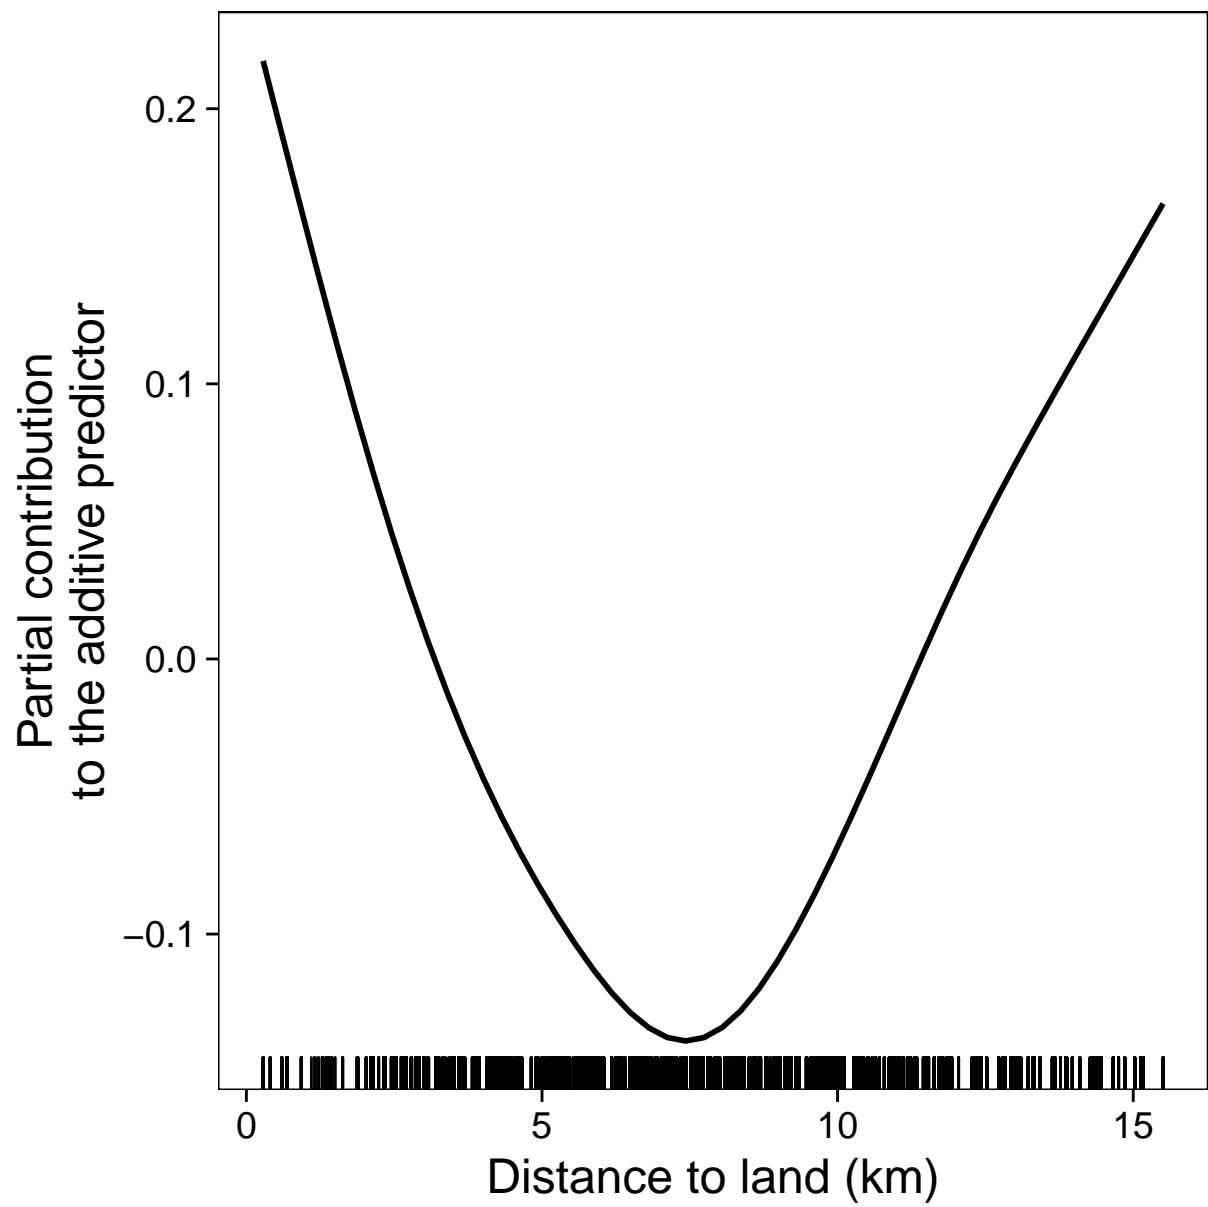

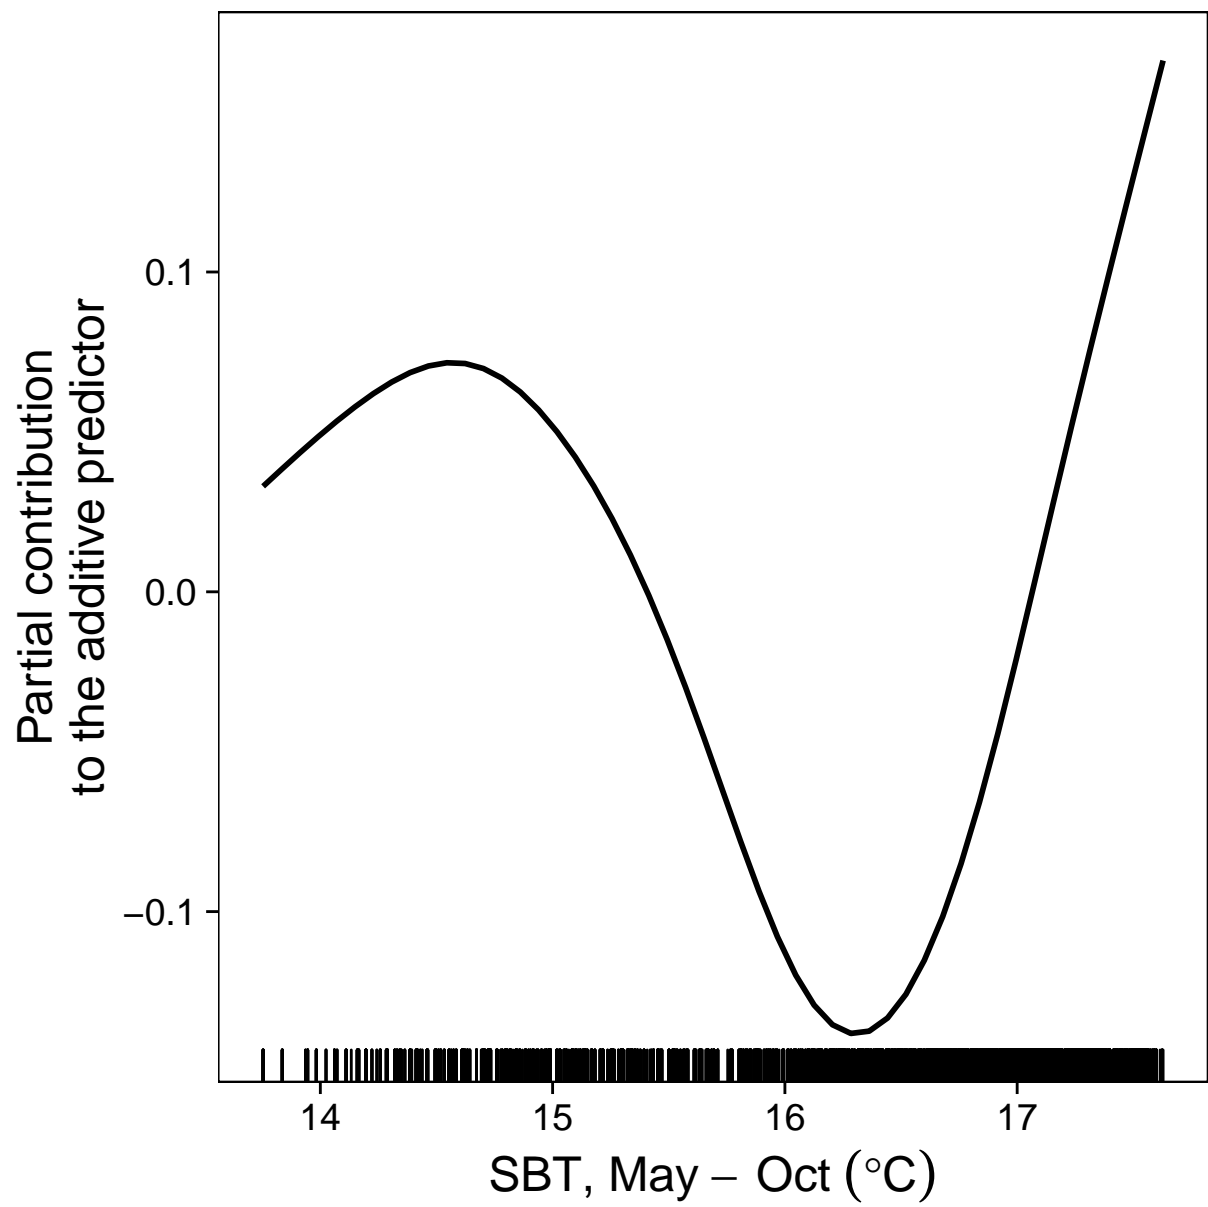

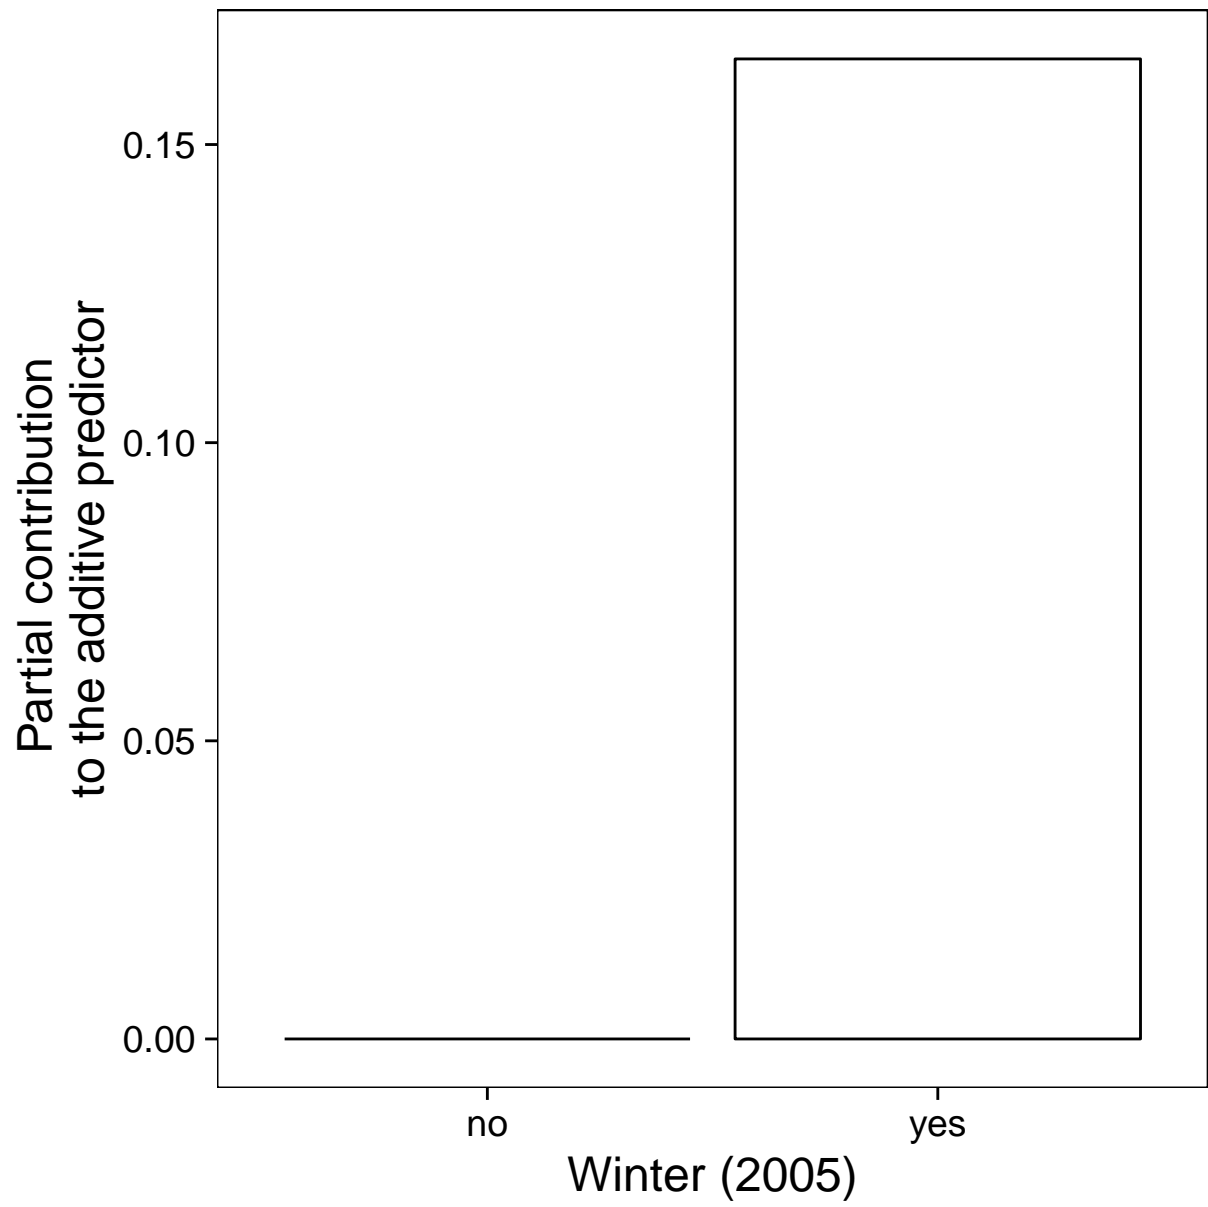

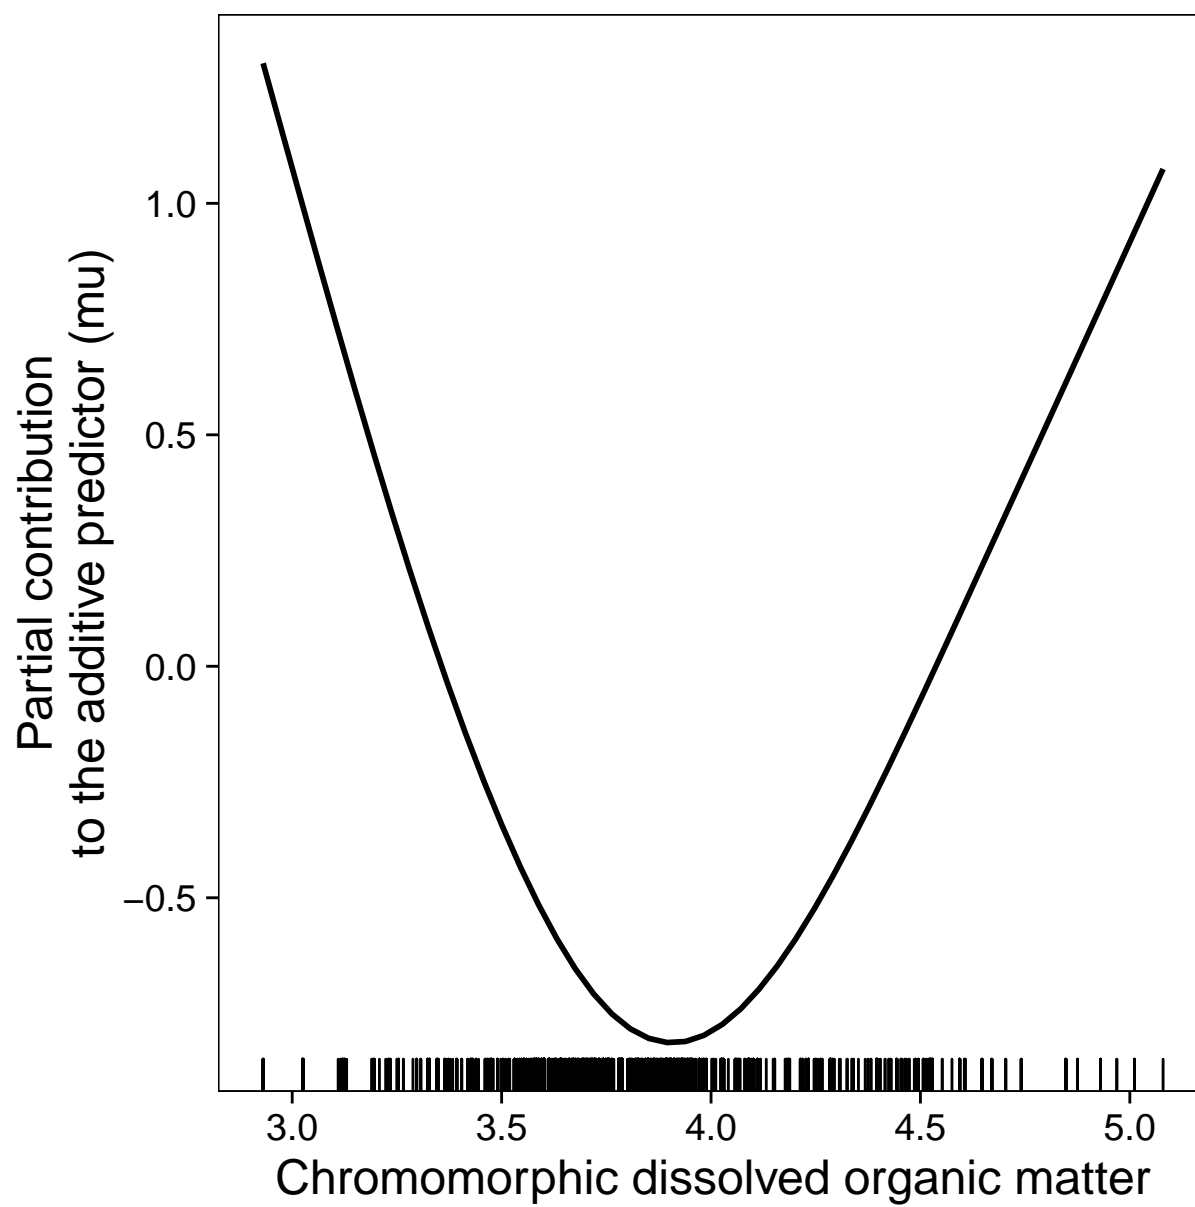

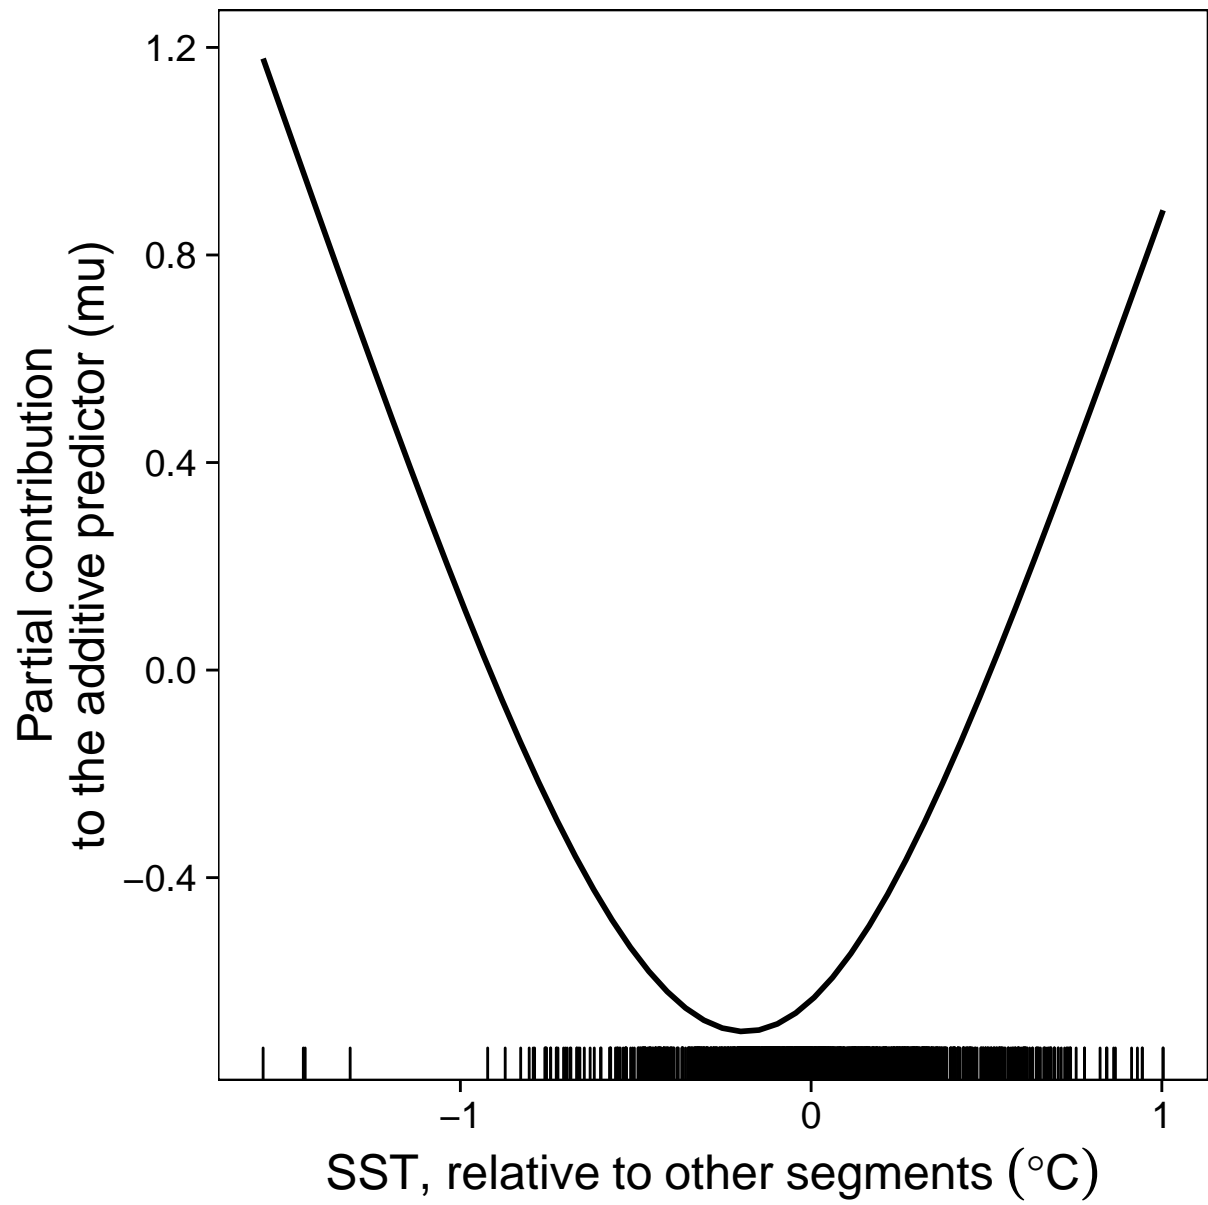

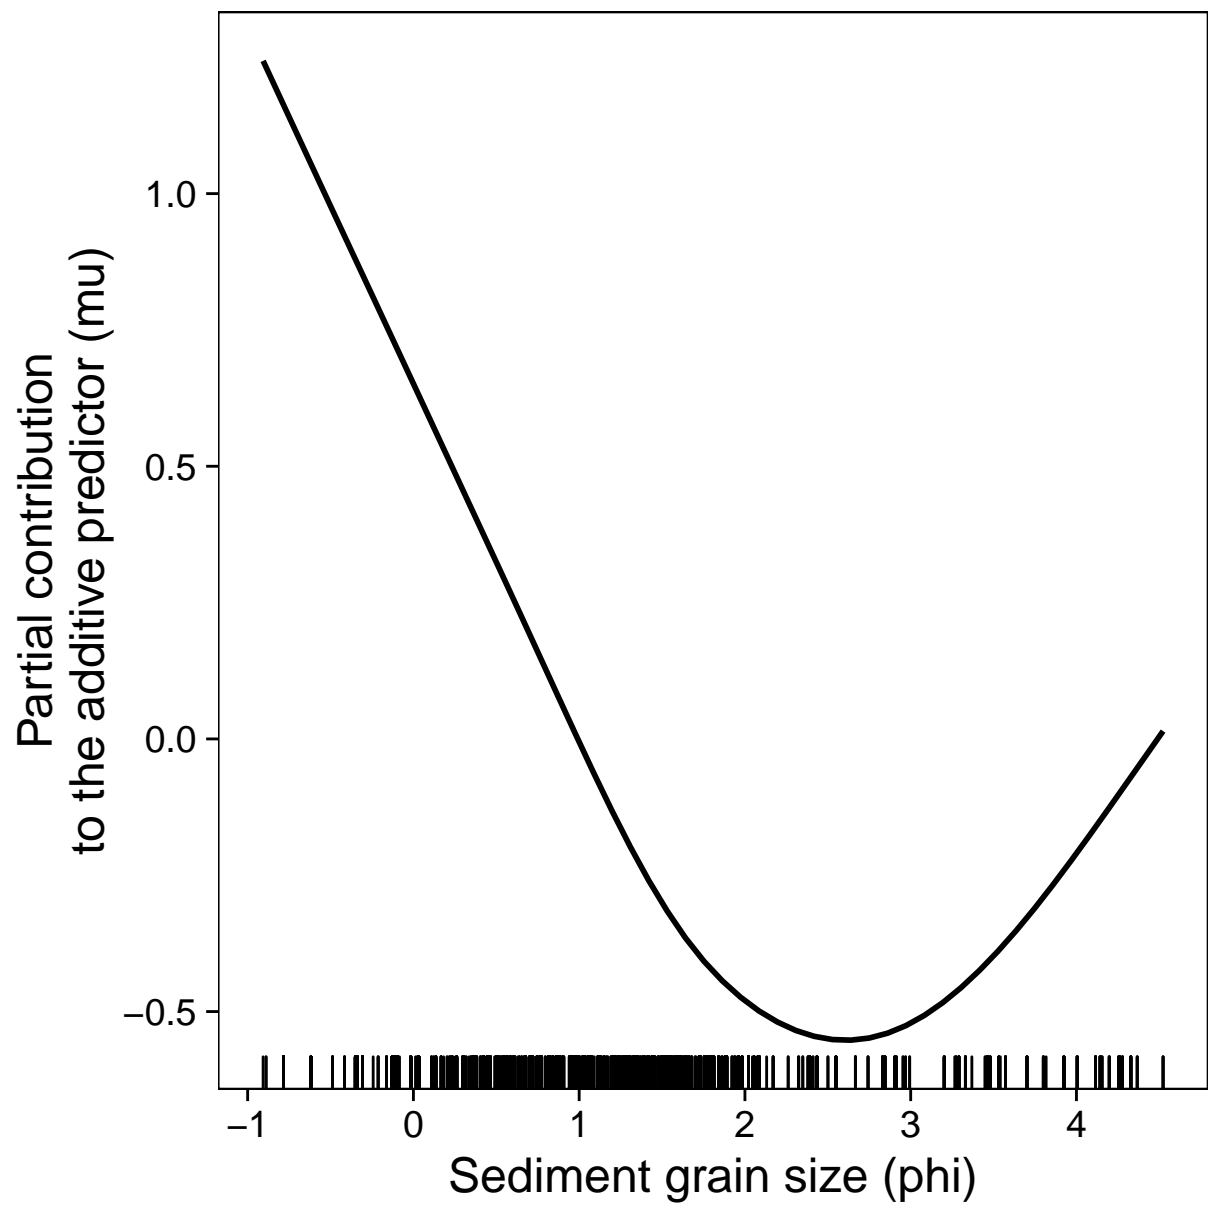

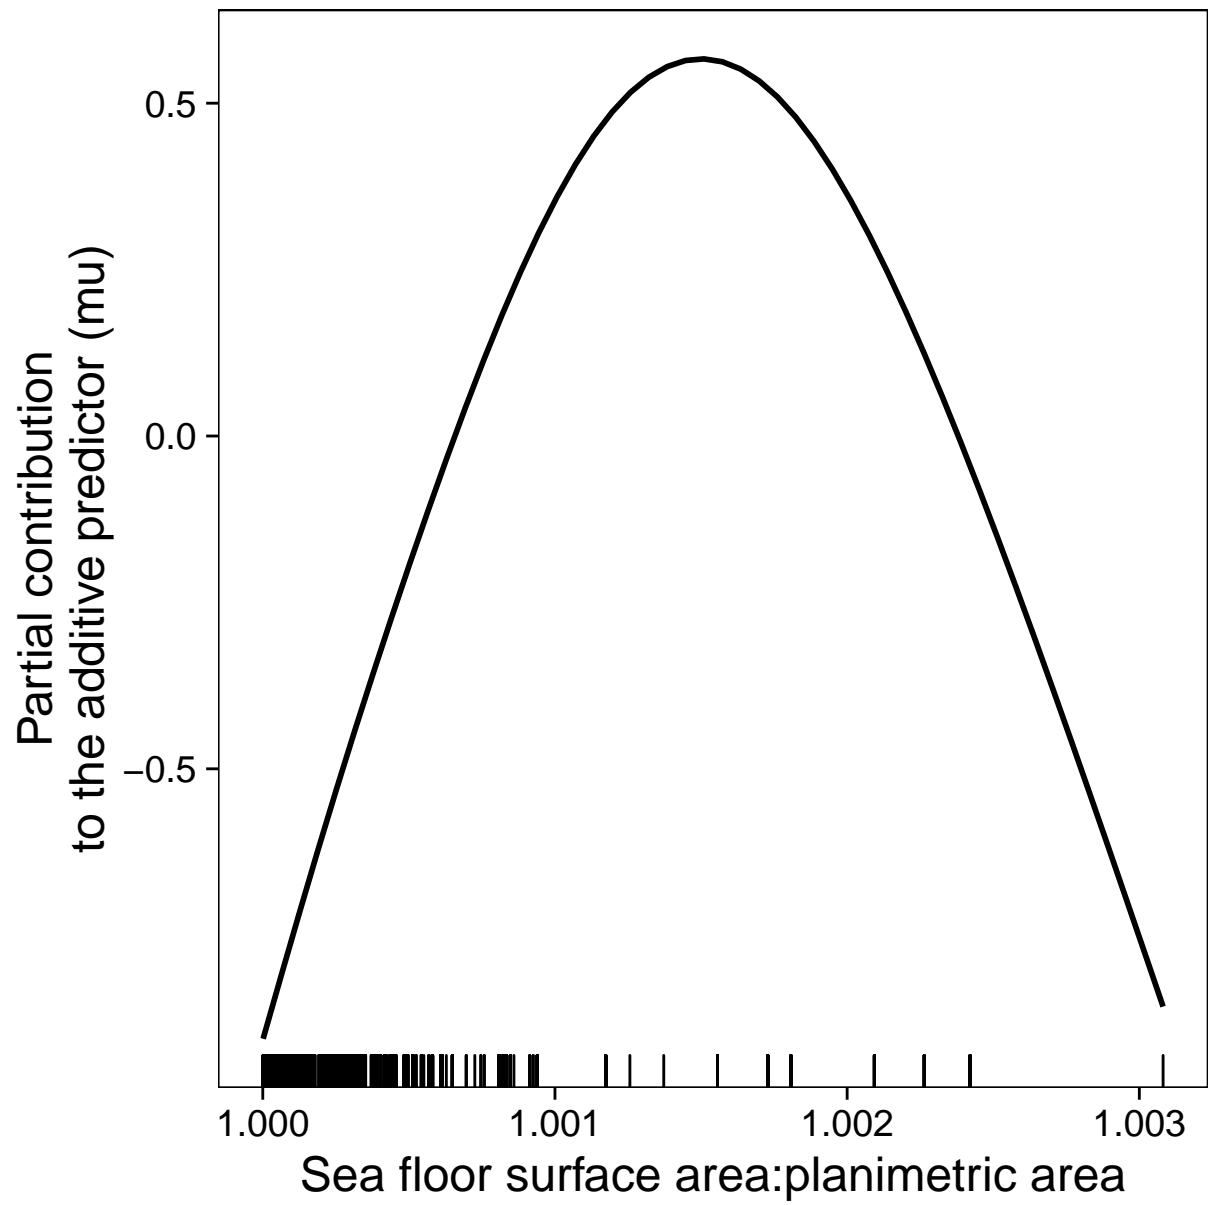

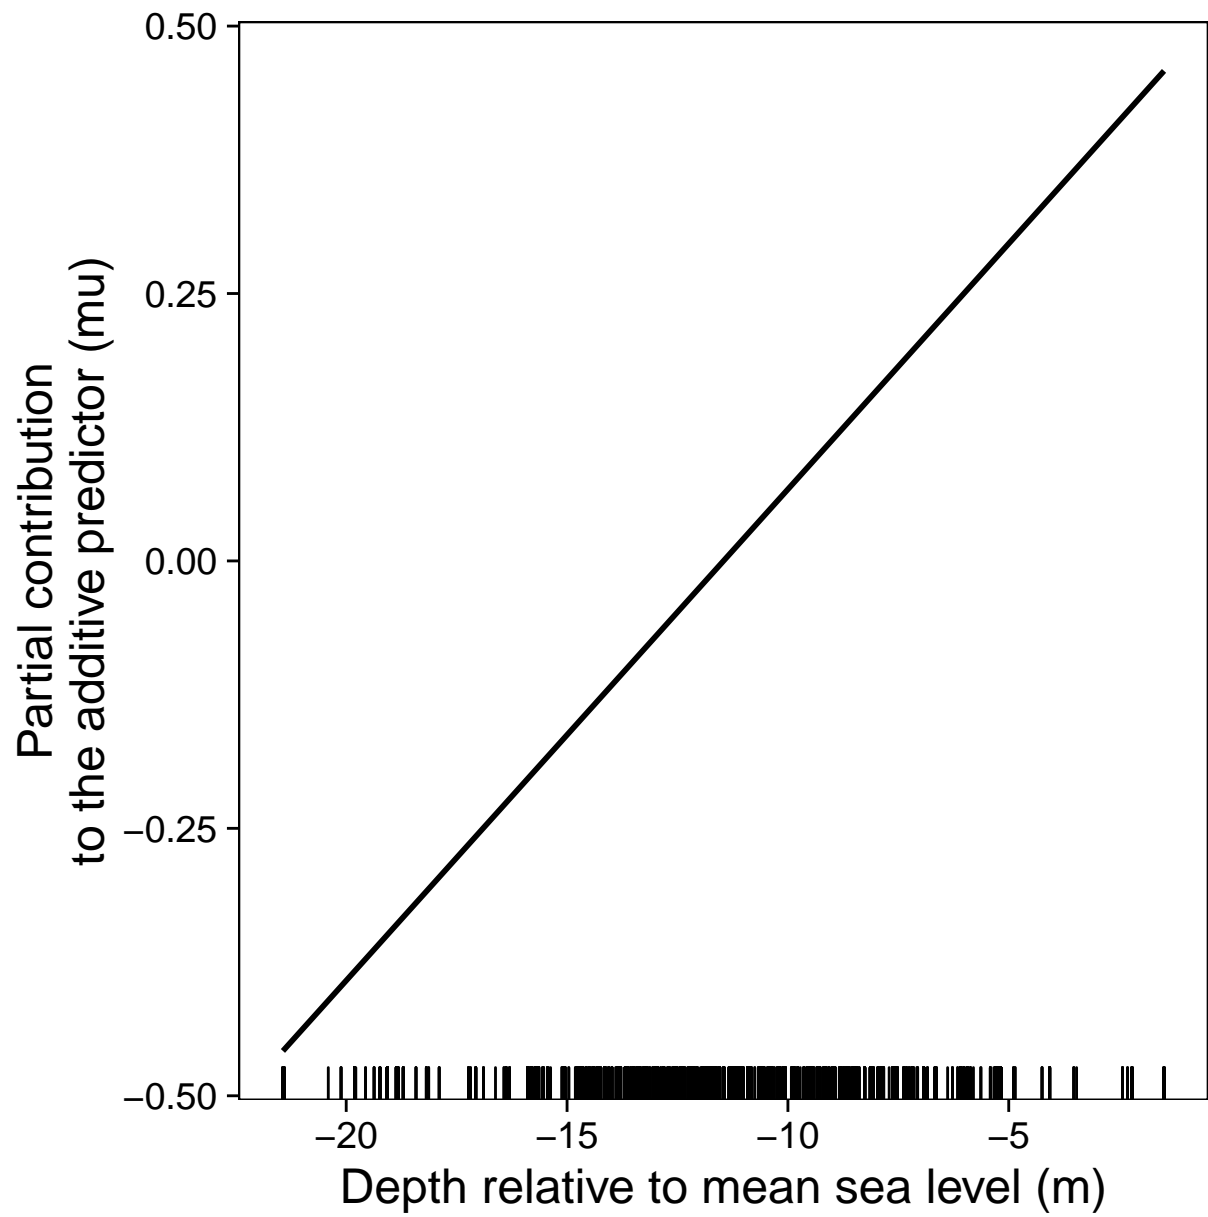

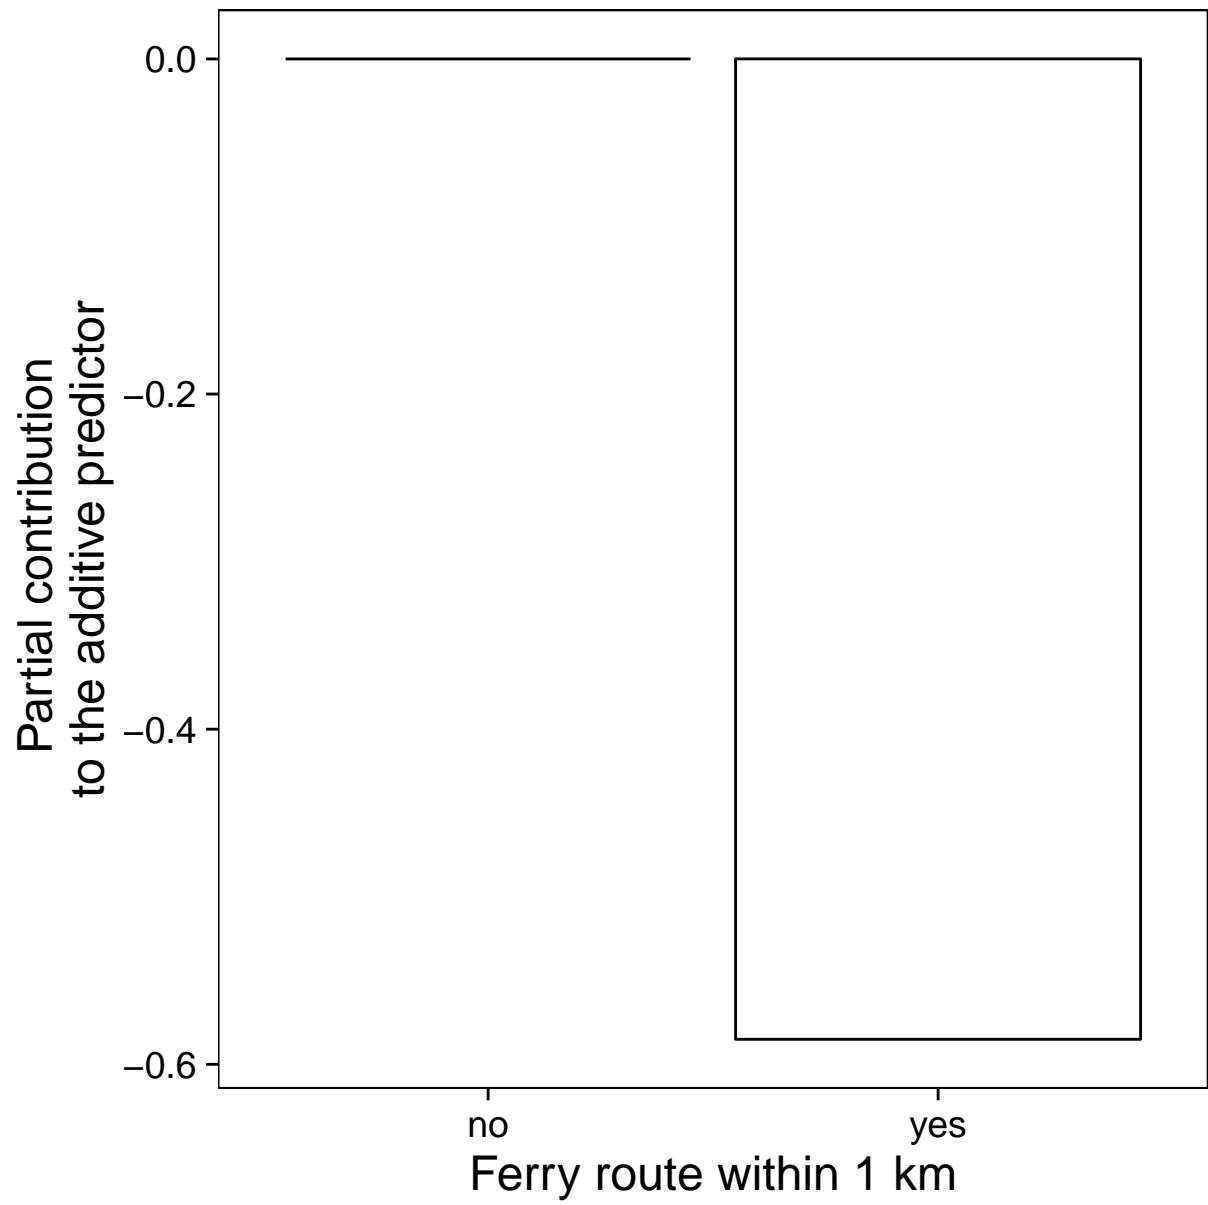

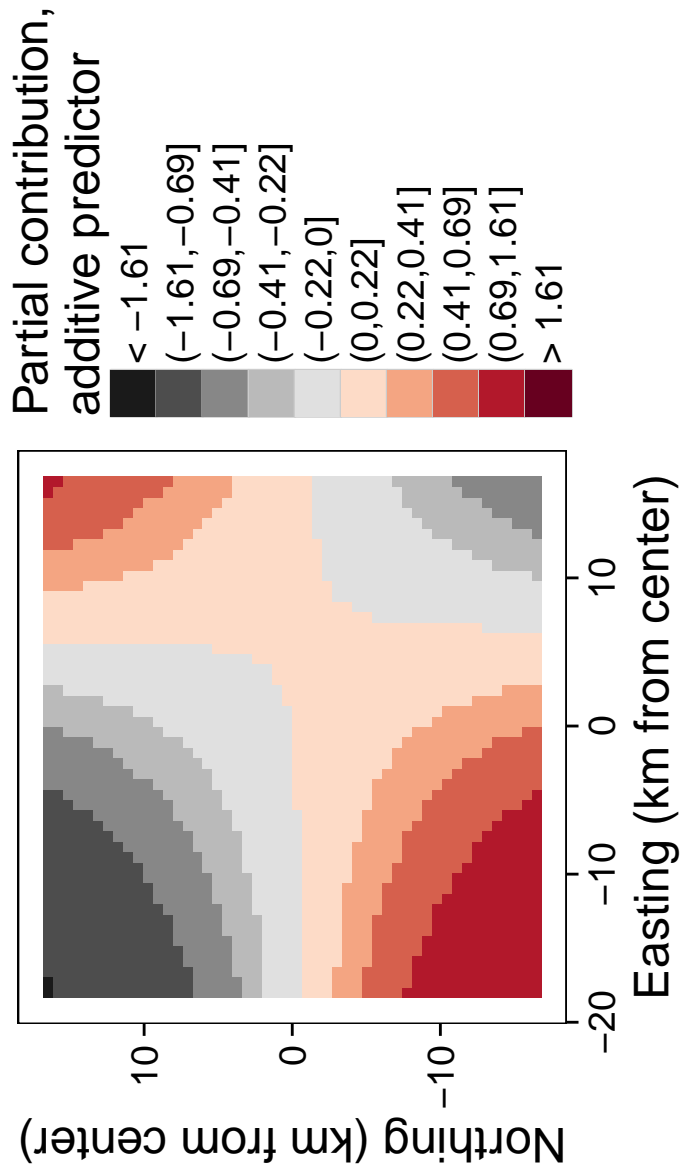

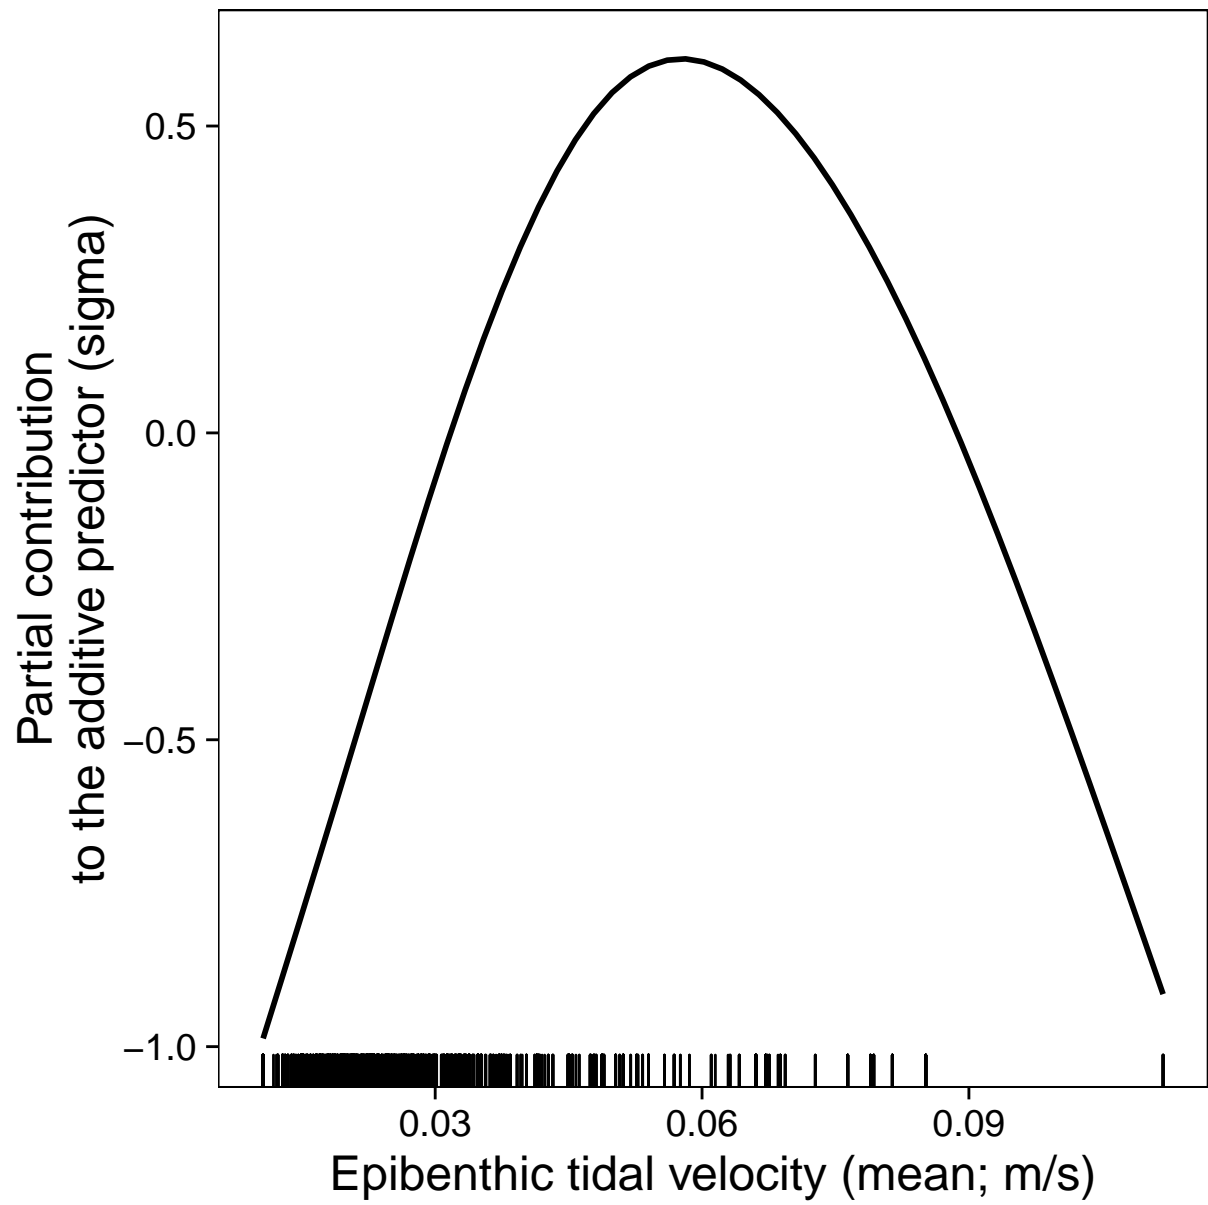

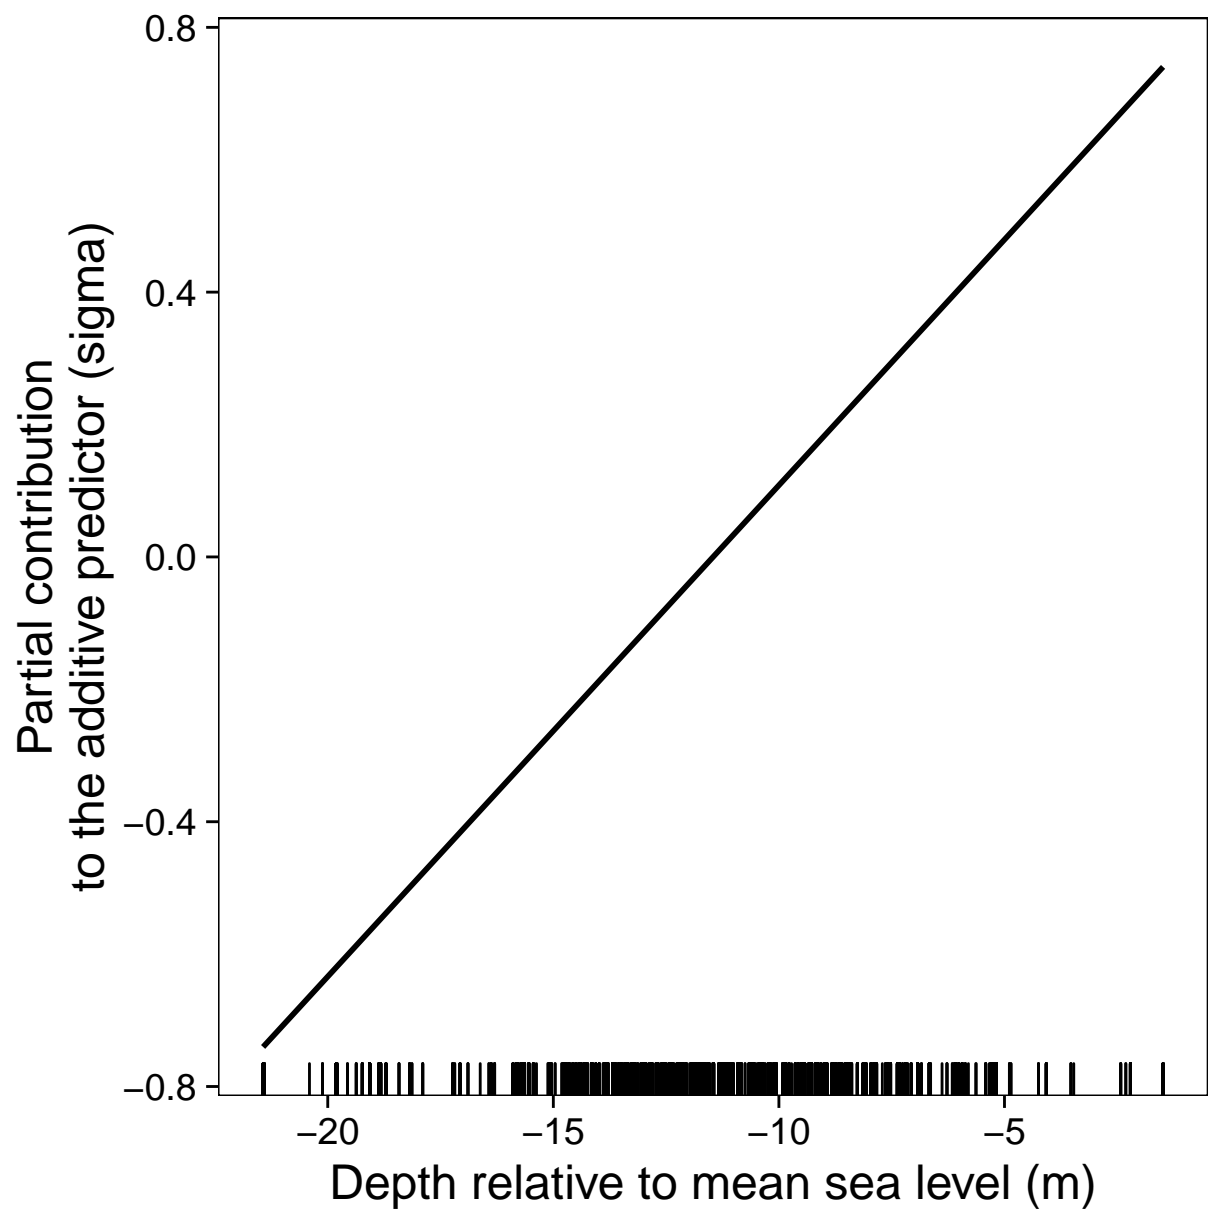

30

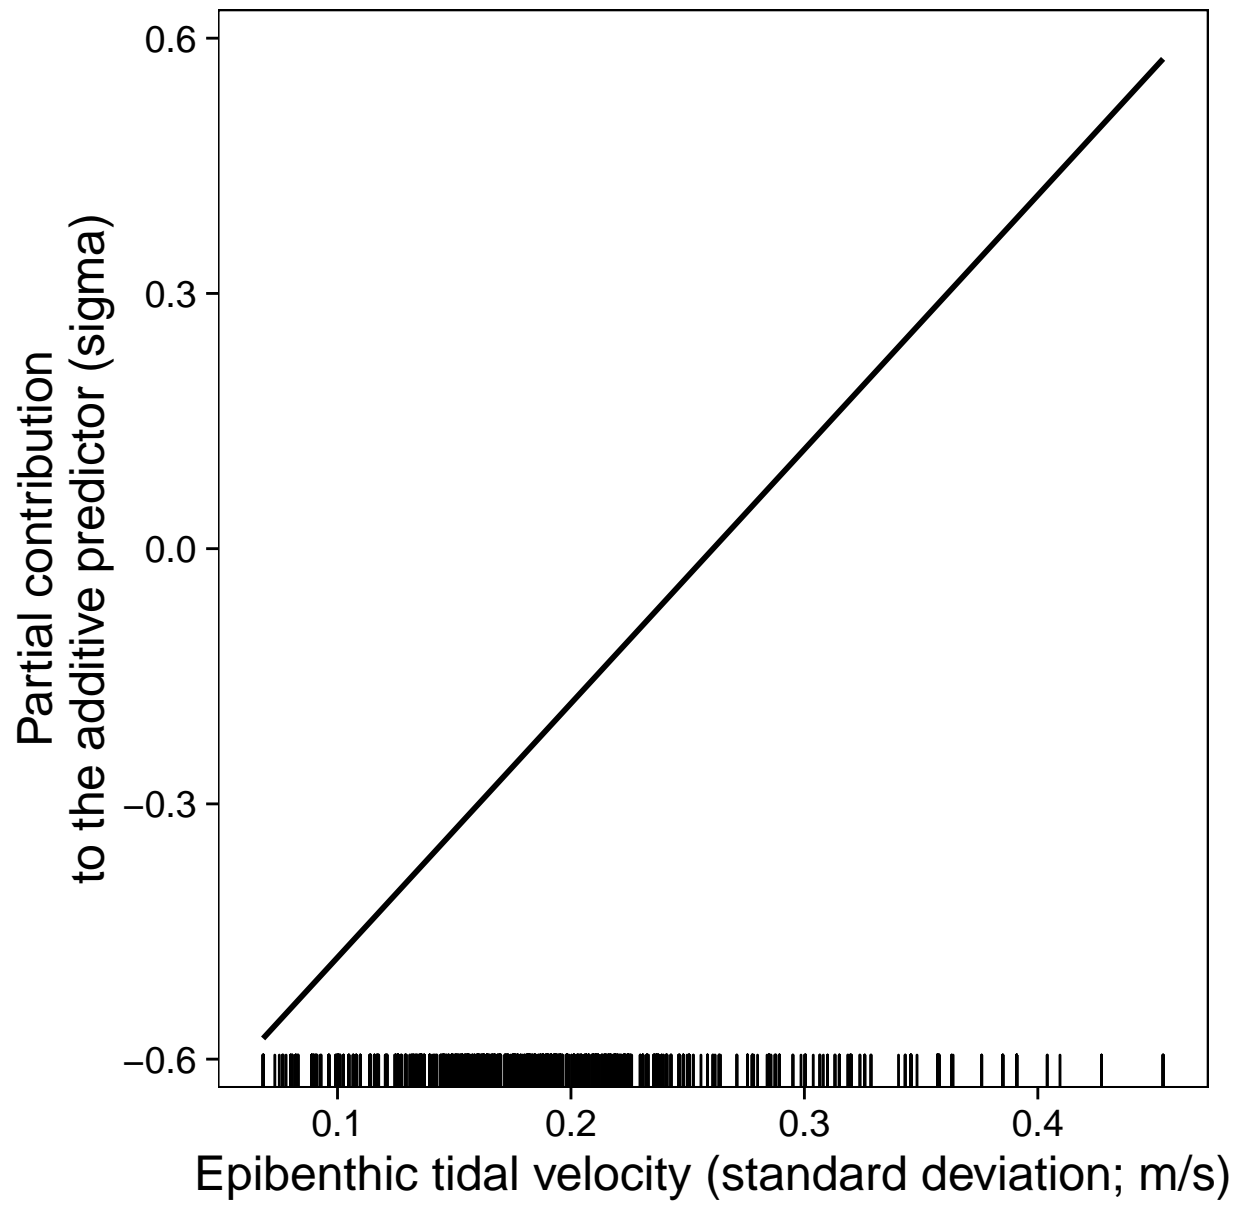

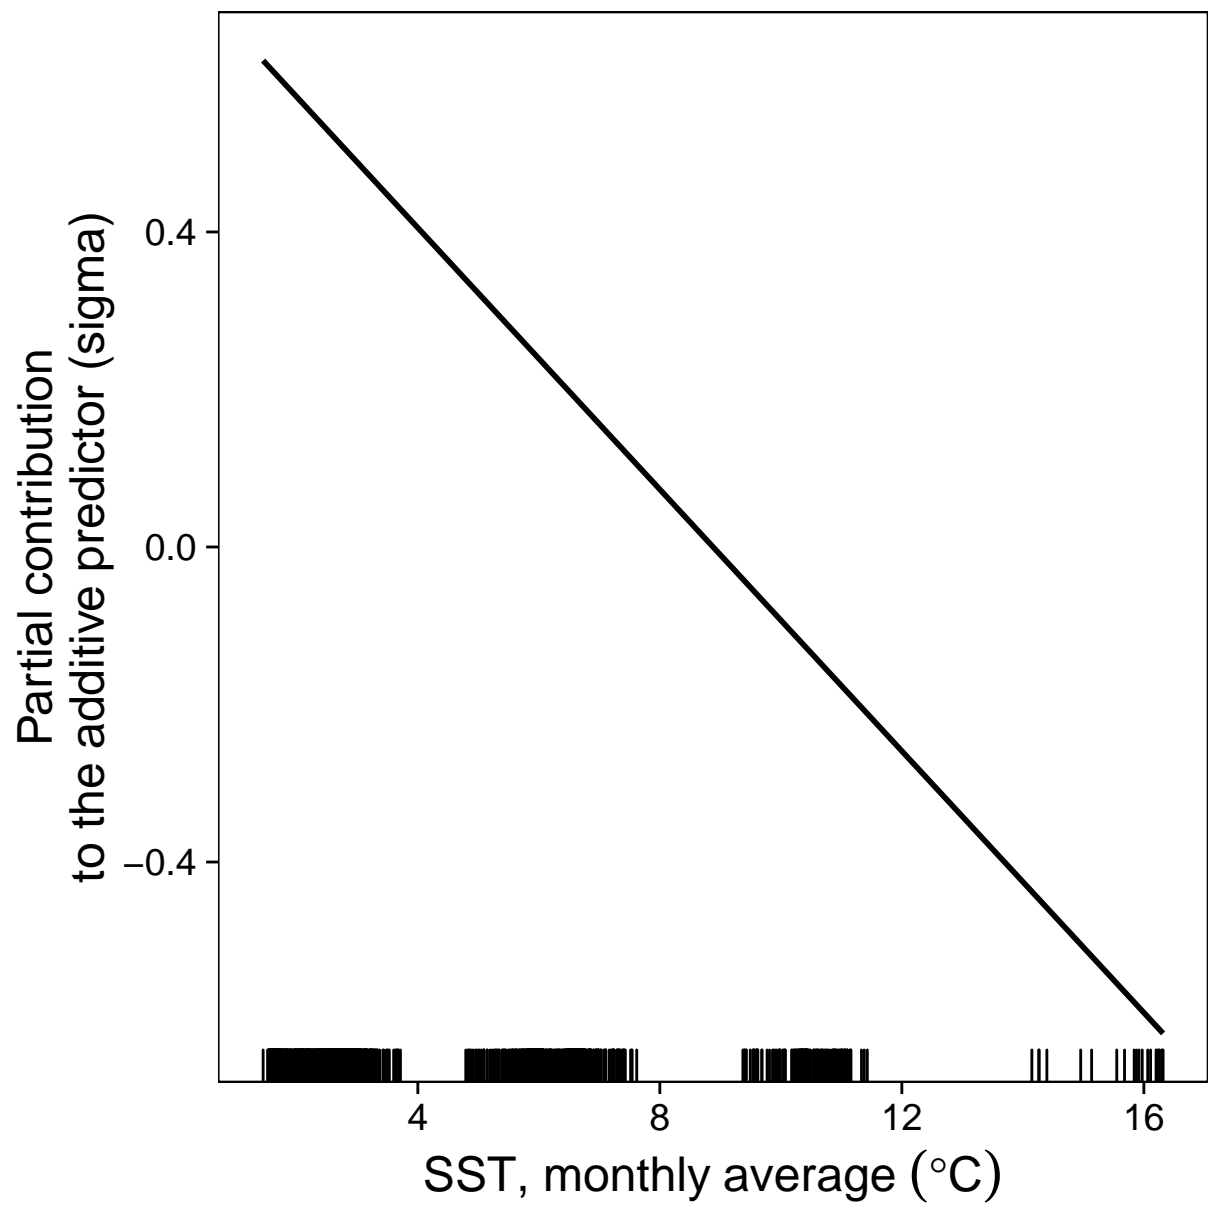

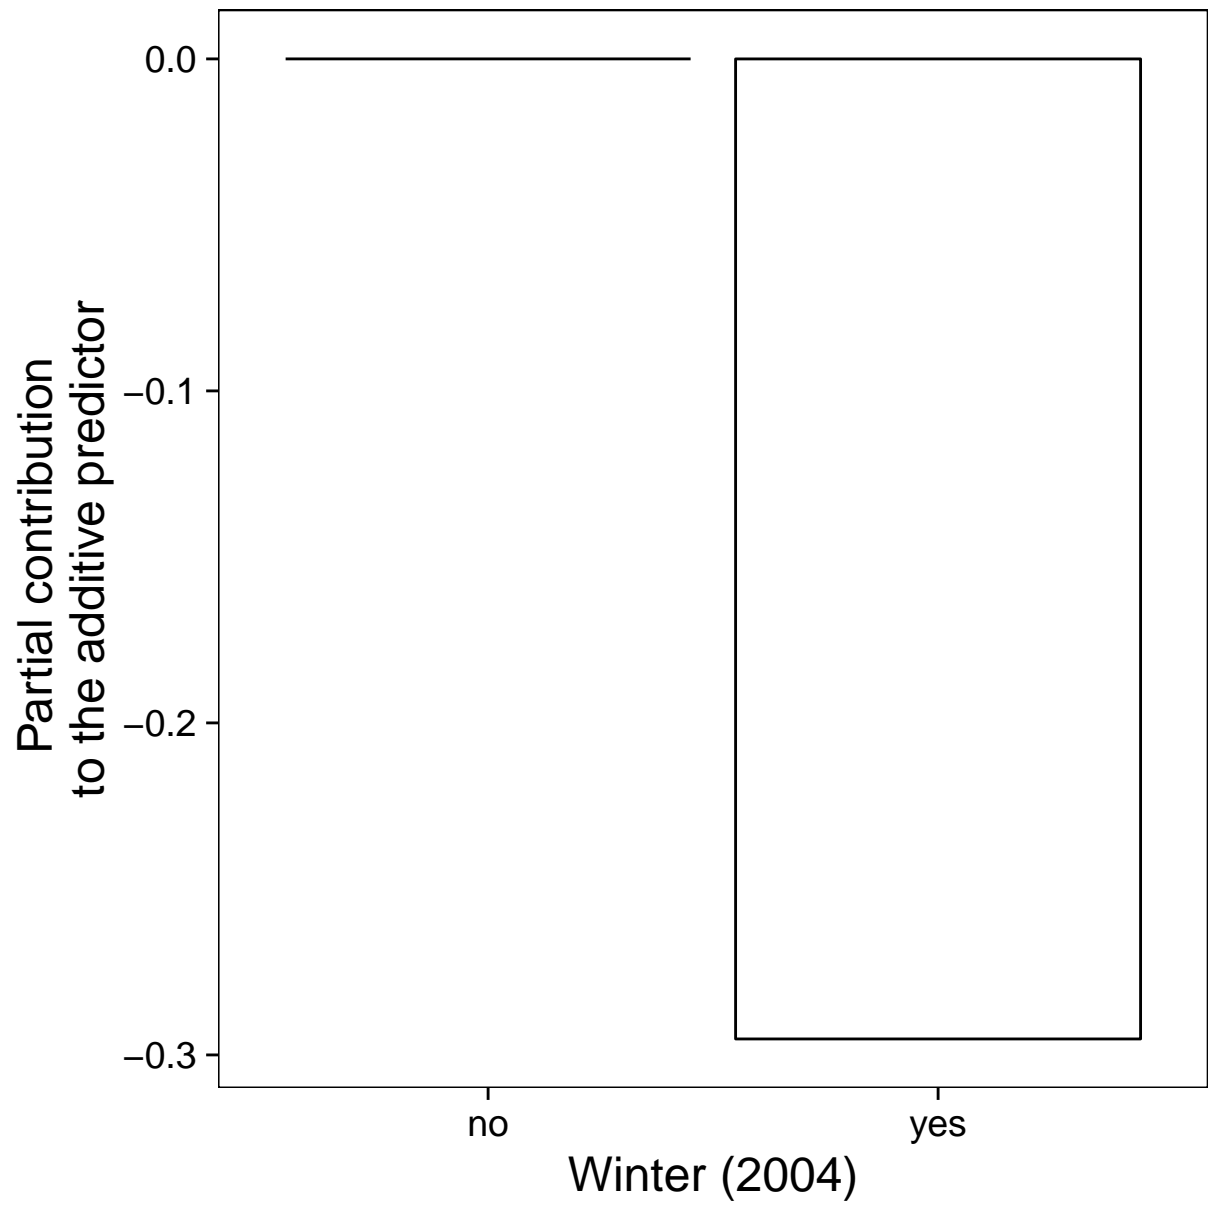

Supplement: Supplementary file 6 [file Appendix_S5.pdf]
