# Supplementary material for: Spatiotemporal modelling of sea duck abundance: implications for marine spatial planning
Source: arXiv:1705.00644 source file (2017-05-01)
Supplement: Supplementary file 8 [file Appendix_S9.pdf]

## **Appendix S9. Seasonal animation of predicted scoter occupancy and abundance**

To provide an example of the seasonal dynamics that can characterize sea duck occupancy and abundance in Nantucket Sound, we animate predicted scoter occupancy (Figure S9.1) and overall abundance (Figure S9.2; scoter per 1.5 km x ca. 180 m) for every week between 1 November 2005 and 31 March 2006.

**Figure S9.1**

**Figure S9.2**
